# Supplementary material for: Accelerated Discovery of Topological Conductors for Nanoscale Interconnects
Source: arXiv:2509.15135 source file (2025-09-18)

Compound: AgN<sub>3</sub>  
Materials Project ID: 571297

Lattice (conventional cell):

| Parameter        | Value   | Unit |
|------------------|---------|------|
| a                | 5.8273  | Å    |
| b                | 5.8273  | Å    |
| c                | 6.0257  | Å    |
| $\alpha$ (alpha) | 90.0000 | °    |
| $\beta$ (beta)   | 90.0000 | °    |
| $\gamma$ (gamma) | 90.0000 | °    |

Crystal structure (conventional cell):

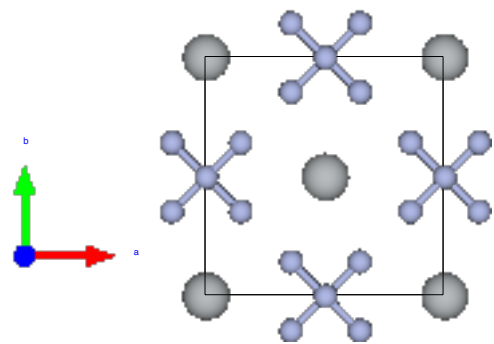

Nanowire Transmission:

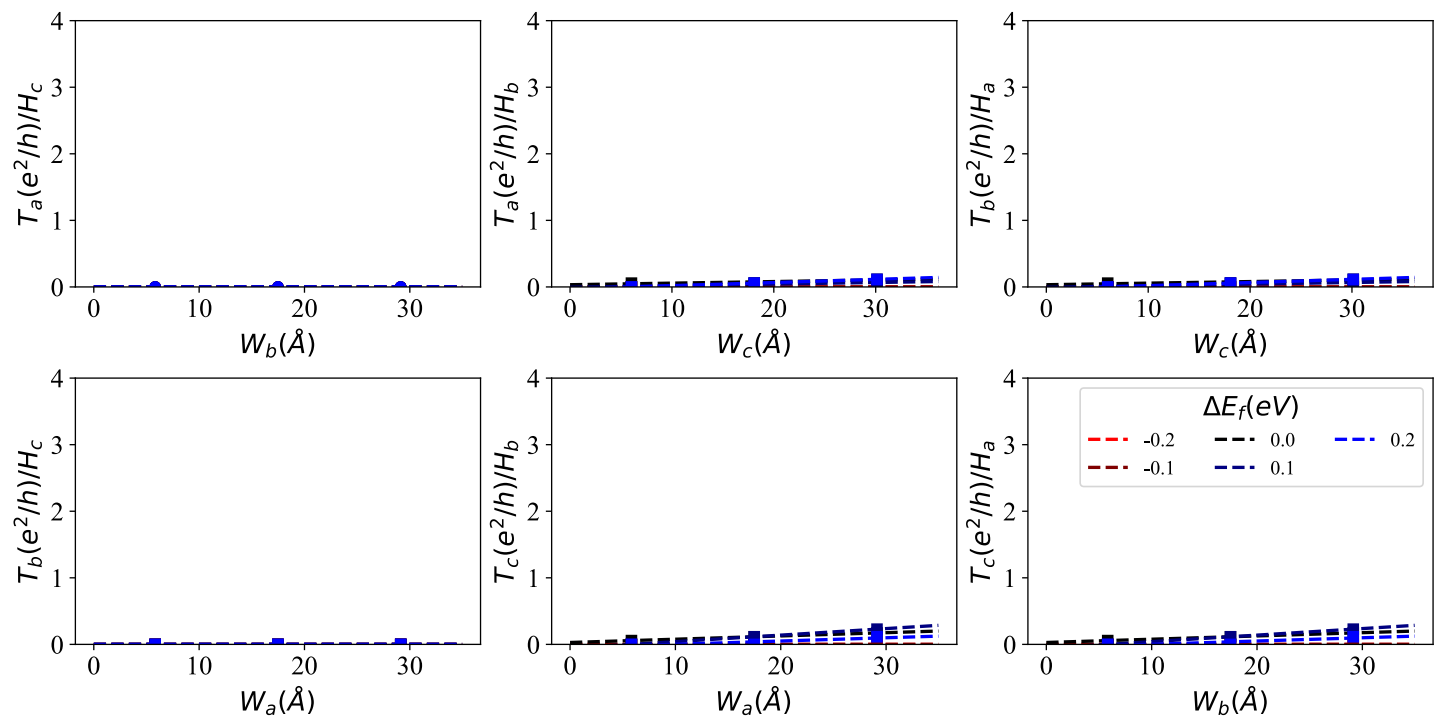

Compound: Ag<sub>2</sub>Se  
Materials Project ID: 568936

Lattice (conventional cell):

| Parameter        | Value   | Unit |
|------------------|---------|------|
| a                | 4.4975  | Å    |
| b                | 7.1133  | Å    |
| c                | 7.6707  | Å    |
| $\alpha$ (alpha) | 90.0000 | °    |
| $\beta$ (beta)   | 90.0000 | °    |
| $\gamma$ (gamma) | 90.0000 | °    |

Crystal structure (conventional cell):

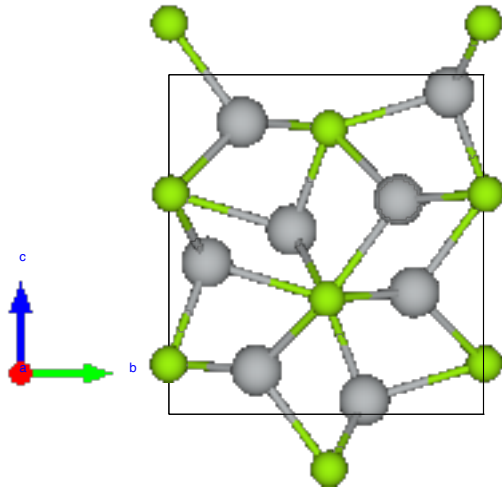

Nanowire Transmission:

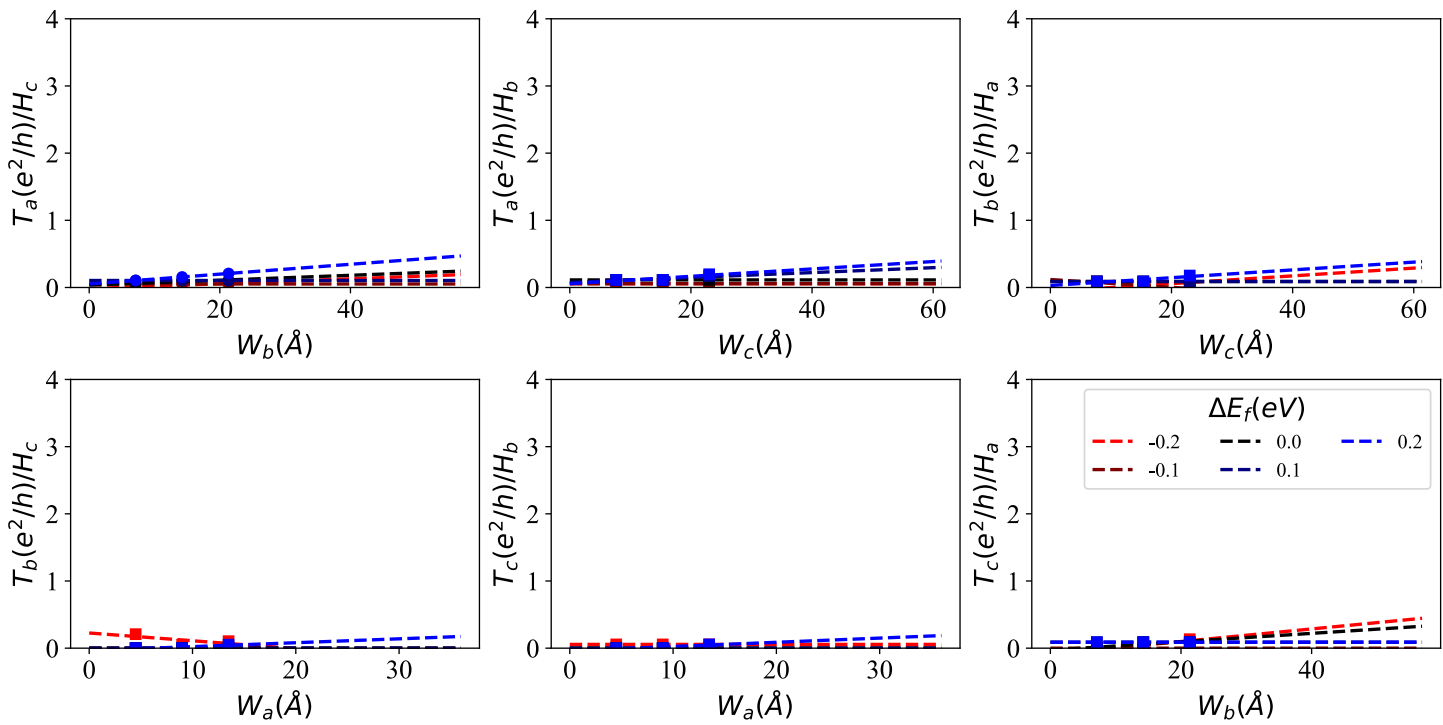

Compound: AlPd<sub>5</sub>I<sub>2</sub>  
Materials Project ID: 27393

Lattice (conventional cell):

| Parameter        | Value   | Unit |
|------------------|---------|------|
| a                | 4.0783  | Å    |
| b                | 4.0783  | Å    |
| c                | 20.2662 | Å    |
| $\alpha$ (alpha) | 90.0000 | °    |
| $\beta$ (beta)   | 90.0000 | °    |
| $\gamma$ (gamma) | 90.0000 | °    |

Crystal structure (conventional cell):

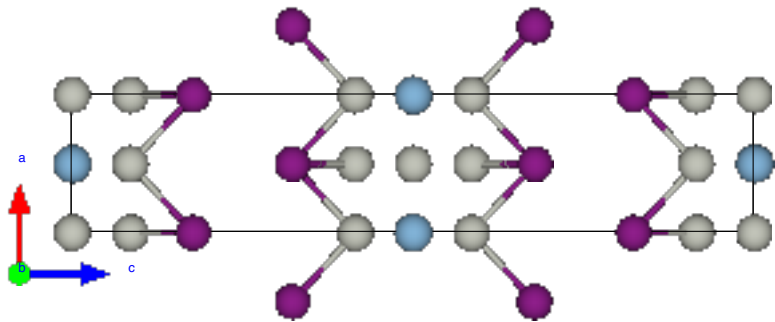

Nanowire Transmission:

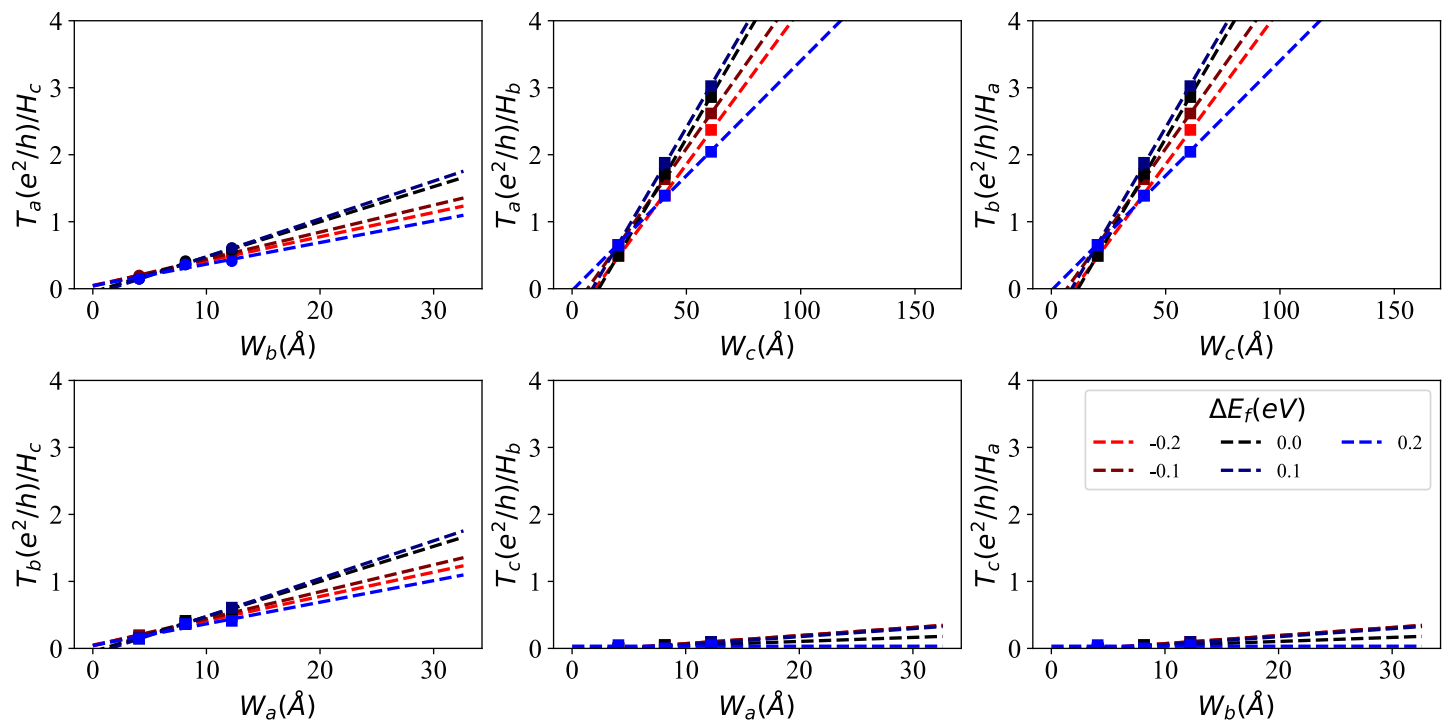

Compound: AlPt  
Materials Project ID: 10904

Lattice (conventional cell):

| Parameter        | Value   | Unit |
|------------------|---------|------|
| a                | 4.9174  | Å    |
| b                | 4.9174  | Å    |
| c                | 4.9174  | Å    |
| $\alpha$ (alpha) | 90.0000 | °    |
| $\beta$ (beta)   | 90.0000 | °    |
| $\gamma$ (gamma) | 90.0000 | °    |

Crystal structure (conventional cell):

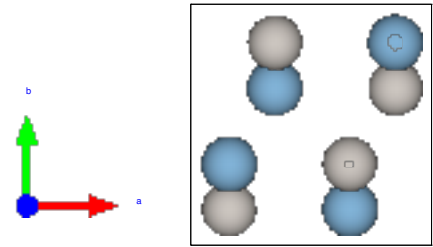

Nanowire Transmission:

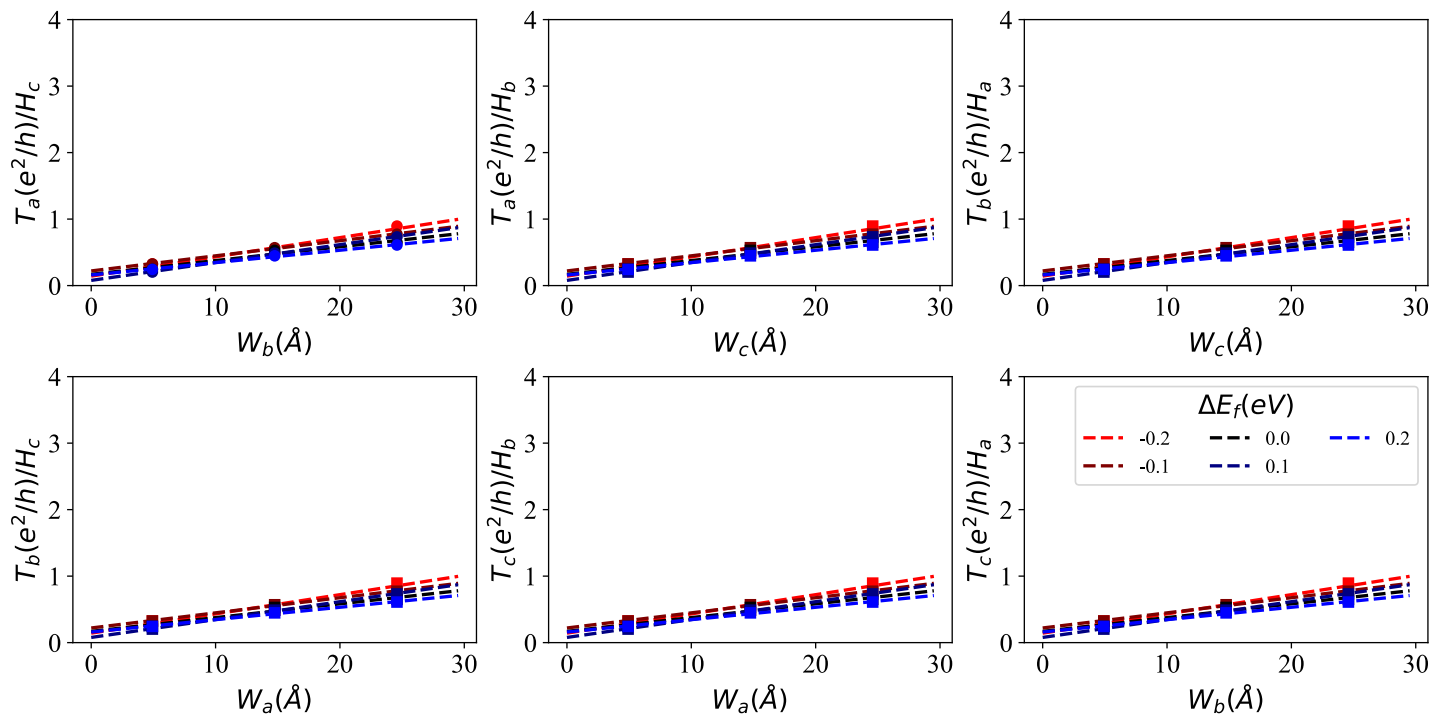



Compound: Au  
Materials Project ID: 81

Lattice (conventional cell):

| Parameter        | Value   | Unit |
|------------------|---------|------|
| a                | 4.1713  | Å    |
| b                | 4.1713  | Å    |
| c                | 4.1713  | Å    |
| $\alpha$ (alpha) | 90.0000 | °    |
| $\beta$ (beta)   | 90.0000 | °    |
| $\gamma$ (gamma) | 90.0000 | °    |

Crystal structure (conventional cell):

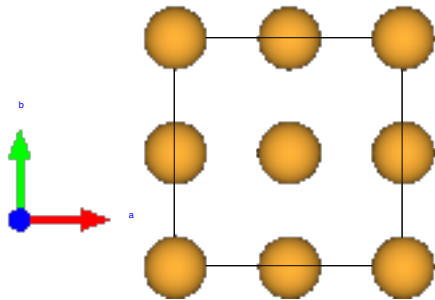

Nanowire Transmission:

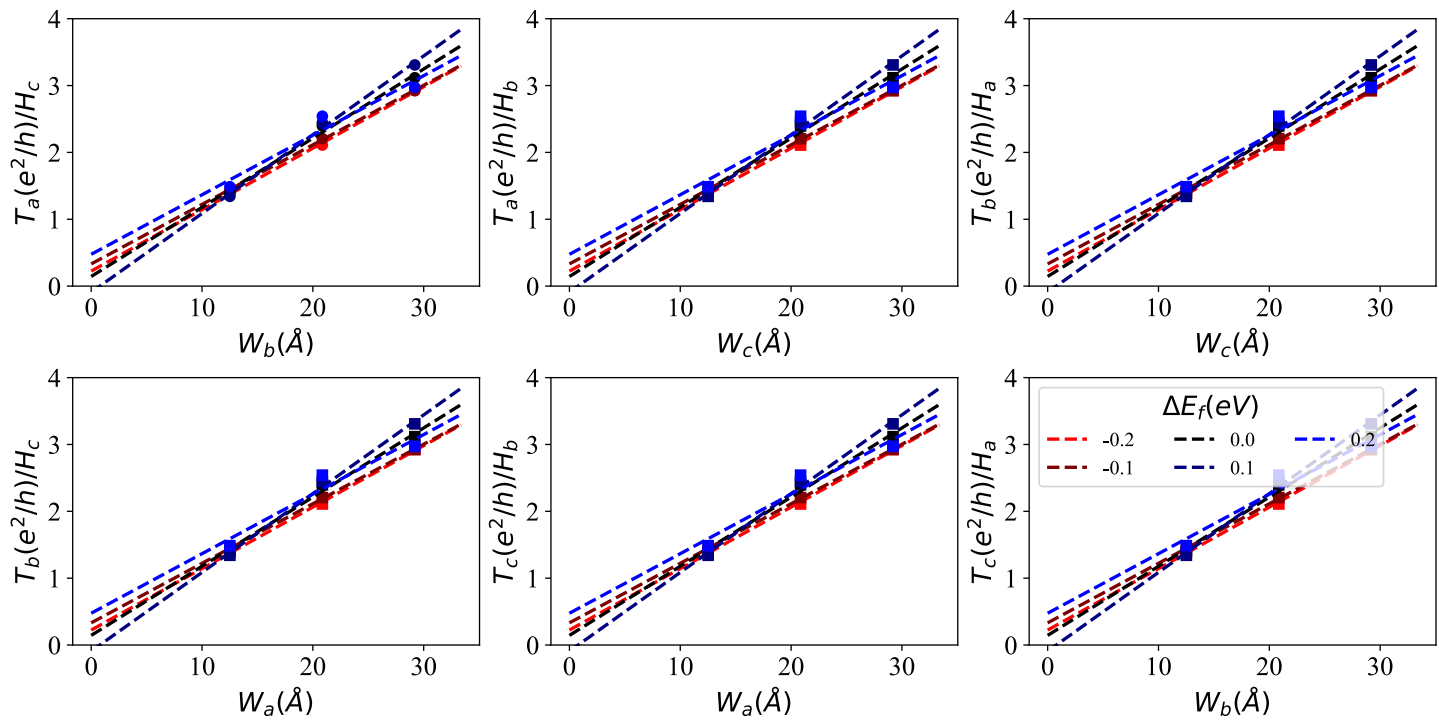

Compound: BaAl<sub>4</sub>  
Materials Project ID: 1903

Lattice (conventional cell):

| Parameter        | Value   | Unit |
|------------------|---------|------|
| a                | 4.5765  | Å    |
| b                | 4.5765  | Å    |
| c                | 11.3531 | Å    |
| $\alpha$ (alpha) | 90.0000 | °    |
| $\beta$ (beta)   | 90.0000 | °    |
| $\gamma$ (gamma) | 90.0000 | °    |

Crystal structure (conventional cell):

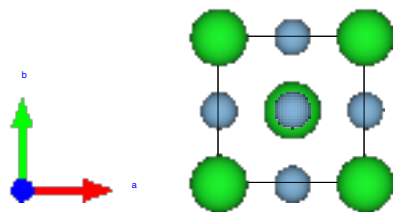

Nanowire Transmission:

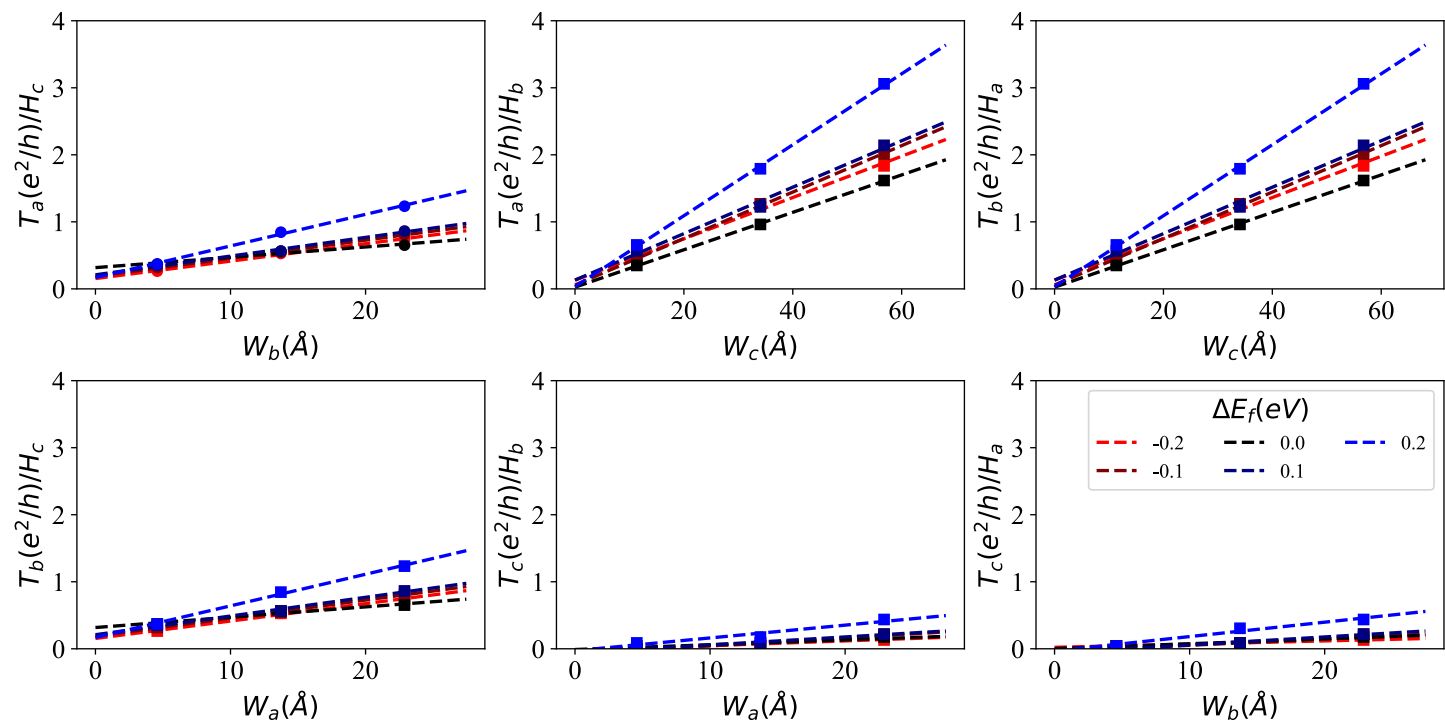

Compound: BaB<sub>6</sub>  
Materials Project ID: 954

Lattice (conventional cell):

| Parameter        | Value   | Unit |
|------------------|---------|------|
| a                | 4.2801  | Å    |
| b                | 4.2801  | Å    |
| c                | 4.2801  | Å    |
| $\alpha$ (alpha) | 90.0000 | °    |
| $\beta$ (beta)   | 90.0000 | °    |
| $\gamma$ (gamma) | 90.0000 | °    |

Crystal structure (conventional cell):

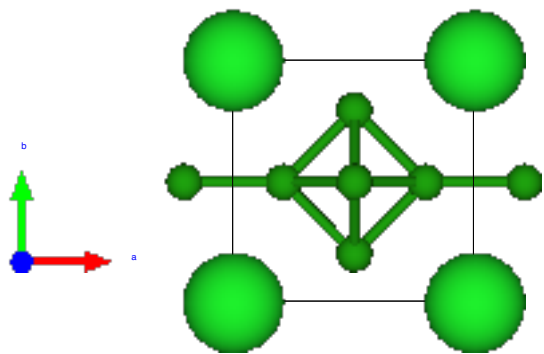

Nanowire Transmission:

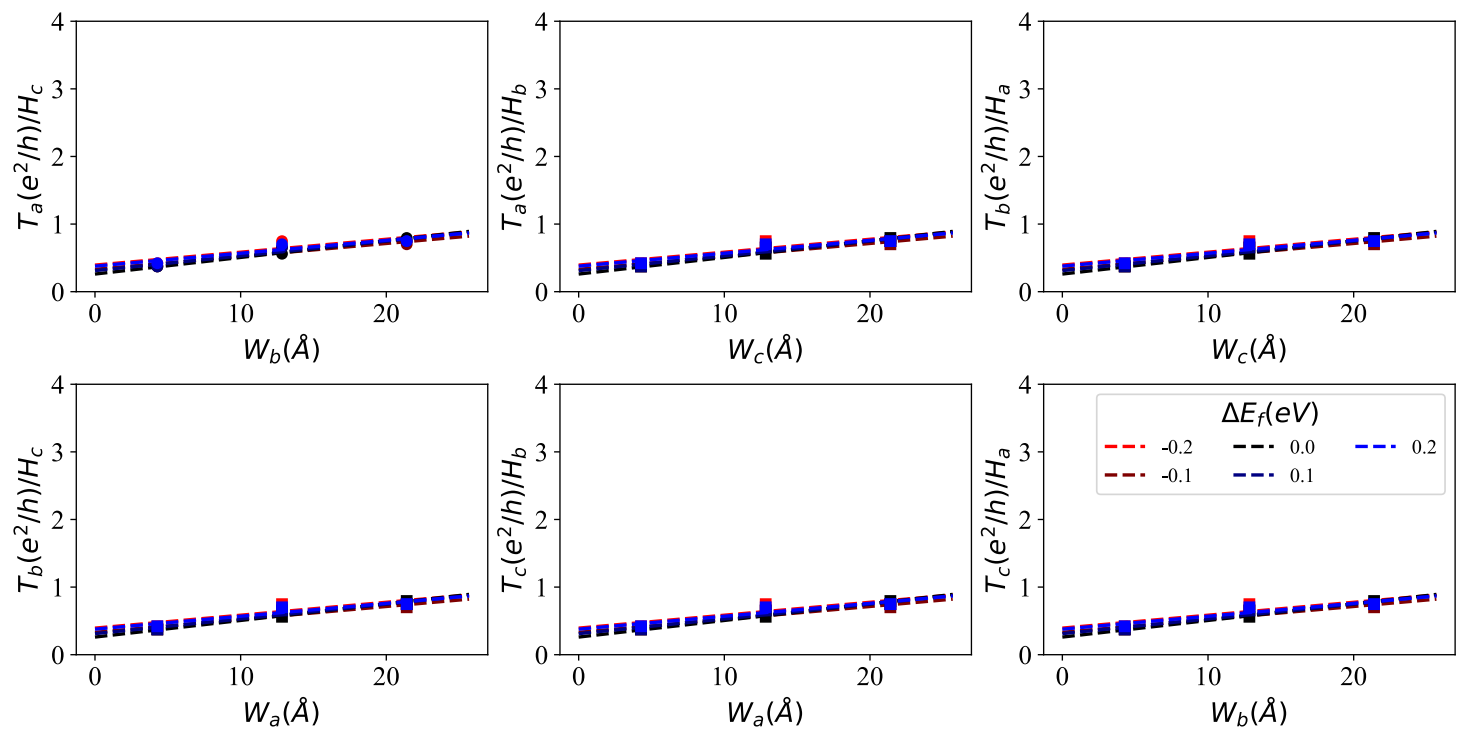

Compound: BaSi<sub>2</sub>  
Materials Project ID: 7655

Lattice (conventional cell):

| Parameter | Value    | Unit |
|-----------|----------|------|
| a         | 4.0928   | Å    |
| b         | 4.0928   | Å    |
| c         | 5.3629   | Å    |
| α (alpha) | 90.0000  | °    |
| β (beta)  | 90.0000  | °    |
| γ (gamma) | 120.0000 | °    |

Crystal structure (conventional cell):

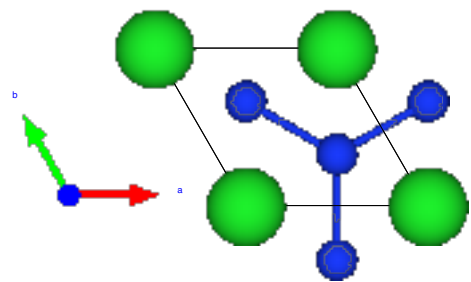

Nanowire Transmission:

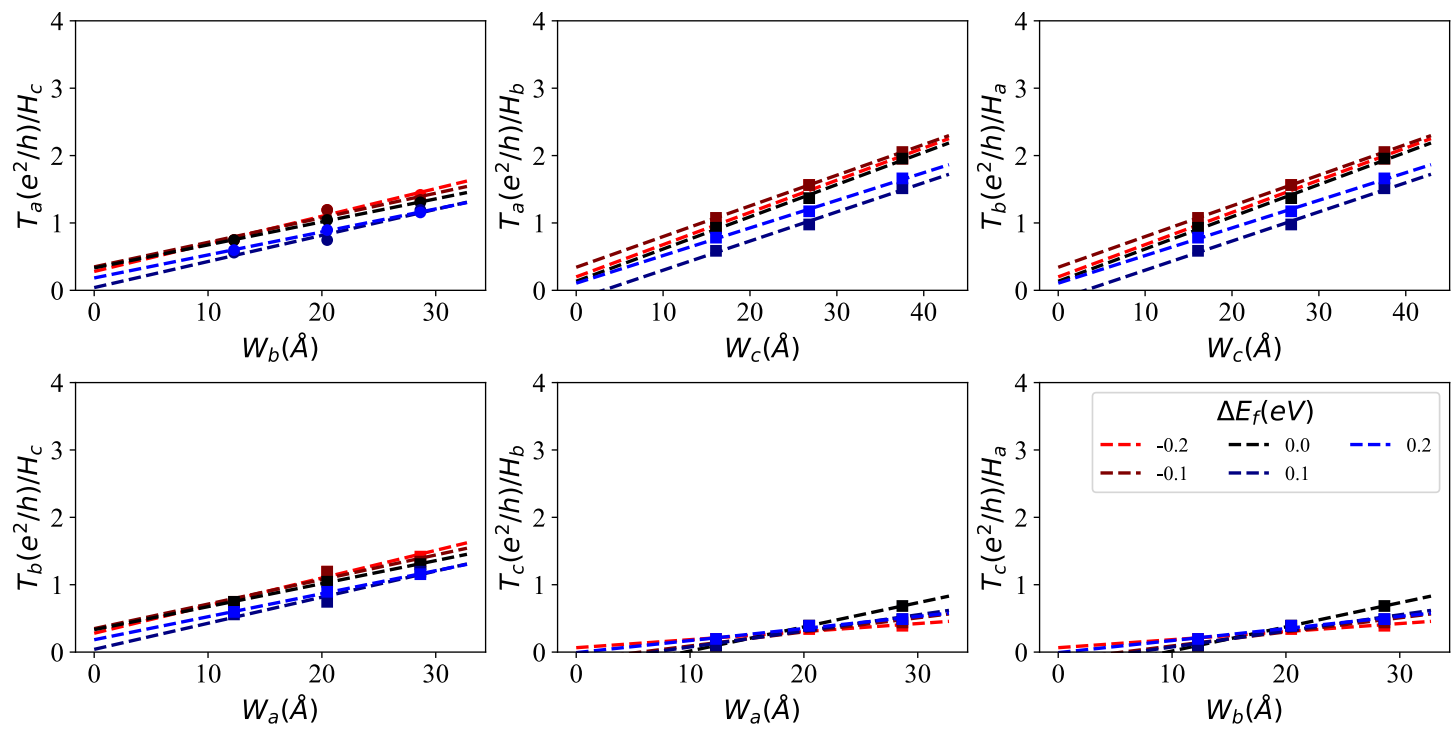

Compound: BaSn<sub>2</sub>  
Materials Project ID: 567510

Lattice (conventional cell):

| Parameter        | Value    | Unit |
|------------------|----------|------|
| a                | 4.7650   | Å    |
| b                | 4.7650   | Å    |
| c                | 5.6084   | Å    |
| $\alpha$ (alpha) | 90.0000  | °    |
| $\beta$ (beta)   | 90.0000  | °    |
| $\gamma$ (gamma) | 120.0000 | °    |

Crystal structure (conventional cell):

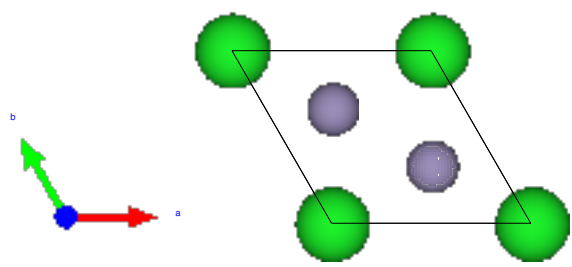

Nanowire Transmission:

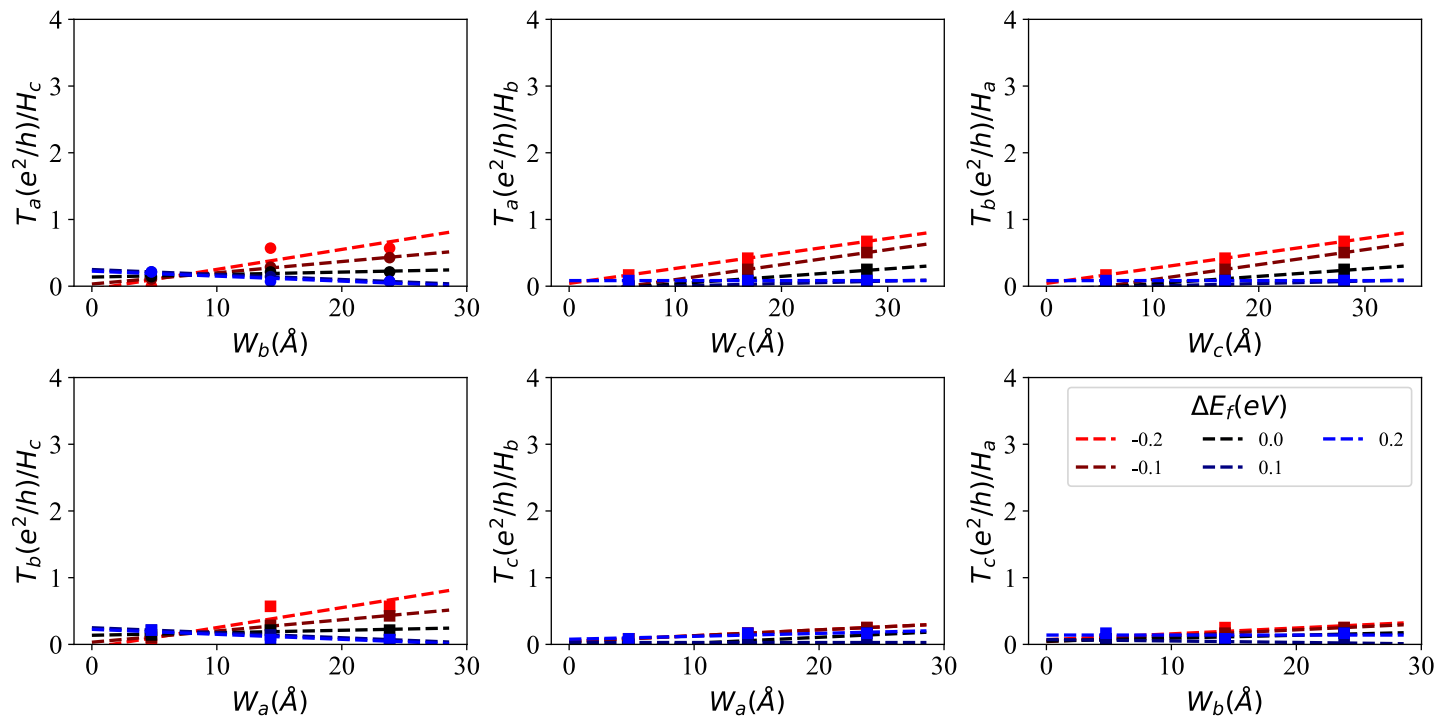

Compound: Be  
Materials Project ID: 87

Lattice (conventional cell):

| Parameter        | Value    | Unit |
|------------------|----------|------|
| a                | 2.2598   | Å    |
| b                | 2.2598   | Å    |
| c                | 3.5699   | Å    |
| $\alpha$ (alpha) | 90.0000  | °    |
| $\beta$ (beta)   | 90.0000  | °    |
| $\gamma$ (gamma) | 120.0000 | °    |

Crystal structure (conventional cell):

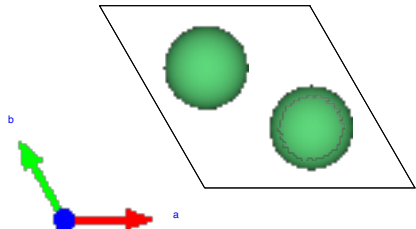

Nanowire Transmission:

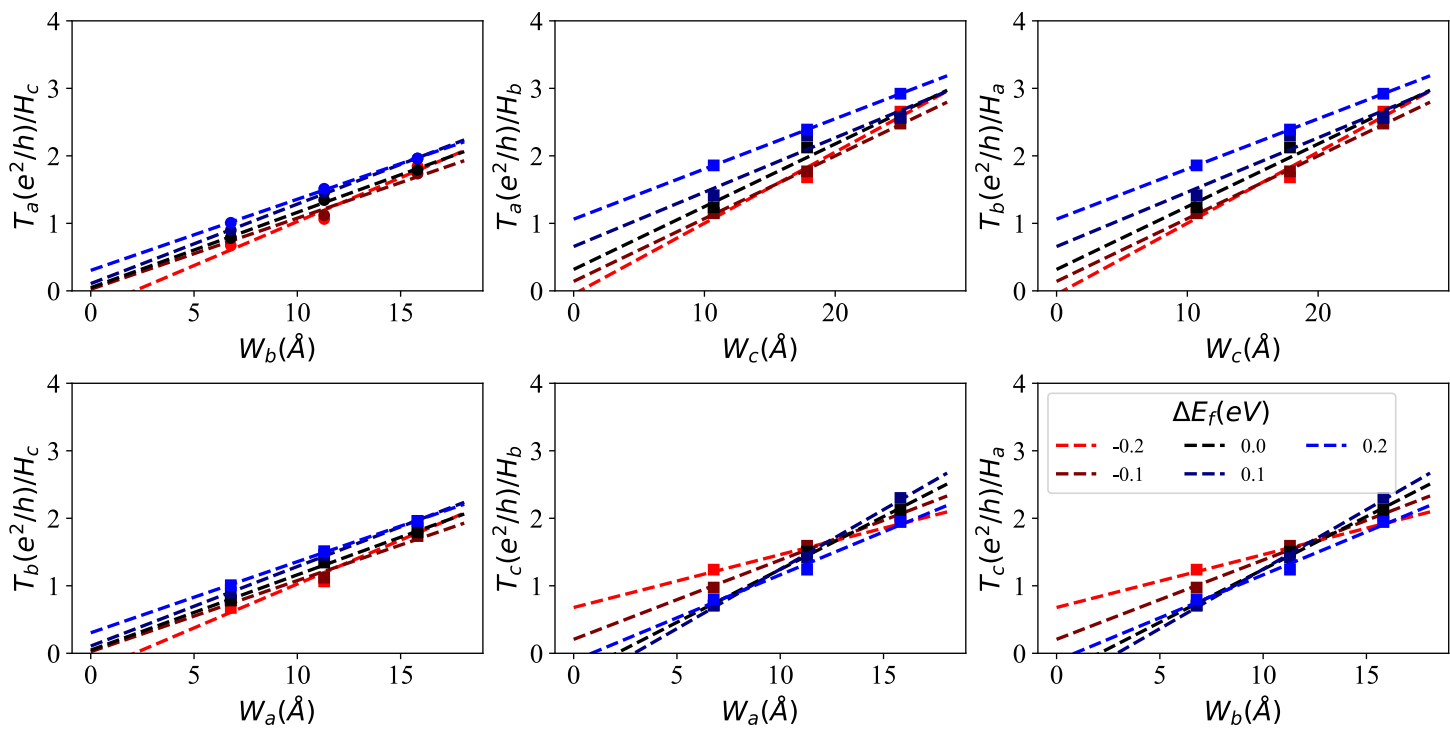

Compound: Bi  
Materials Project ID: 23152

Lattice (conventional cell):

| Parameter        | Value    | Unit |
|------------------|----------|------|
| a                | 4.6096   | Å    |
| b                | 4.6096   | Å    |
| c                | 11.9755  | Å    |
| $\alpha$ (alpha) | 90.0000  | °    |
| $\beta$ (beta)   | 90.0000  | °    |
| $\gamma$ (gamma) | 120.0000 | °    |

Crystal structure (conventional cell):

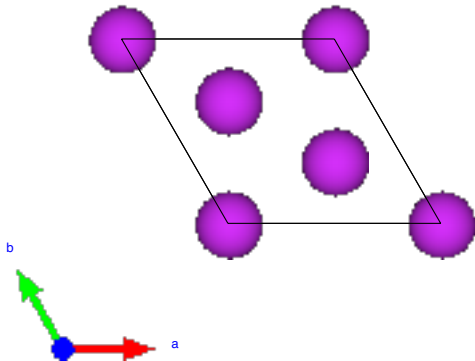

Nanowire Transmission:

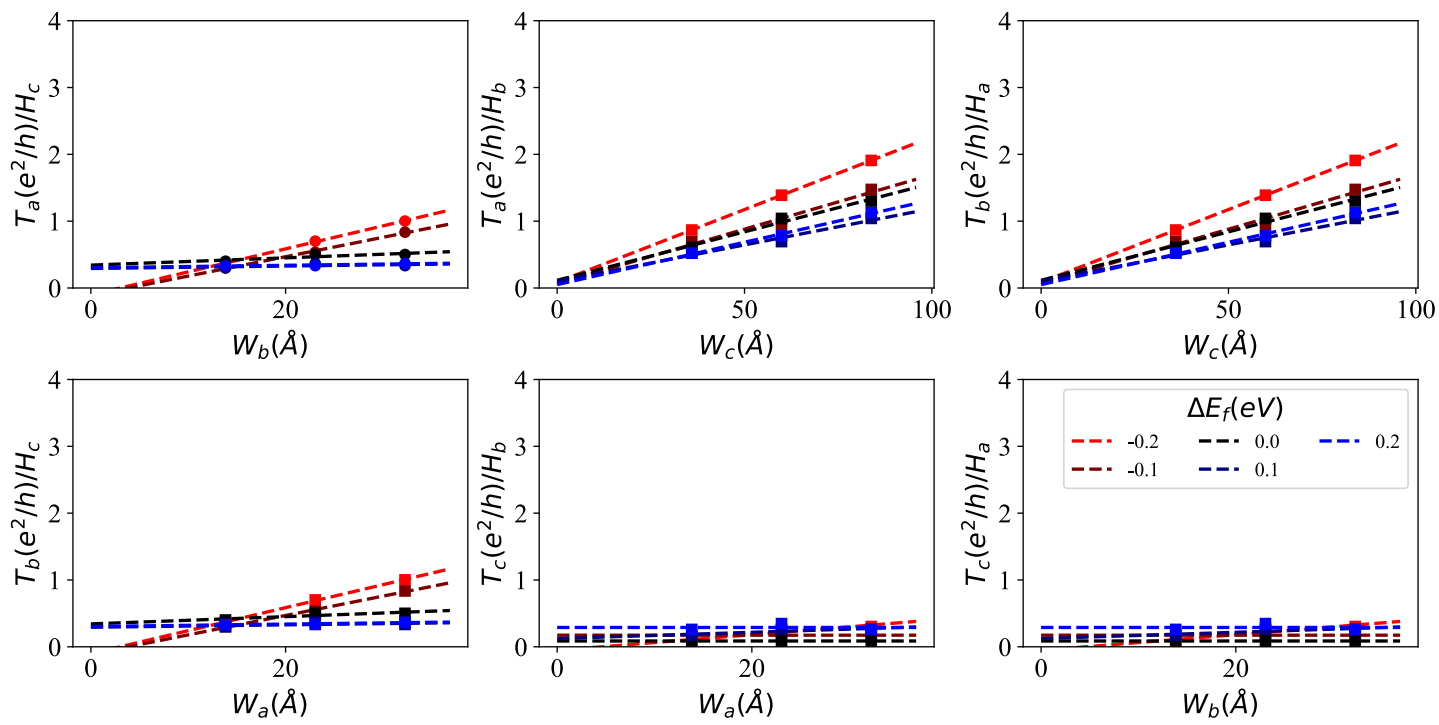

Compound: BiTeI  
Materials Project ID: 22965

Lattice (conventional cell):

| Parameter        | Value    | Unit |
|------------------|----------|------|
| a                | 4.4252   | Å    |
| b                | 4.4252   | Å    |
| c                | 7.3781   | Å    |
| $\alpha$ (alpha) | 90.0000  | °    |
| $\beta$ (beta)   | 90.0000  | °    |
| $\gamma$ (gamma) | 120.0000 | °    |

Crystal structure (conventional cell):

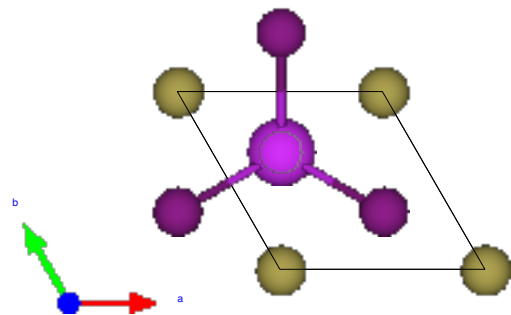

Nanowire Transmission:

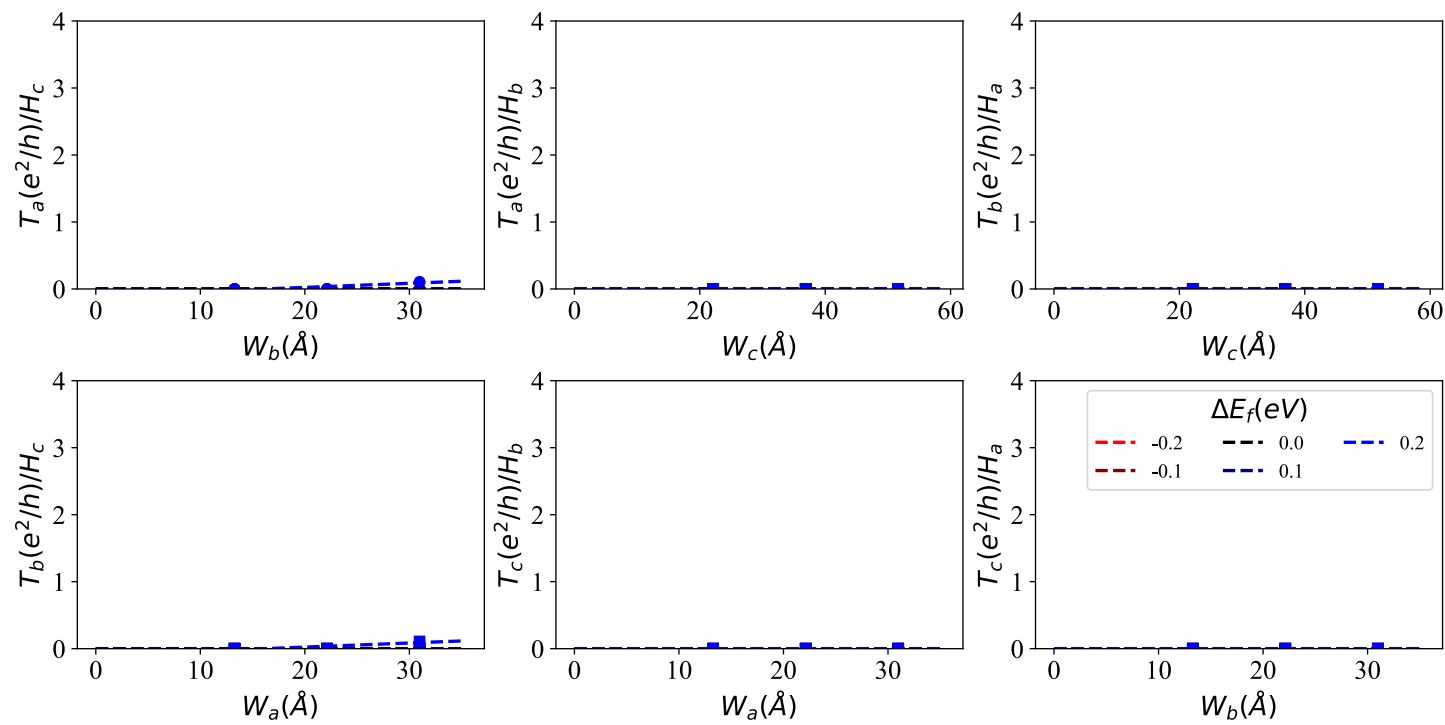



Compound: Ca<sub>2</sub>As  
Materials Project ID: 10106

Lattice (conventional cell):

| Parameter        | Value   | Unit |
|------------------|---------|------|
| a                | 4.5724  | Å    |
| b                | 4.5724  | Å    |
| c                | 15.8762 | Å    |
| $\alpha$ (alpha) | 90.0000 | °    |
| $\beta$ (beta)   | 90.0000 | °    |
| $\gamma$ (gamma) | 90.0000 | °    |

Crystal structure (conventional cell):

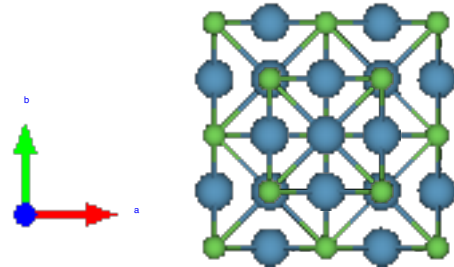

## Nanowire Transmission:

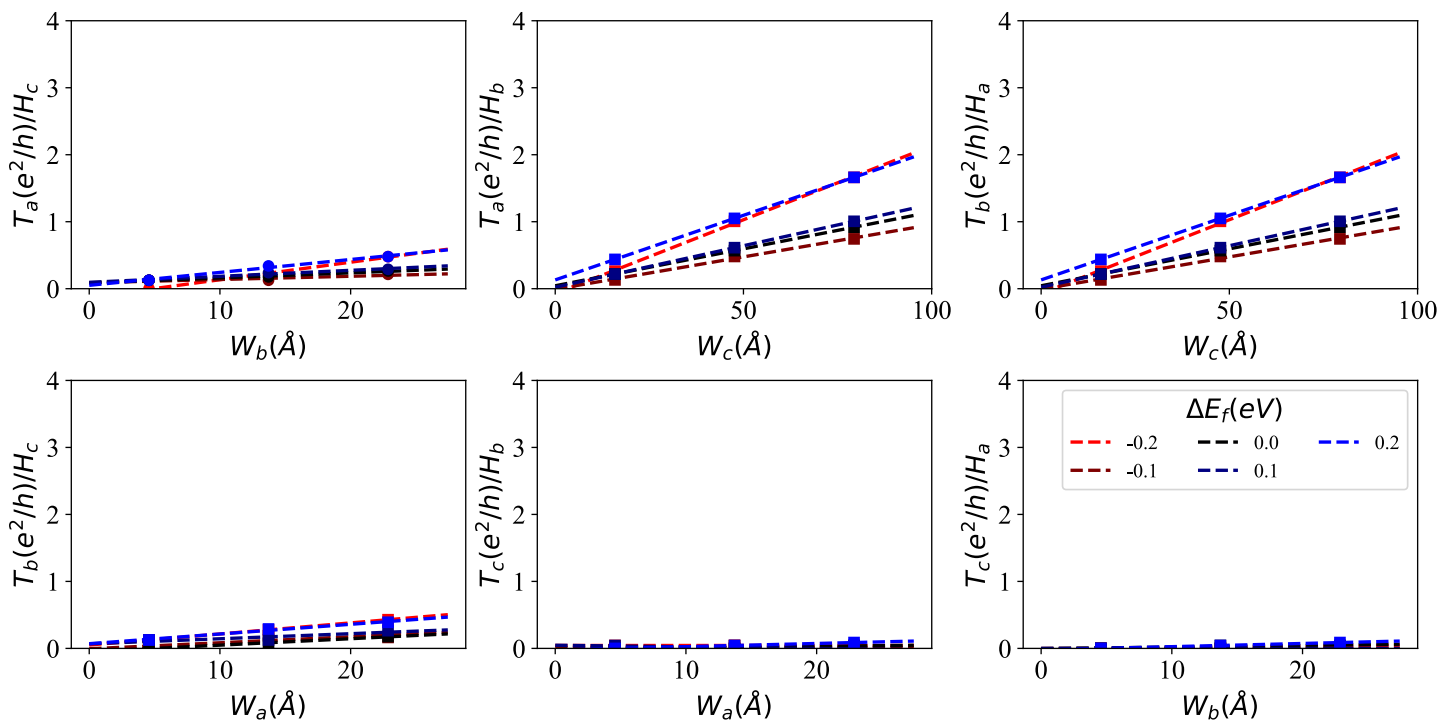

Compound: CaAgAs  
Materials Project ID: 5615

Lattice (conventional cell):

| Parameter        | Value    | Unit |
|------------------|----------|------|
| a                | 7.2663   | Å    |
| b                | 7.2663   | Å    |
| c                | 4.3127   | Å    |
| $\alpha$ (alpha) | 90.0000  | °    |
| $\beta$ (beta)   | 90.0000  | °    |
| $\gamma$ (gamma) | 120.0000 | °    |

Crystal structure (conventional cell):

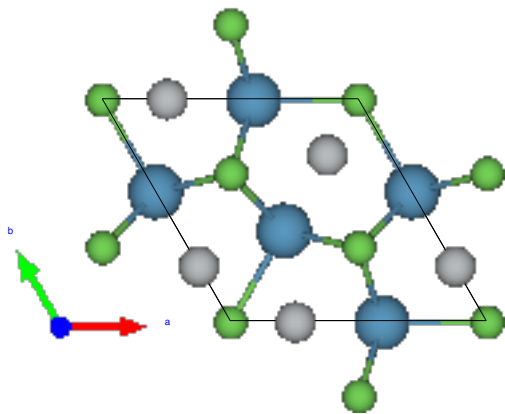

Nanowire Transmission:

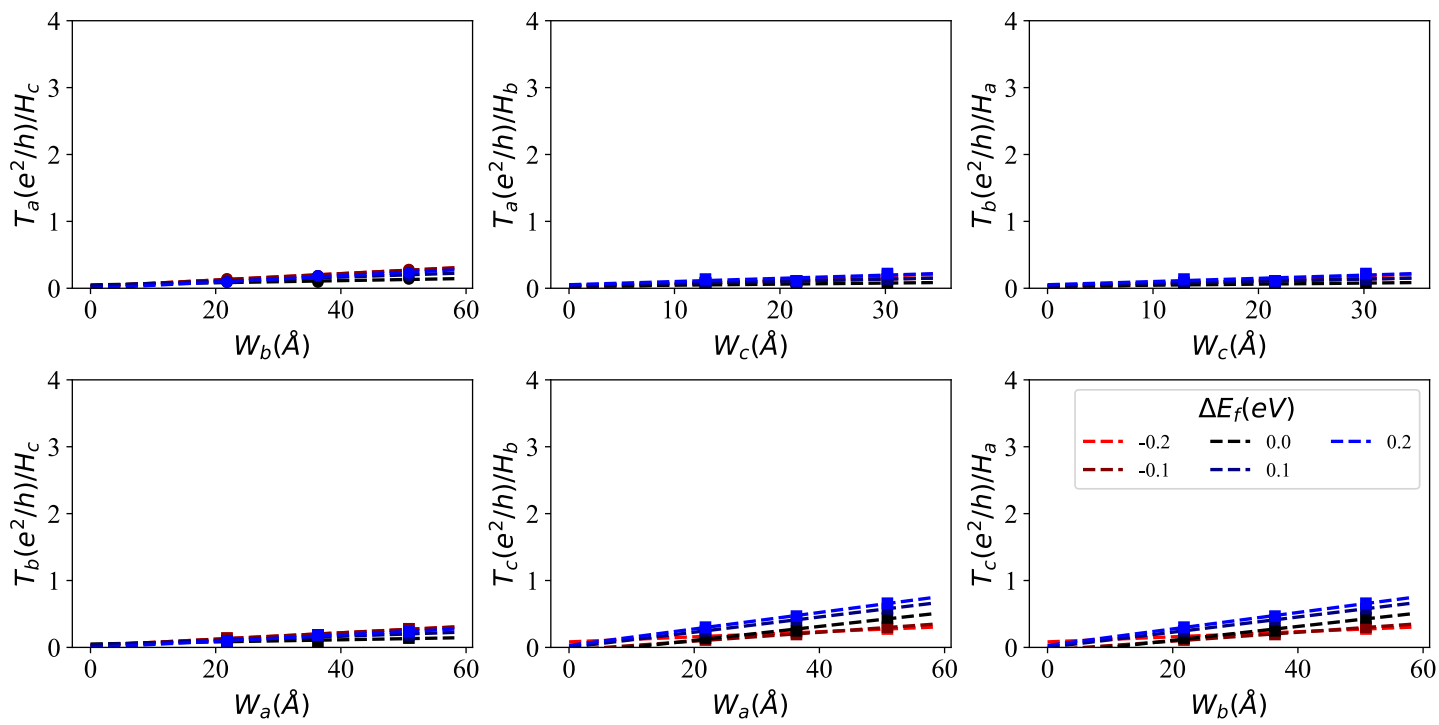

Compound: CaAgBi  
Materials Project ID: 568664

Lattice (conventional cell):

| Parameter        | Value    | Unit |
|------------------|----------|------|
| a                | 4.9065   | Å    |
| b                | 4.9065   | Å    |
| c                | 7.8429   | Å    |
| $\alpha$ (alpha) | 90.0000  | °    |
| $\beta$ (beta)   | 90.0000  | °    |
| $\gamma$ (gamma) | 120.0000 | °    |

Crystal structure (conventional cell):

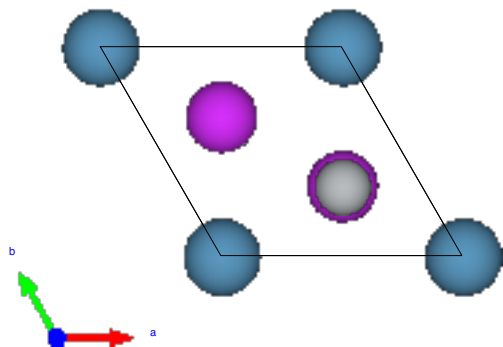

Nanowire Transmission:

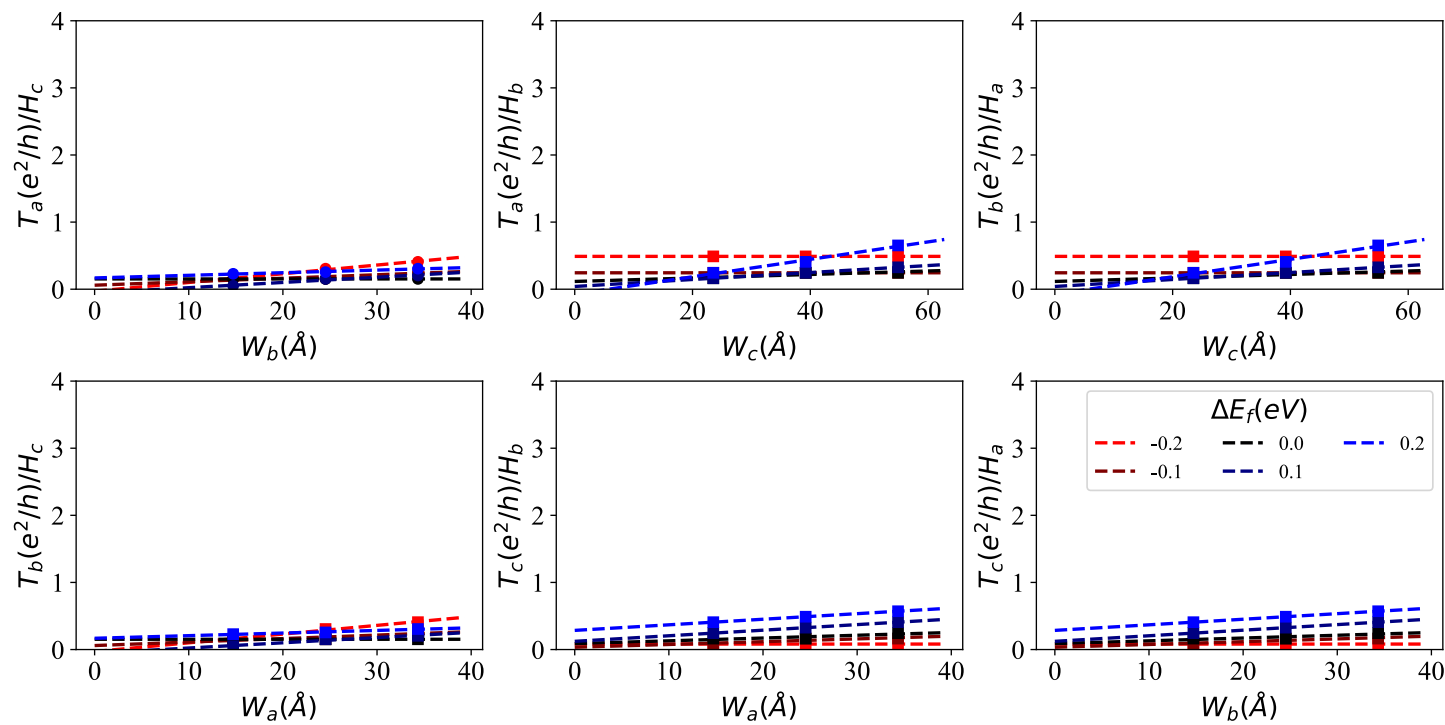

Compound: CaAgP  
Materials Project ID: 12277

Lattice (conventional cell):

| Parameter        | Value    | Unit |
|------------------|----------|------|
| a                | 7.0768   | Å    |
| b                | 7.0768   | Å    |
| c                | 4.2030   | Å    |
| $\alpha$ (alpha) | 90.0000  | °    |
| $\beta$ (beta)   | 90.0000  | °    |
| $\gamma$ (gamma) | 120.0000 | °    |

Crystal structure (conventional cell):

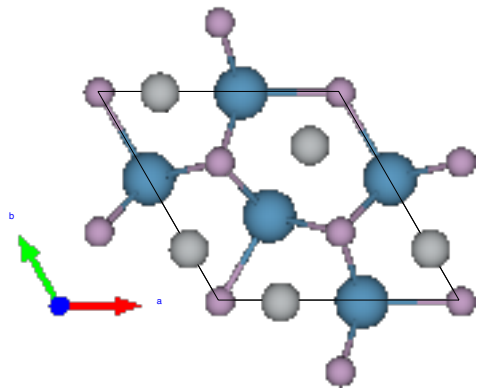

Nanowire Transmission:

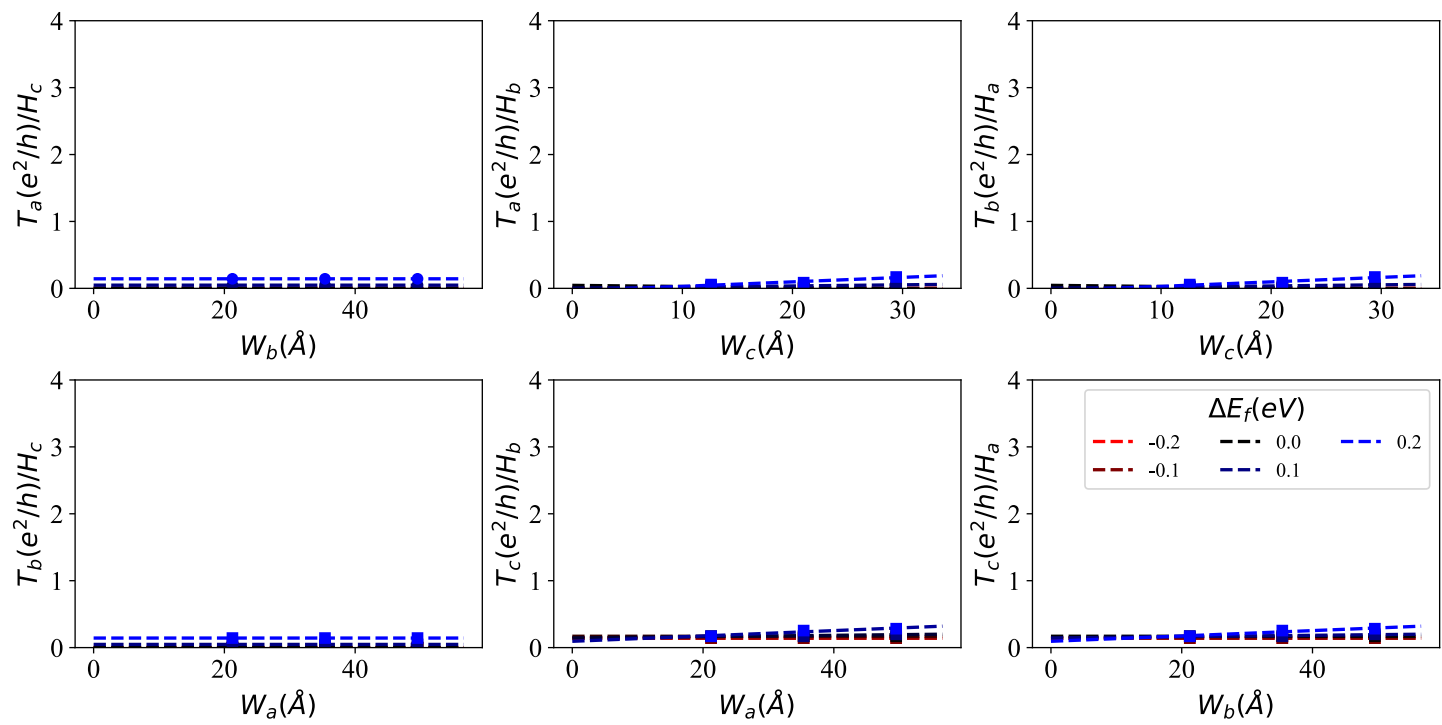

Compound: CaB<sub>6</sub>  
Materials Project ID: 865

Lattice (conventional cell):

| Parameter | Value   | Unit |
|-----------|---------|------|
| a         | 4.1501  | Å    |
| b         | 4.1501  | Å    |
| c         | 4.1501  | Å    |
| α (alpha) | 90.0000 | °    |
| β (beta)  | 90.0000 | °    |
| γ (gamma) | 90.0000 | °    |

Crystal structure (conventional cell):

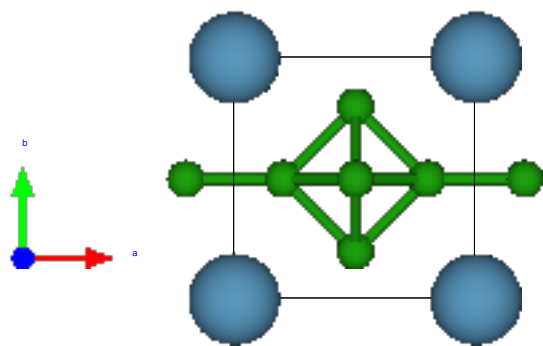

Nanowire Transmission:

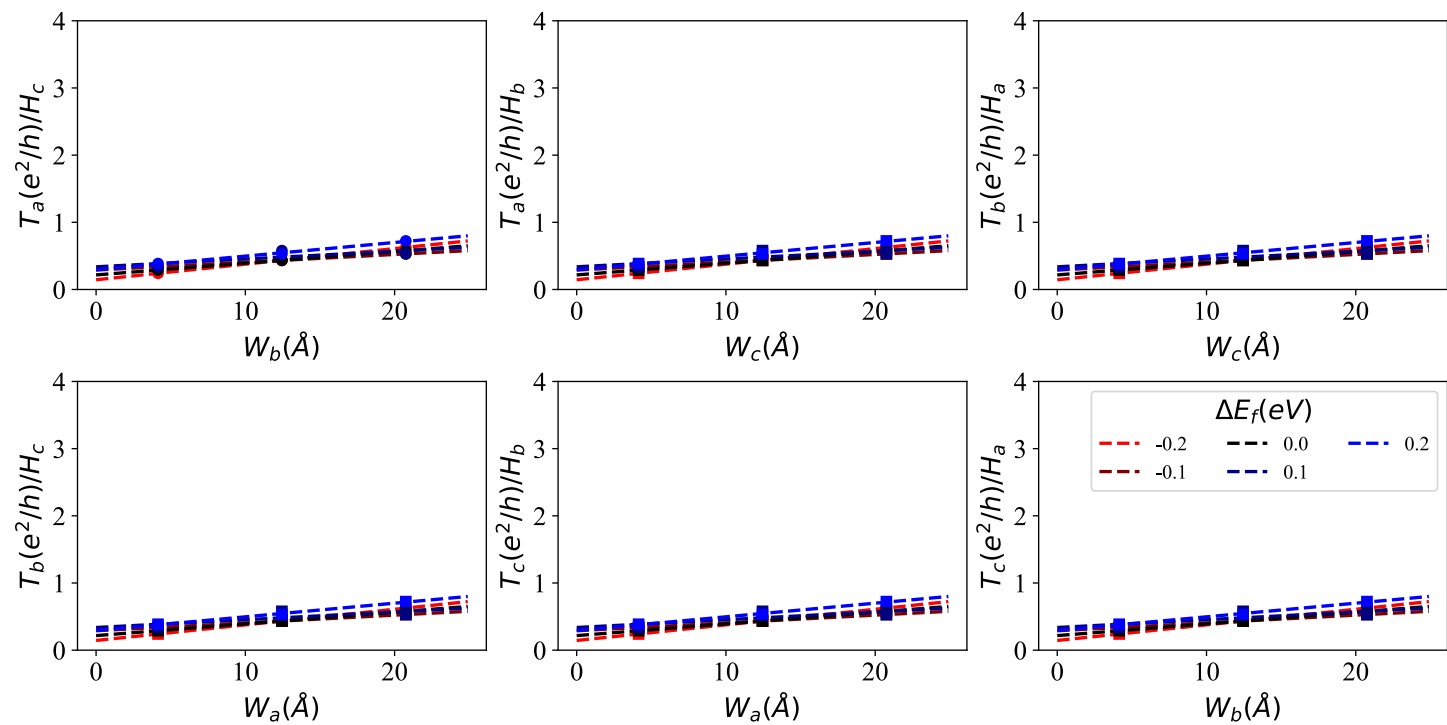

Compound: CaBiAu  
Materials Project ID: 1018657

Lattice (conventional cell):

| Parameter        | Value    | Unit |
|------------------|----------|------|
| a                | 4.8612   | Å    |
| b                | 4.8612   | Å    |
| c                | 7.9224   | Å    |
| $\alpha$ (alpha) | 90.0000  | °    |
| $\beta$ (beta)   | 90.0000  | °    |
| $\gamma$ (gamma) | 120.0000 | °    |

Crystal structure (conventional cell):

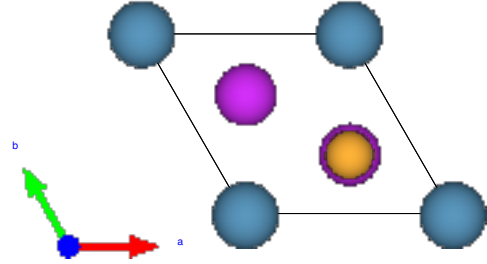

Nanowire Transmission:

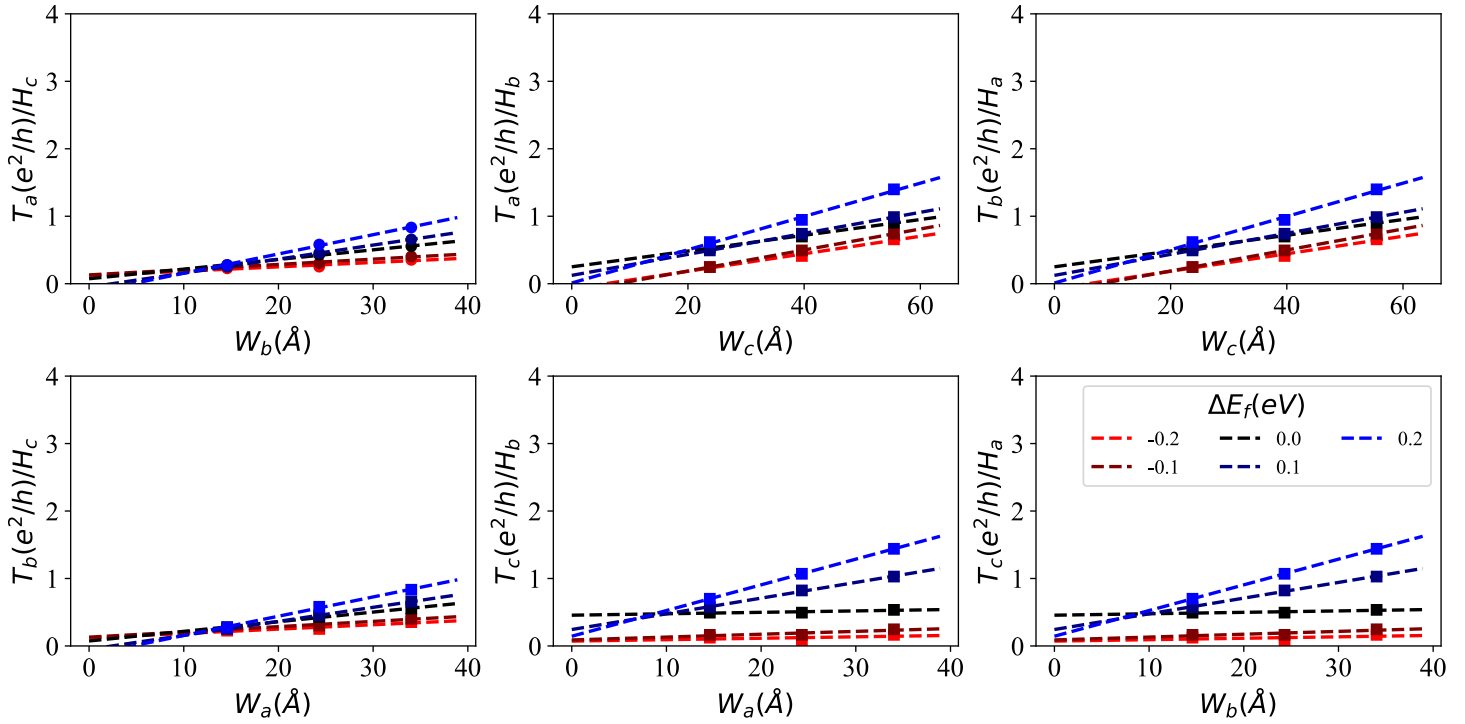

Compound:  $\text{CaC}_2$   
Materials Project ID: 1077545

Lattice (conventional cell):

| Parameter        | Value   | Unit |
|------------------|---------|------|
| a                | 3.7480  | Å    |
| b                | 8.7387  | Å    |
| c                | 4.7766  | Å    |
| $\alpha$ (alpha) | 90.0000 | °    |
| $\beta$ (beta)   | 90.0000 | °    |
| $\gamma$ (gamma) | 90.0000 | °    |

Crystal structure (conventional cell):

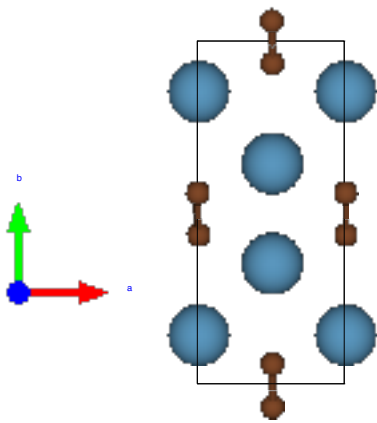

Nanowire Transmission:

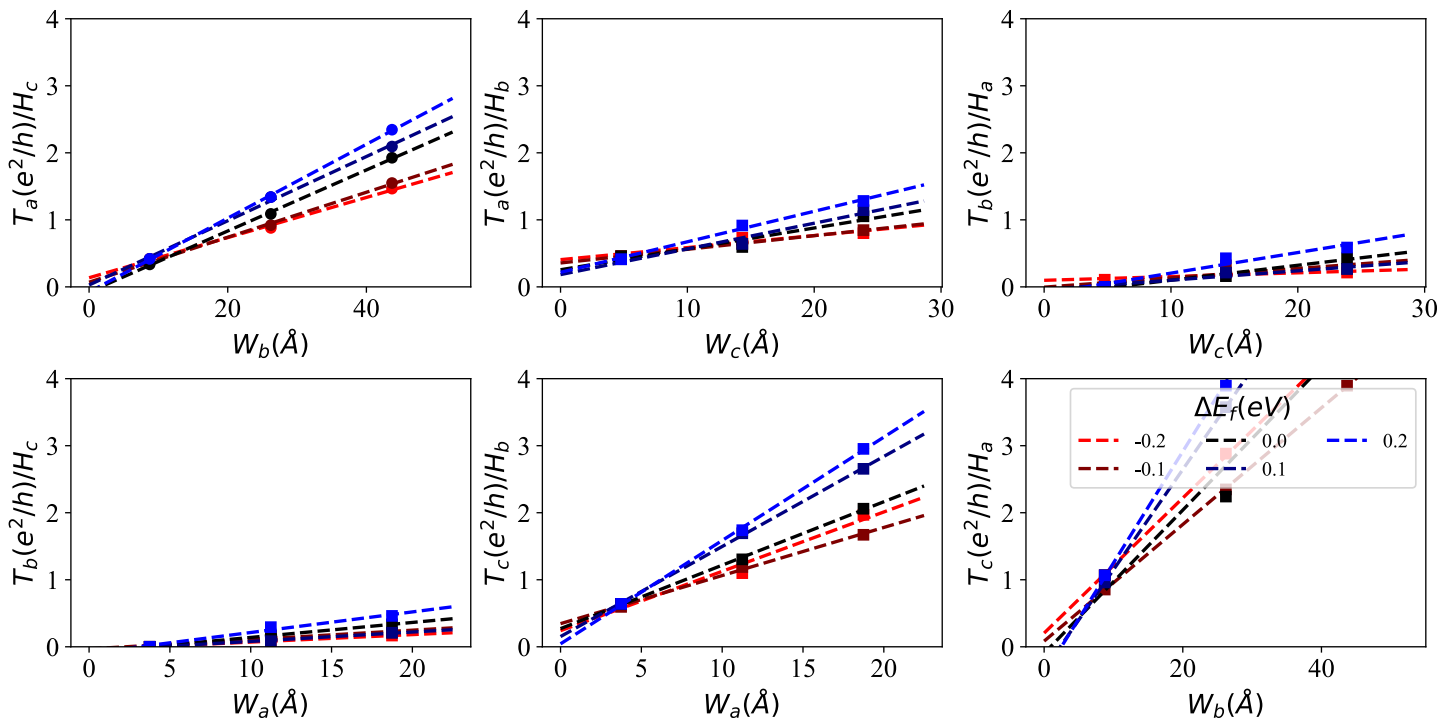

Compound:  $\text{CaSi}_2$   
Materials Project ID: 8372

Lattice (conventional cell):

| Parameter        | Value    | Unit |
|------------------|----------|------|
| a                | 3.8878   | Å    |
| b                | 3.8878   | Å    |
| c                | 4.9460   | Å    |
| $\alpha$ (alpha) | 90.0000  | °    |
| $\beta$ (beta)   | 90.0000  | °    |
| $\gamma$ (gamma) | 120.0000 | °    |

Crystal structure (conventional cell):

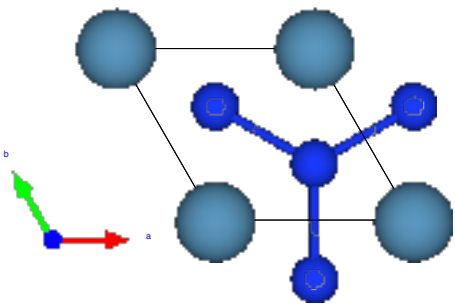

Nanowire Transmission:

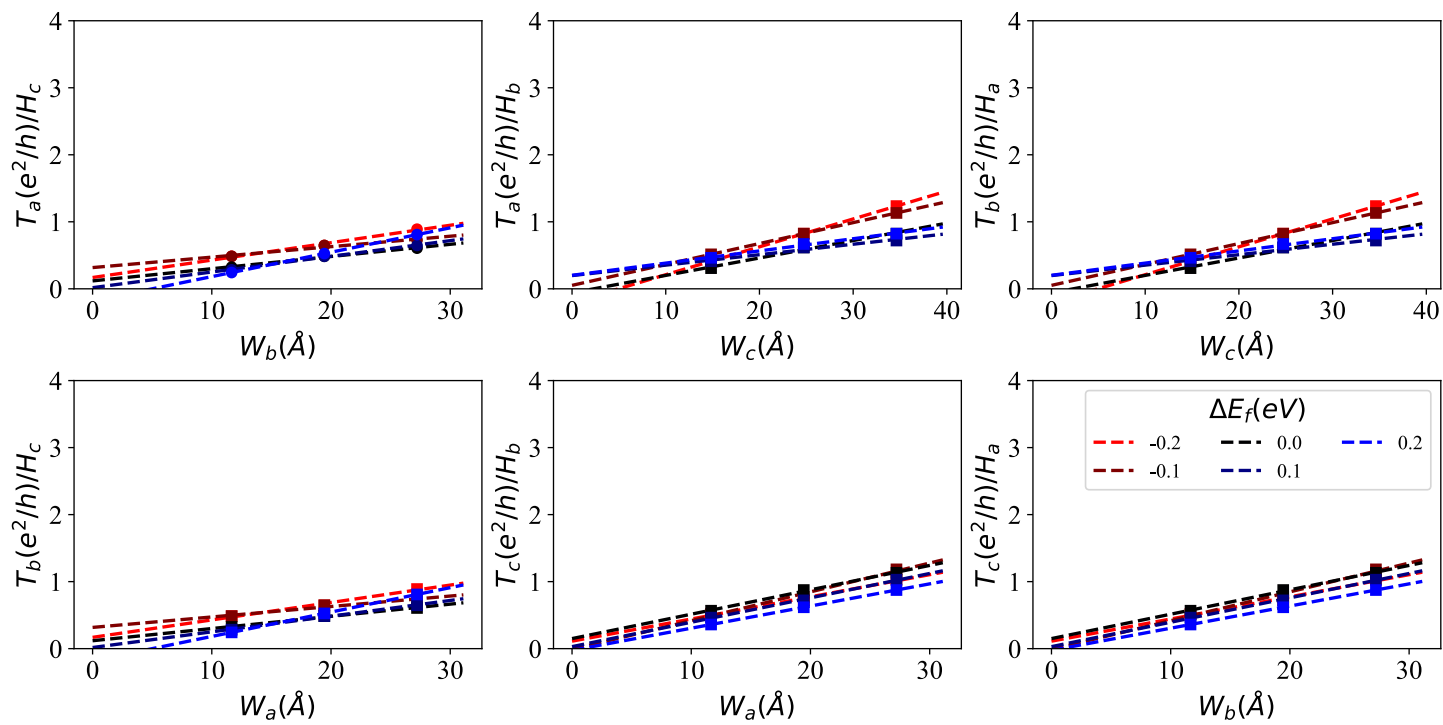



Compound: CaSnHg  
Materials Project ID: 1019104

Lattice (conventional cell):

| Parameter        | Value    | Unit |
|------------------|----------|------|
| a                | 4.9042   | Å    |
| b                | 4.9042   | Å    |
| c                | 7.8216   | Å    |
| $\alpha$ (alpha) | 90.0000  | °    |
| $\beta$ (beta)   | 90.0000  | °    |
| $\gamma$ (gamma) | 120.0000 | °    |

Crystal structure (conventional cell):

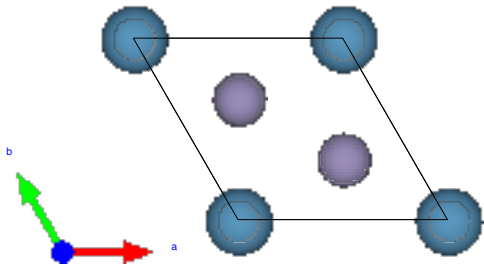

Nanowire Transmission:

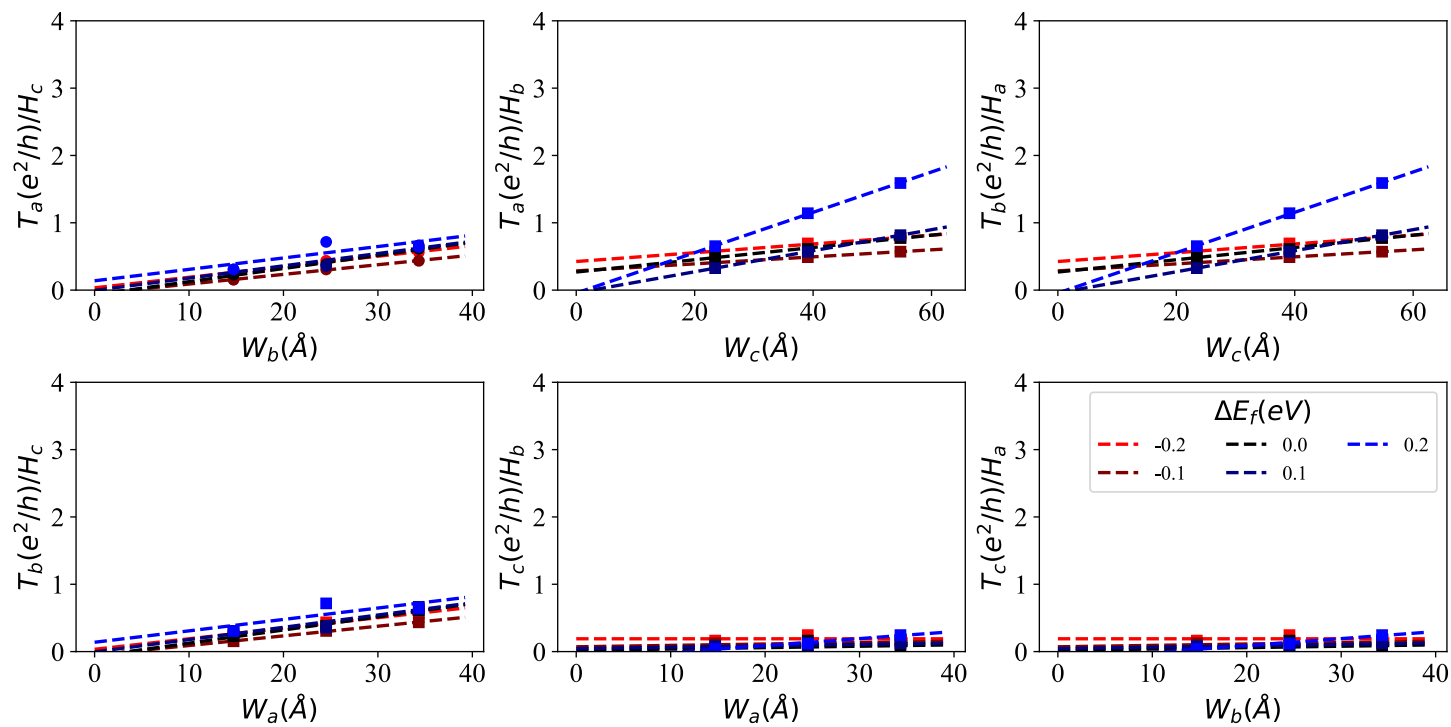

Compound: CaTe  
Materials Project ID: 10684

Lattice (conventional cell):

| Parameter        | Value   | Unit |
|------------------|---------|------|
| a                | 3.9261  | Å    |
| b                | 3.9261  | Å    |
| c                | 3.9261  | Å    |
| $\alpha$ (alpha) | 90.0000 | °    |
| $\beta$ (beta)   | 90.0000 | °    |
| $\gamma$ (gamma) | 90.0000 | °    |

Crystal structure (conventional cell):

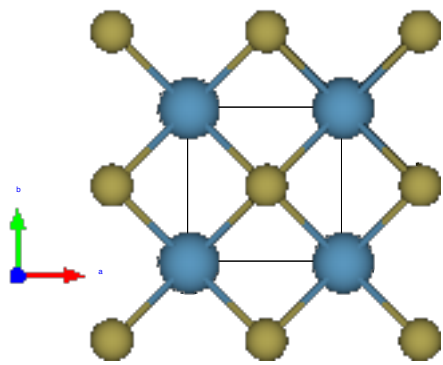

Nanowire Transmission:

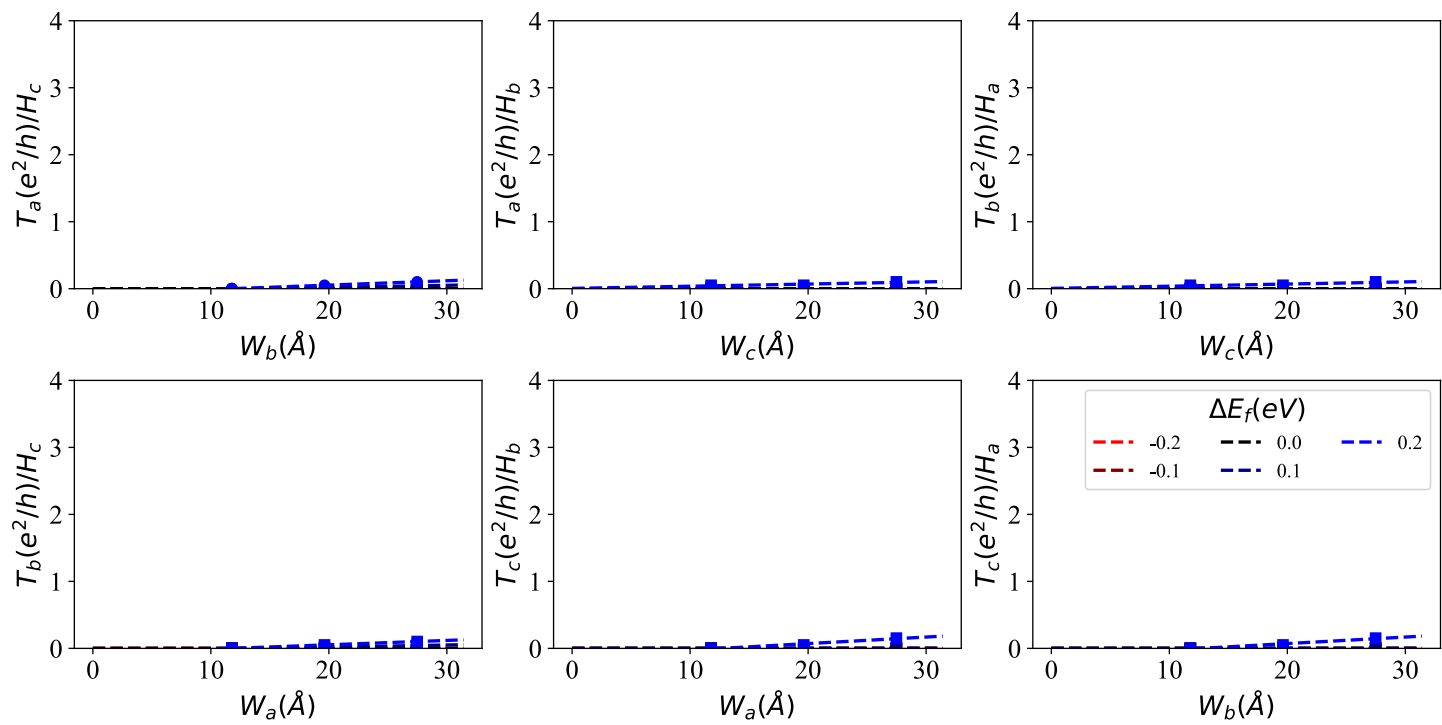

Compound:  $\text{CaP}_3$   
Materials Project ID: 9122

Lattice (conventional cell):

| Parameter        | Value   | Unit |
|------------------|---------|------|
| a                | 5.6095  | Å    |
| b                | 5.6390  | Å    |
| c                | 5.6946  | Å    |
| $\alpha$ (alpha) | 70.0761 | °    |
| $\beta$ (beta)   | 79.6272 | °    |
| $\gamma$ (gamma) | 74.6843 | °    |

Crystal structure (conventional cell):

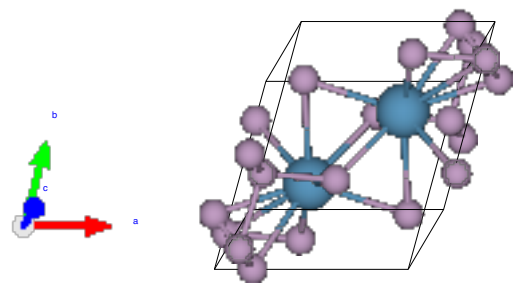

Nanowire Transmission:

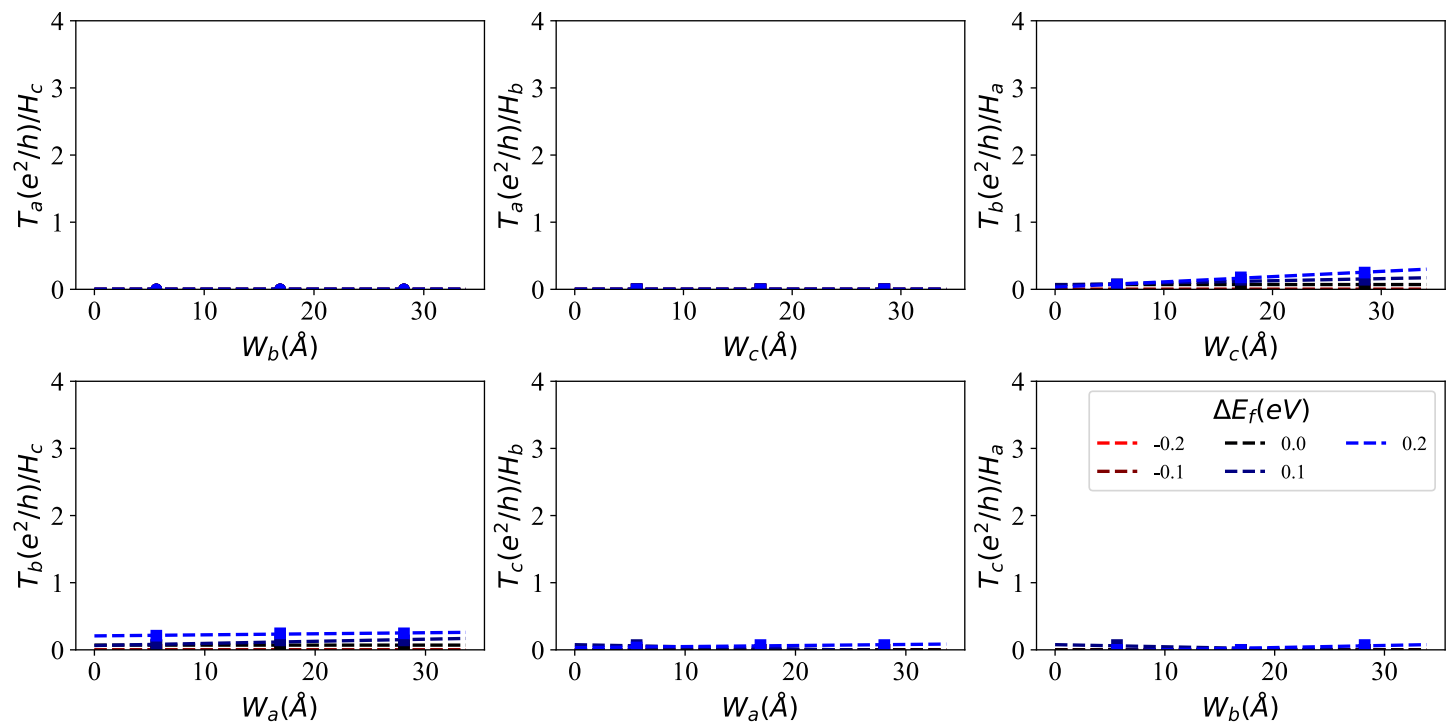

Compound: Co  
Materials Project ID: 54

Lattice (conventional cell):

| Parameter        | Value    | Unit |
|------------------|----------|------|
| a                | 2.5008   | Å    |
| b                | 2.5008   | Å    |
| c                | 4.0333   | Å    |
| $\alpha$ (alpha) | 90.0000  | °    |
| $\beta$ (beta)   | 90.0000  | °    |
| $\gamma$ (gamma) | 120.0000 | °    |

Crystal structure (conventional cell):

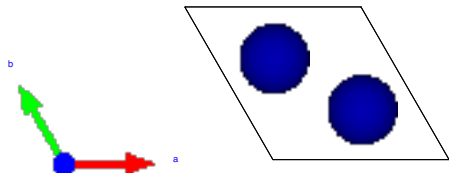

Nanowire Transmission:

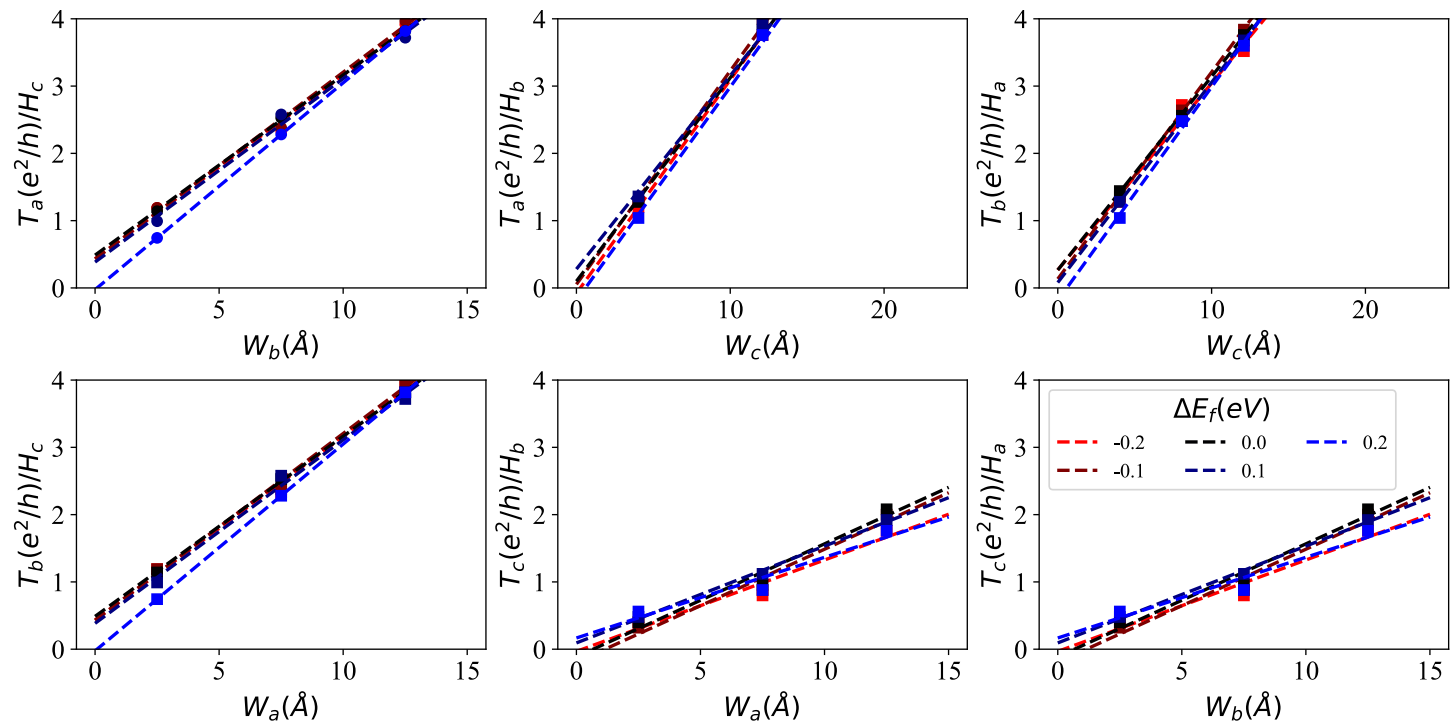

Compound: CoGe  
Materials Project ID: 10692

Lattice (conventional cell):

| Parameter        | Value   | Unit |
|------------------|---------|------|
| a                | 4.6370  | Å    |
| b                | 4.6370  | Å    |
| c                | 4.6370  | Å    |
| $\alpha$ (alpha) | 90.0000 | °    |
| $\beta$ (beta)   | 90.0000 | °    |
| $\gamma$ (gamma) | 90.0000 | °    |

Crystal structure (conventional cell):

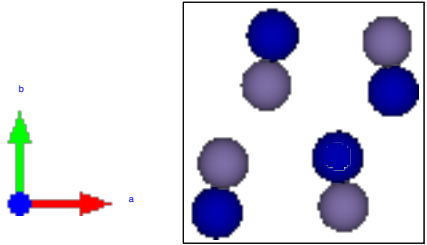

Nanowire Transmission:

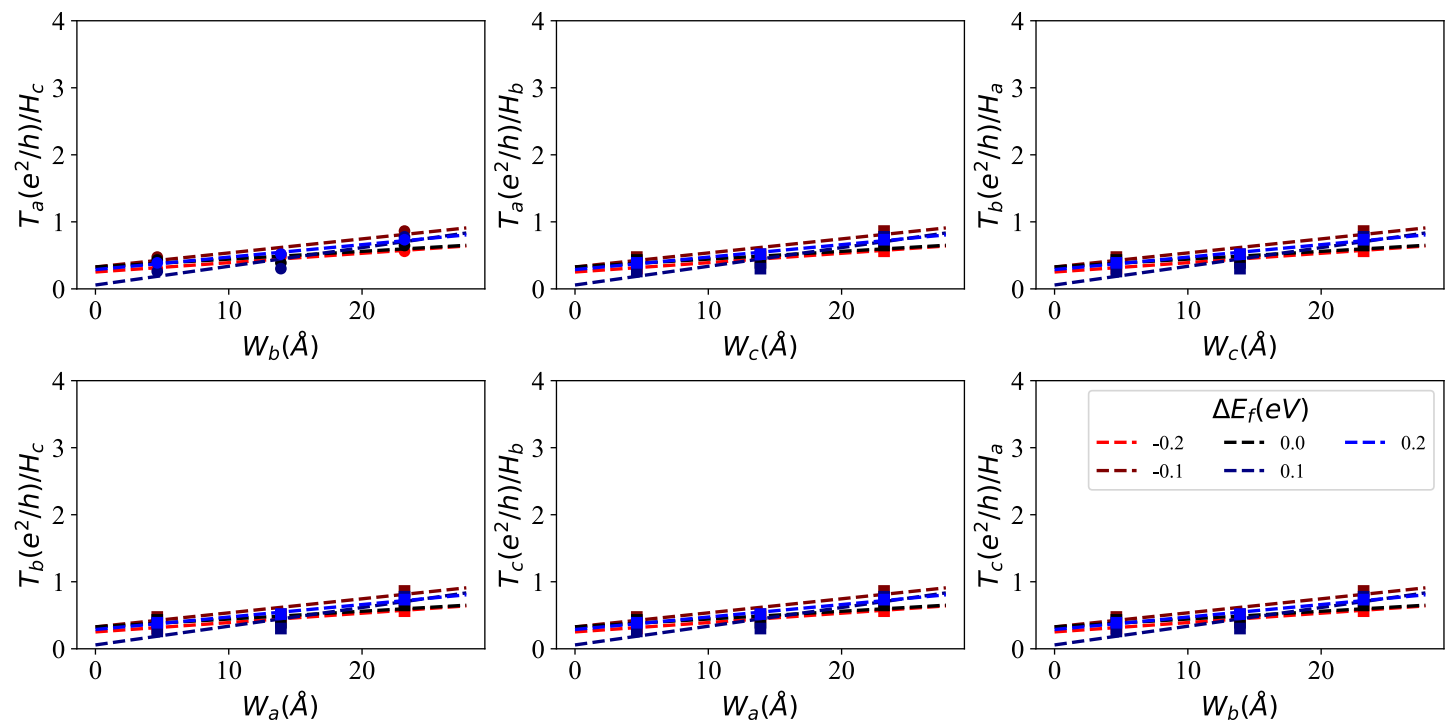

Compound: CoSi  
Materials Project ID: 7577

Lattice (conventional cell):

| Parameter        | Value   | Unit |
|------------------|---------|------|
| a                | 4.4332  | Å    |
| b                | 4.4332  | Å    |
| c                | 4.4332  | Å    |
| $\alpha$ (alpha) | 90.0000 | °    |
| $\beta$ (beta)   | 90.0000 | °    |
| $\gamma$ (gamma) | 90.0000 | °    |

Crystal structure (conventional cell):

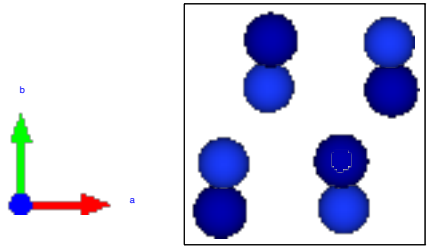

Nanowire Transmission:

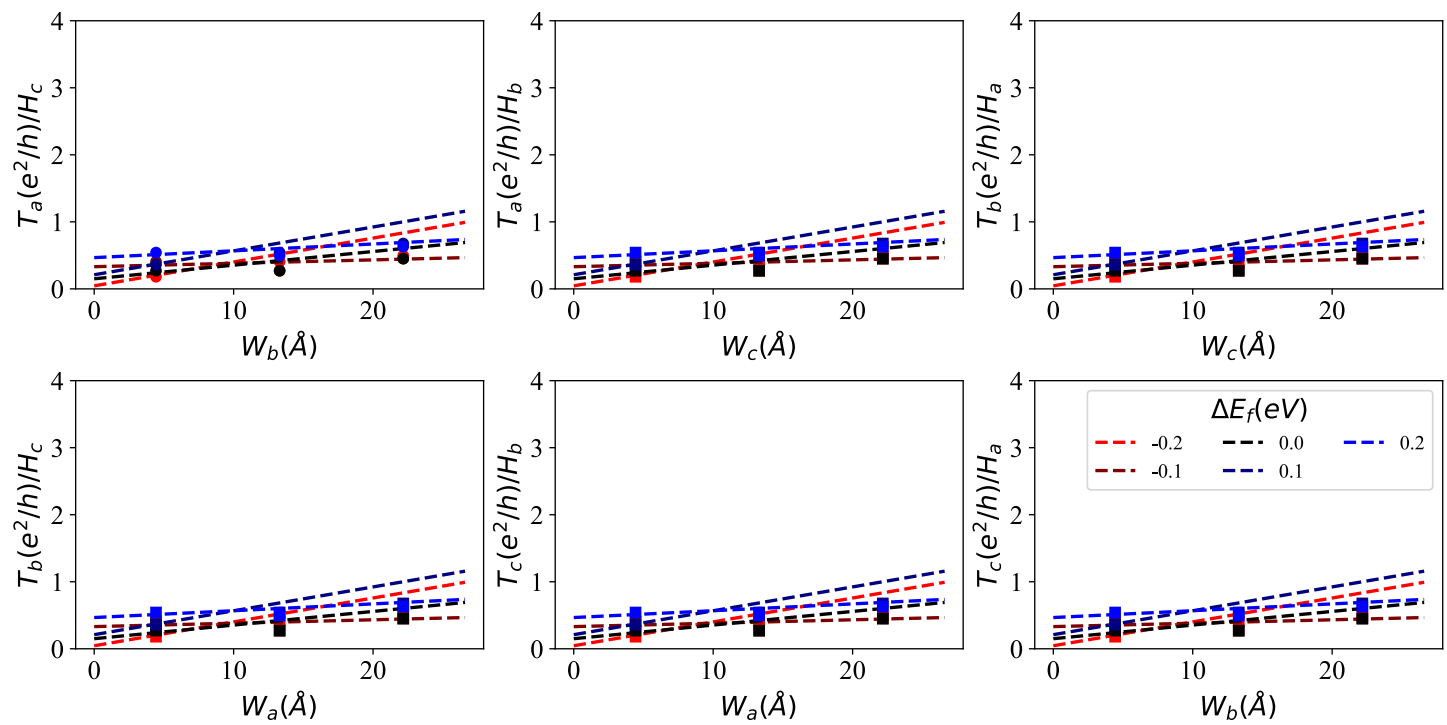

Compound: CoPtO<sub>2</sub>  
Materials Project ID: 19210

Lattice (conventional cell):

| Parameter | Value    | Unit |
|-----------|----------|------|
| a         | 2.8847   | Å    |
| b         | 2.8847   | Å    |
| c         | 18.2033  | Å    |
| α (alpha) | 90.0000  | °    |
| β (beta)  | 90.0000  | °    |
| γ (gamma) | 120.0000 | °    |

Crystal structure (conventional cell):

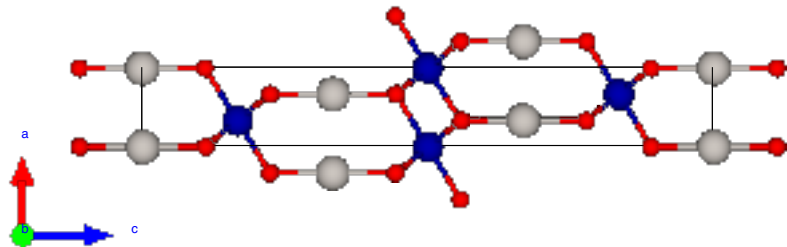

Nanowire Transmission:

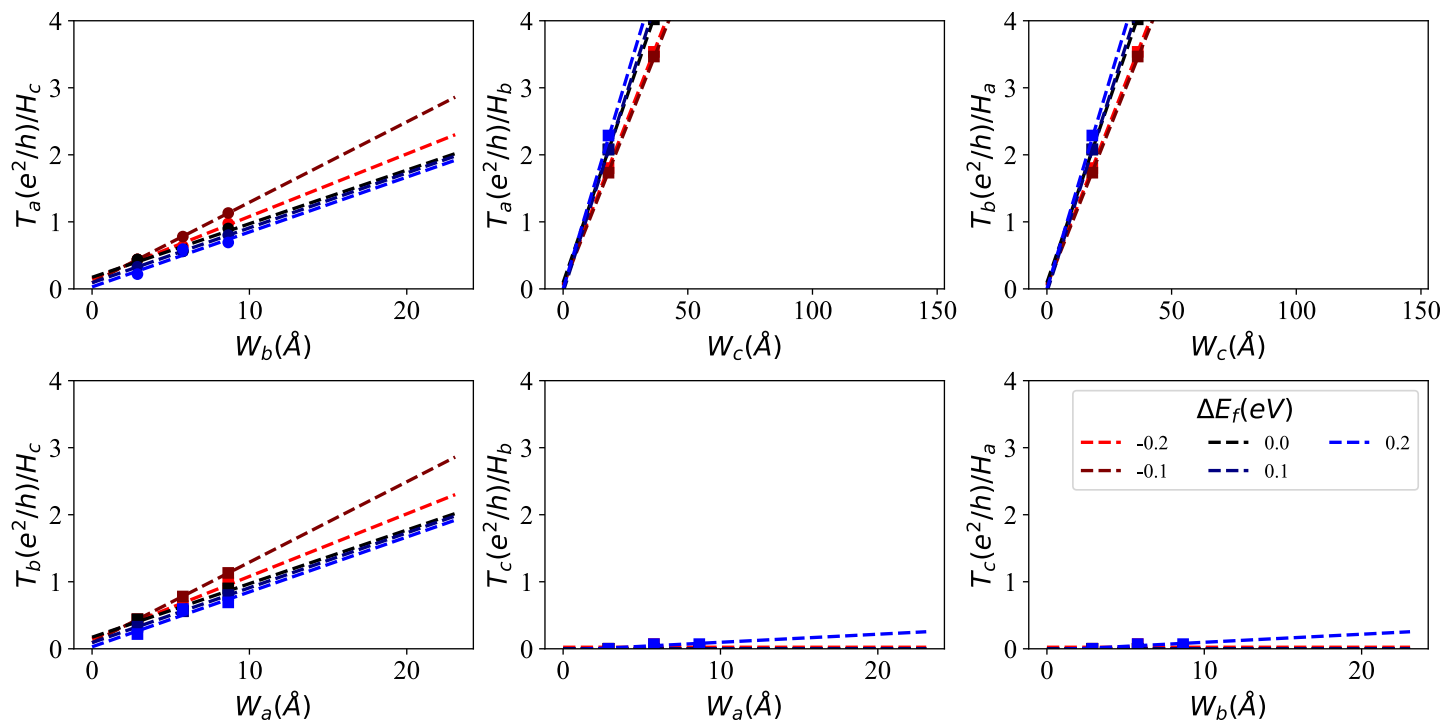

Compound: Cu  
Materials Project ID: 30

Lattice (conventional cell):

| Parameter        | Value   | Unit |
|------------------|---------|------|
| a                | 3.6213  | Å    |
| b                | 3.6213  | Å    |
| c                | 3.6213  | Å    |
| $\alpha$ (alpha) | 90.0000 | °    |
| $\beta$ (beta)   | 90.0000 | °    |
| $\gamma$ (gamma) | 90.0000 | °    |

Crystal structure (conventional cell):

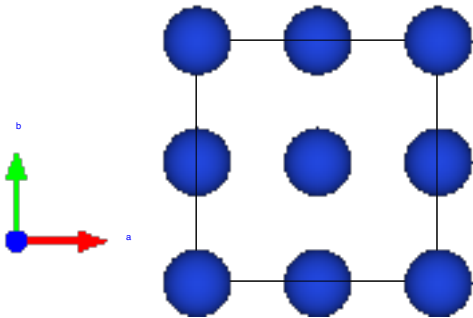

Nanowire Transmission:

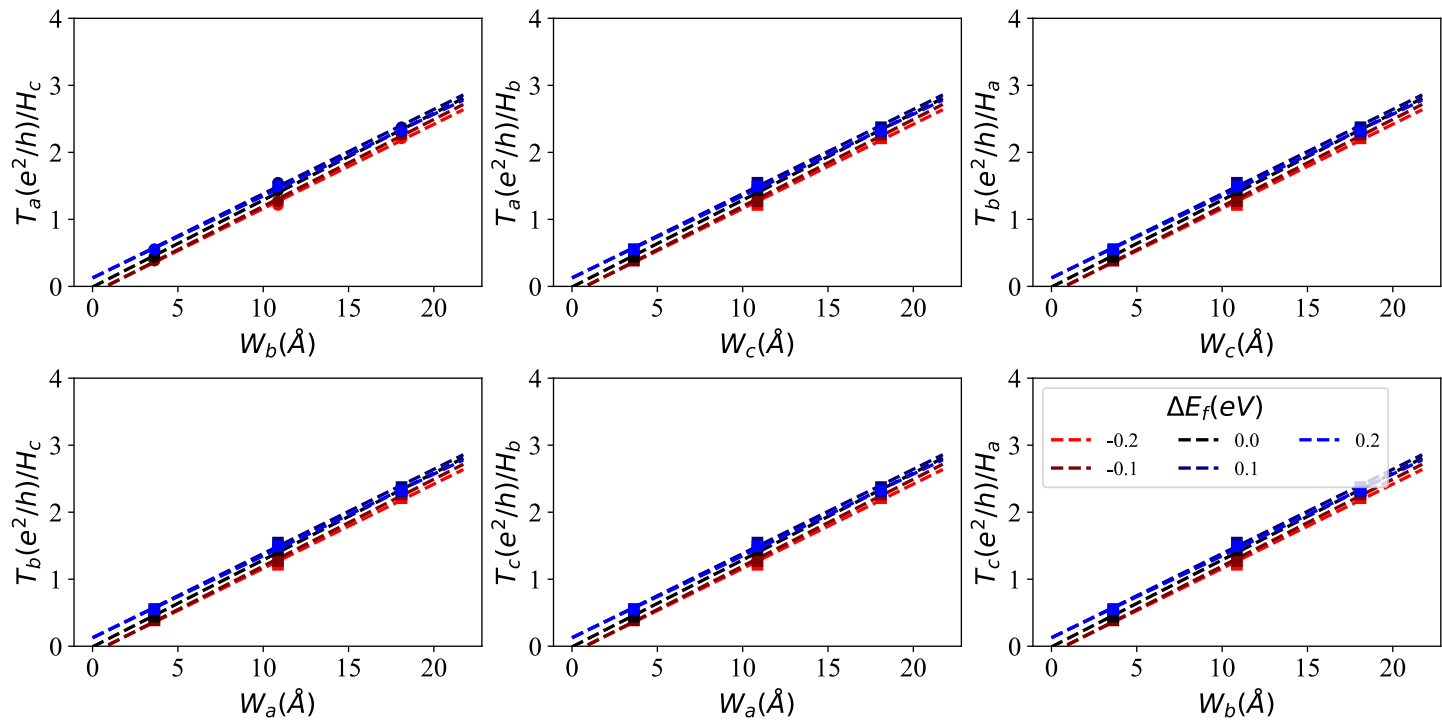



Compound:  $\text{Cu}_3\text{AsSe}_4$   
Materials Project ID: 675626

Lattice (conventional cell):

| Parameter        | Value   | Unit |
|------------------|---------|------|
| a                | 5.6212  | Å    |
| b                | 5.6212  | Å    |
| c                | 11.1400 | Å    |
| $\alpha$ (alpha) | 90.0000 | °    |
| $\beta$ (beta)   | 90.0000 | °    |
| $\gamma$ (gamma) | 90.0000 | °    |

Crystal structure (conventional cell):

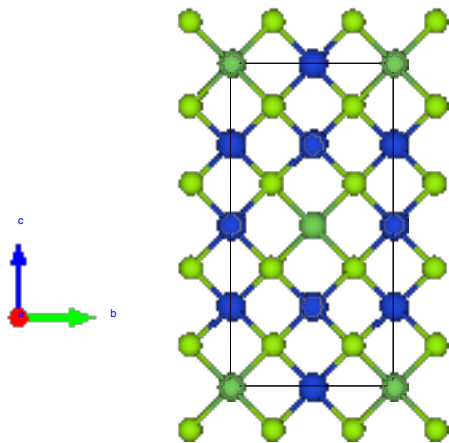

Nanowire Transmission:

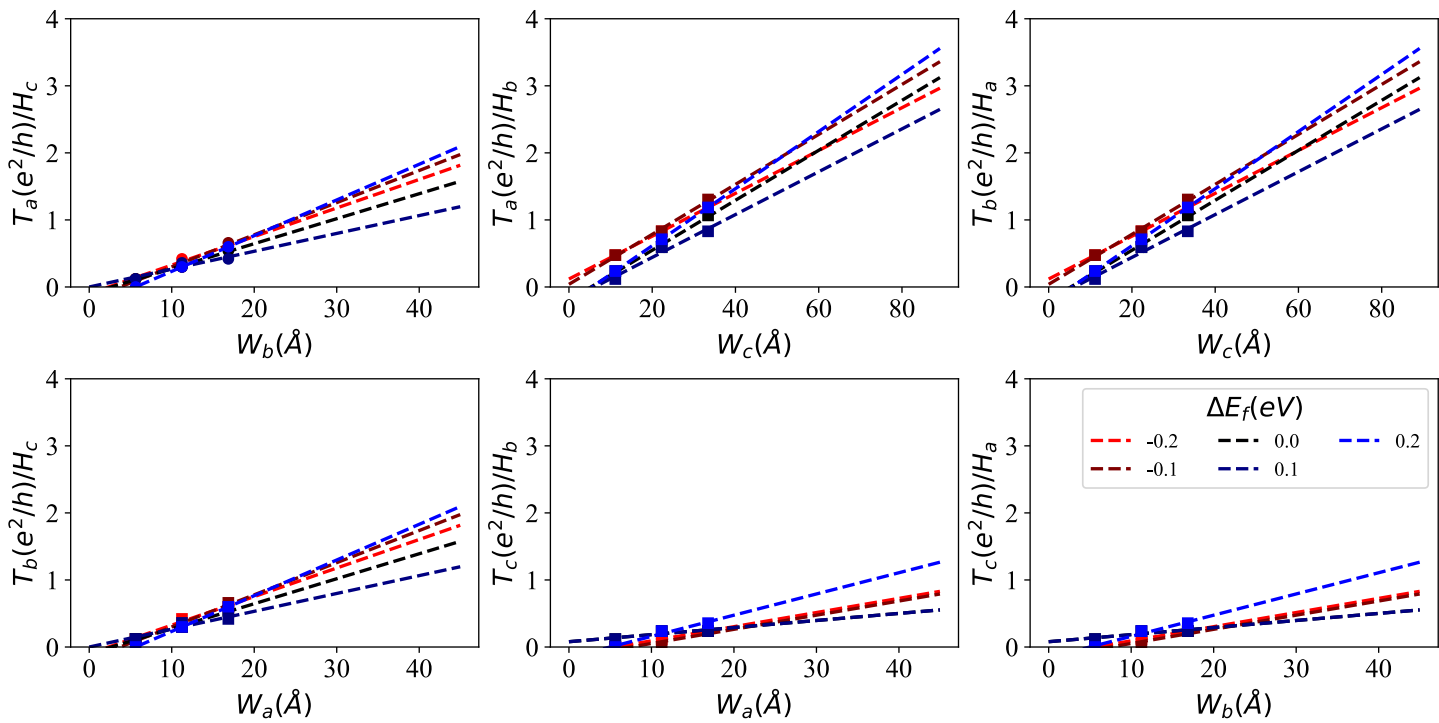

Compound: GaPd  
Materials Project ID: 1078526

Lattice (conventional cell):

| Parameter        | Value   | Unit |
|------------------|---------|------|
| a                | 4.9634  | Å    |
| b                | 4.9634  | Å    |
| c                | 4.9634  | Å    |
| $\alpha$ (alpha) | 90.0000 | °    |
| $\beta$ (beta)   | 90.0000 | °    |
| $\gamma$ (gamma) | 90.0000 | °    |

Crystal structure (conventional cell):

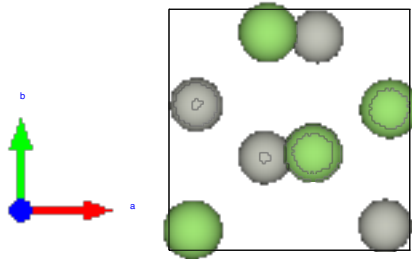

Nanowire Transmission:

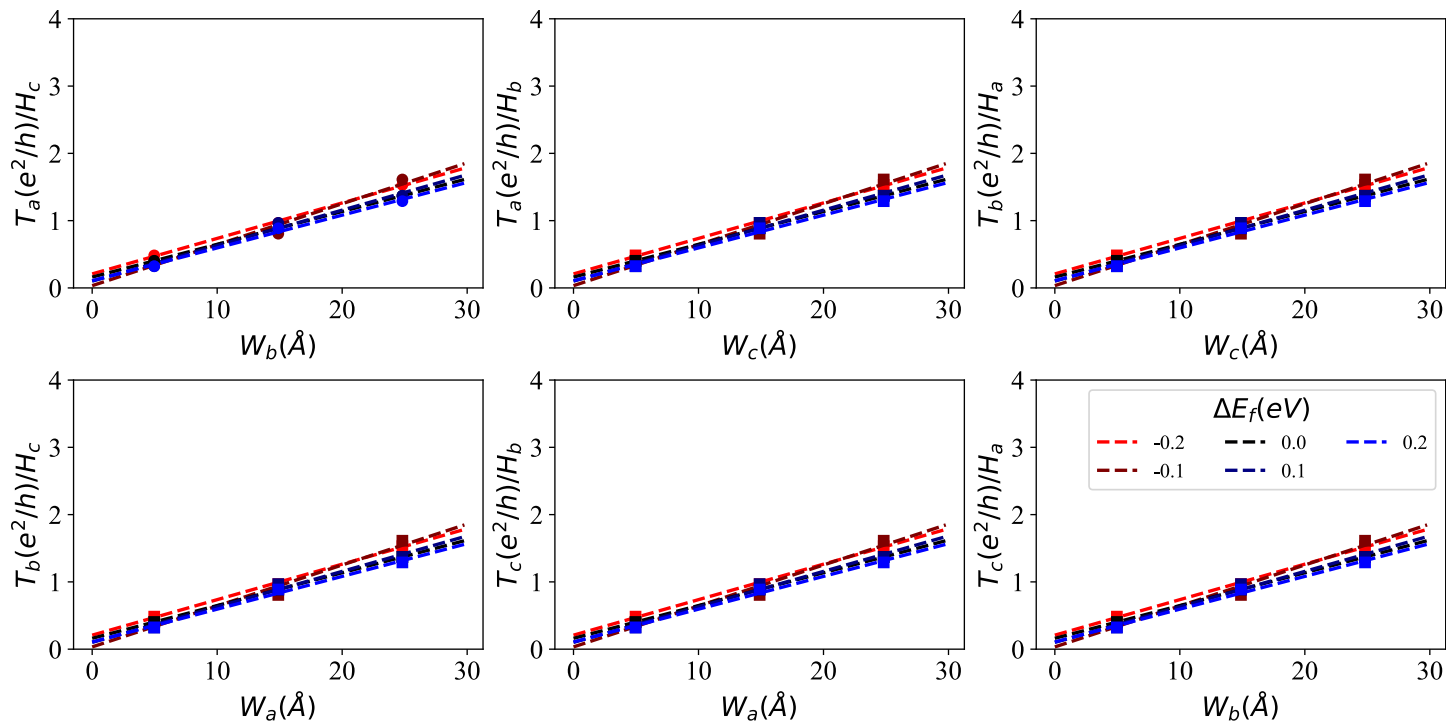

Compound: GaPt  
Materials Project ID: 1025551

Lattice (conventional cell):

| Parameter        | Value   | Unit |
|------------------|---------|------|
| a                | 4.9729  | Å    |
| b                | 4.9729  | Å    |
| c                | 4.9729  | Å    |
| $\alpha$ (alpha) | 90.0000 | °    |
| $\beta$ (beta)   | 90.0000 | °    |
| $\gamma$ (gamma) | 90.0000 | °    |

Crystal structure (conventional cell):

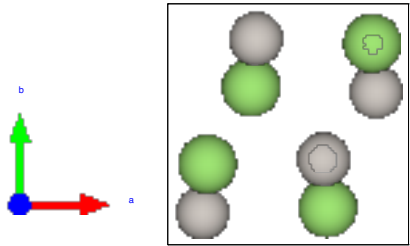

Nanowire Transmission:

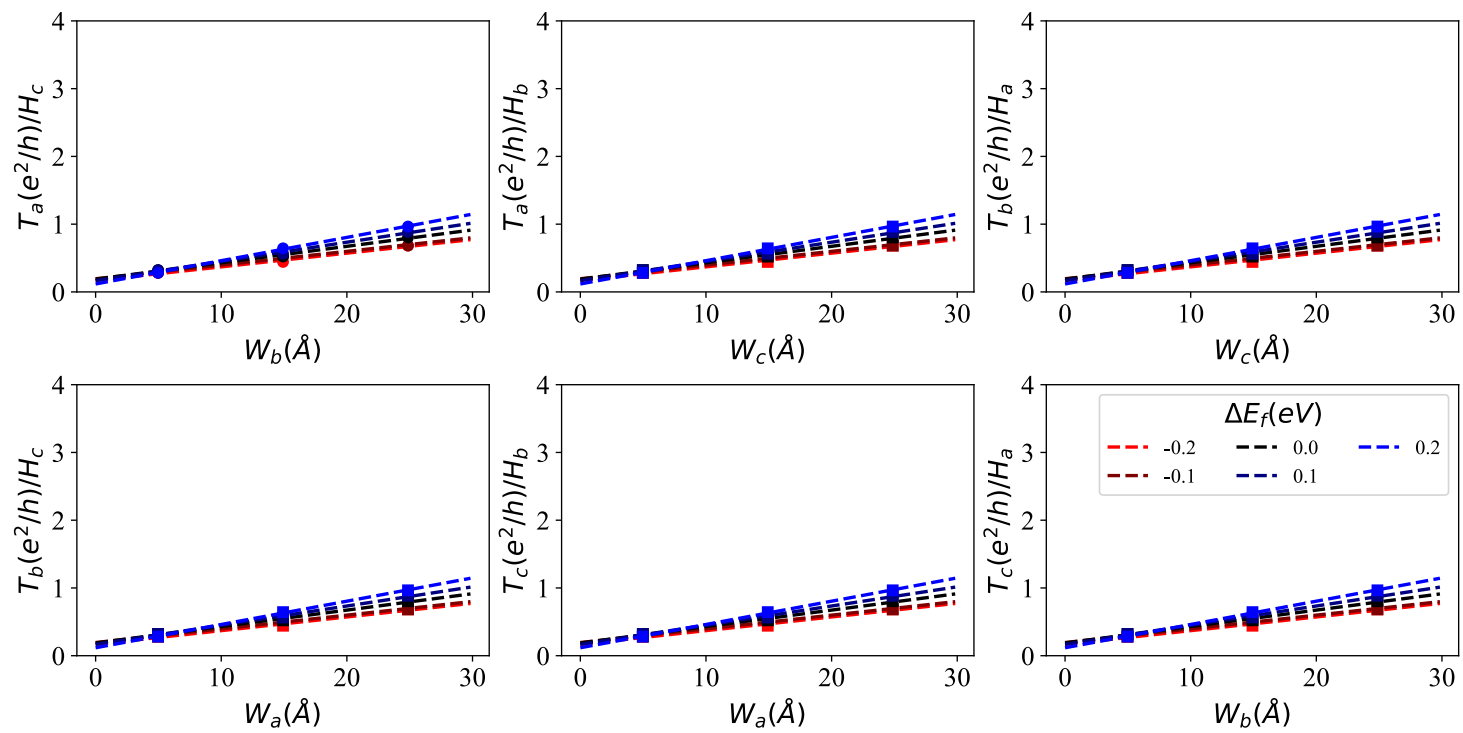

Compound: GaGeTe  
Materials Project ID: 8211

Lattice (conventional cell):

| Parameter        | Value    | Unit |
|------------------|----------|------|
| a                | 4.1264   | Å    |
| b                | 4.1264   | Å    |
| c                | 36.5601  | Å    |
| $\alpha$ (alpha) | 90.0000  | °    |
| $\beta$ (beta)   | 90.0000  | °    |
| $\gamma$ (gamma) | 120.0000 | °    |

Crystal structure (conventional cell):

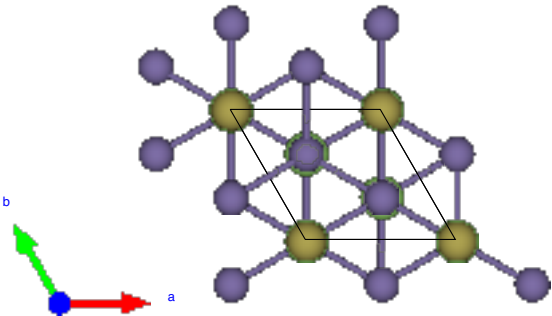

Nanowire Transmission:

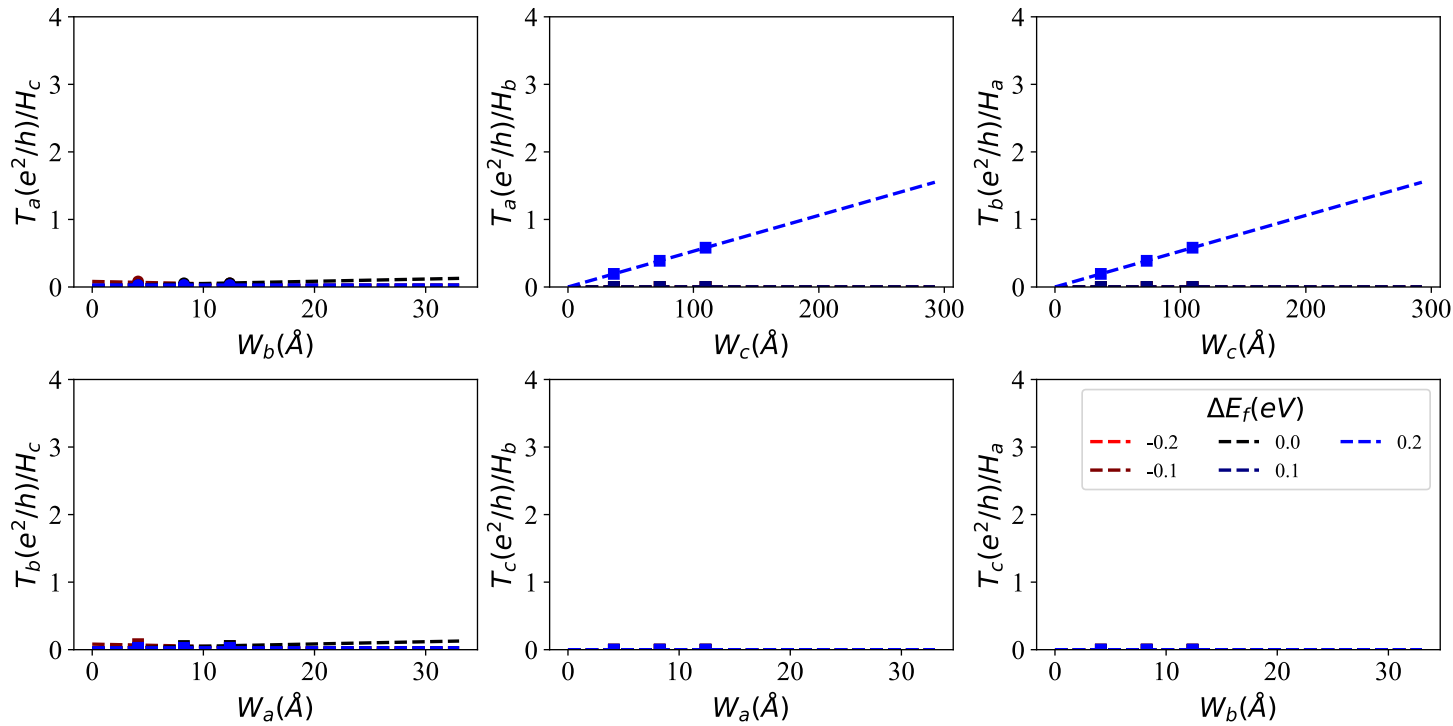

Compound: GeRh  
Materials Project ID: 20866

Lattice (conventional cell):

| Parameter        | Value   | Unit |
|------------------|---------|------|
| a                | 4.8620  | Å    |
| b                | 4.8620  | Å    |
| c                | 4.8620  | Å    |
| $\alpha$ (alpha) | 90.0000 | °    |
| $\beta$ (beta)   | 90.0000 | °    |
| $\gamma$ (gamma) | 90.0000 | °    |

Crystal structure (conventional cell):

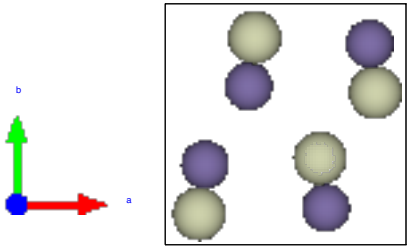

Nanowire Transmission:

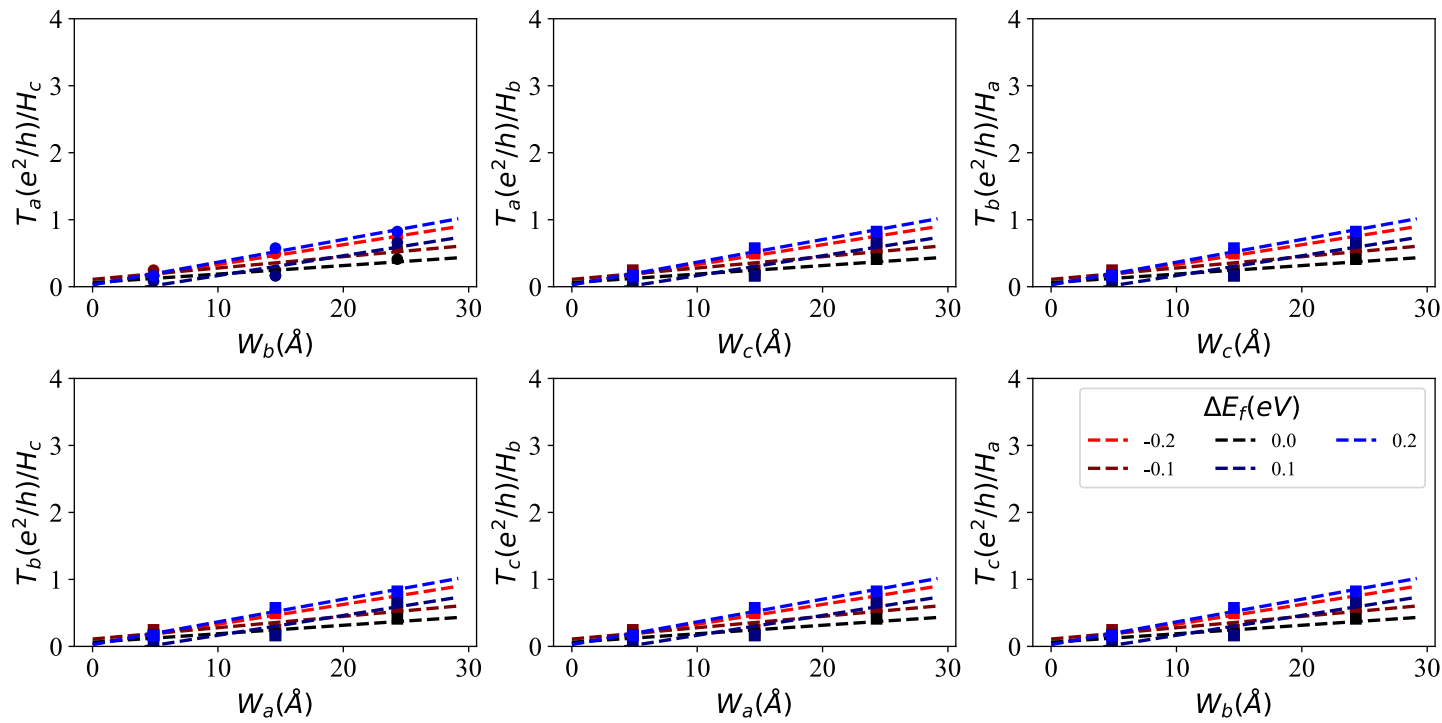

Compound:  $\text{HfB}_2$   
Materials Project ID: 1994

Lattice (conventional cell):

| Parameter        | Value    | Unit |
|------------------|----------|------|
| a                | 3.1487   | Å    |
| b                | 3.1487   | Å    |
| c                | 3.4799   | Å    |
| $\alpha$ (alpha) | 90.0000  | °    |
| $\beta$ (beta)   | 90.0000  | °    |
| $\gamma$ (gamma) | 120.0000 | °    |

Crystal structure (conventional cell):

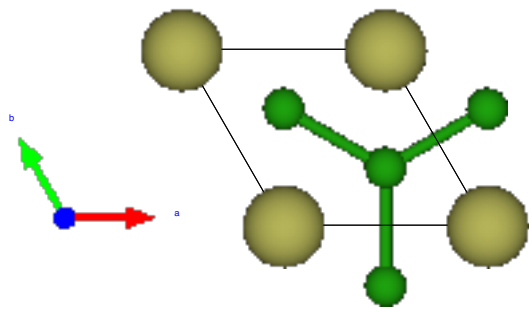

Nanowire Transmission:

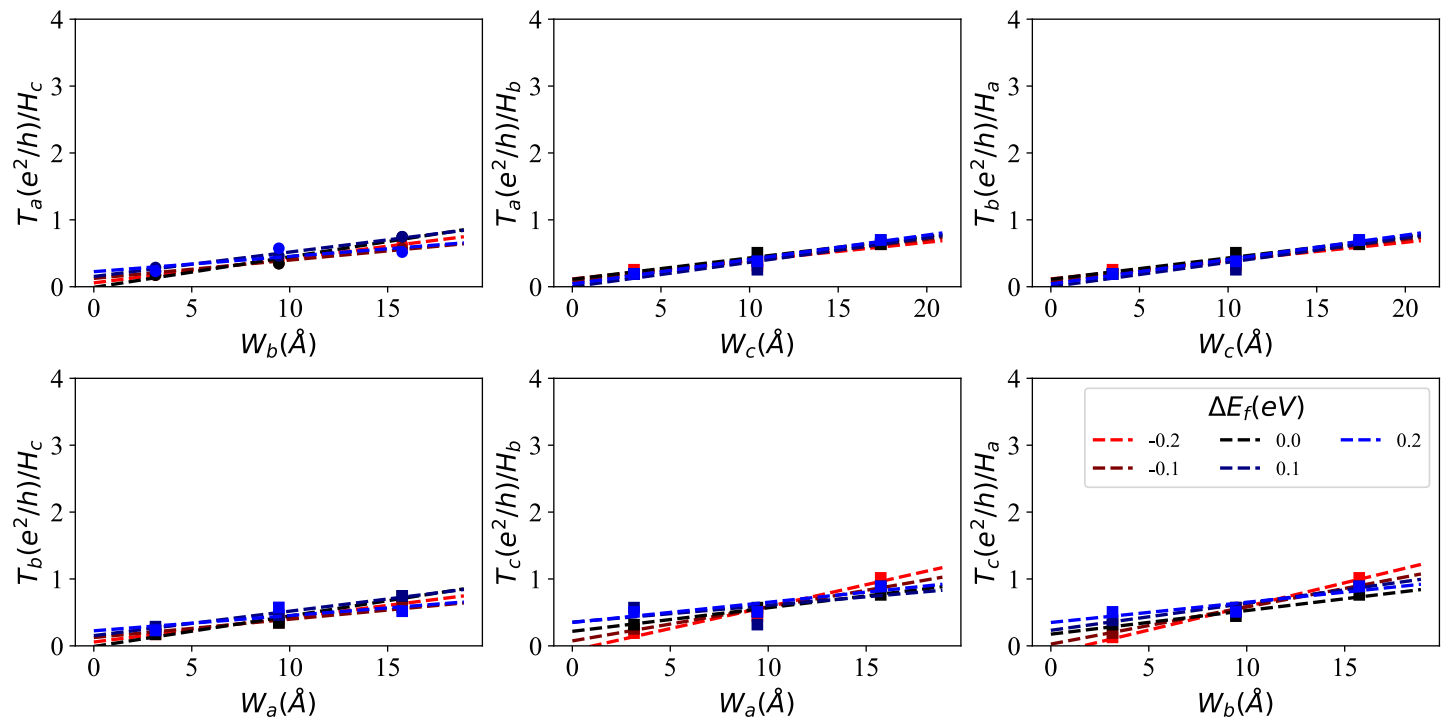

Compound: HfCuP  
Materials Project ID: 569933

Lattice (conventional cell):

| Parameter        | Value    | Unit |
|------------------|----------|------|
| a                | 3.5872   | Å    |
| b                | 3.5872   | Å    |
| c                | 5.5801   | Å    |
| $\alpha$ (alpha) | 90.0000  | °    |
| $\beta$ (beta)   | 90.0000  | °    |
| $\gamma$ (gamma) | 120.0000 | °    |

Crystal structure (conventional cell):

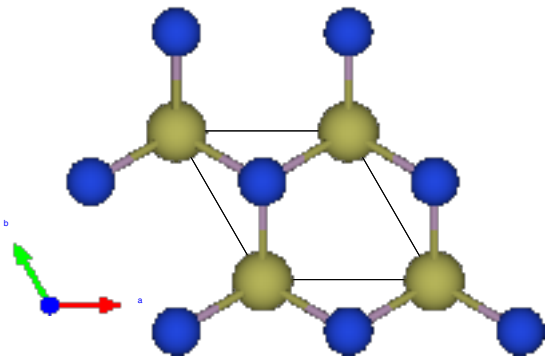

Nanowire Transmission:

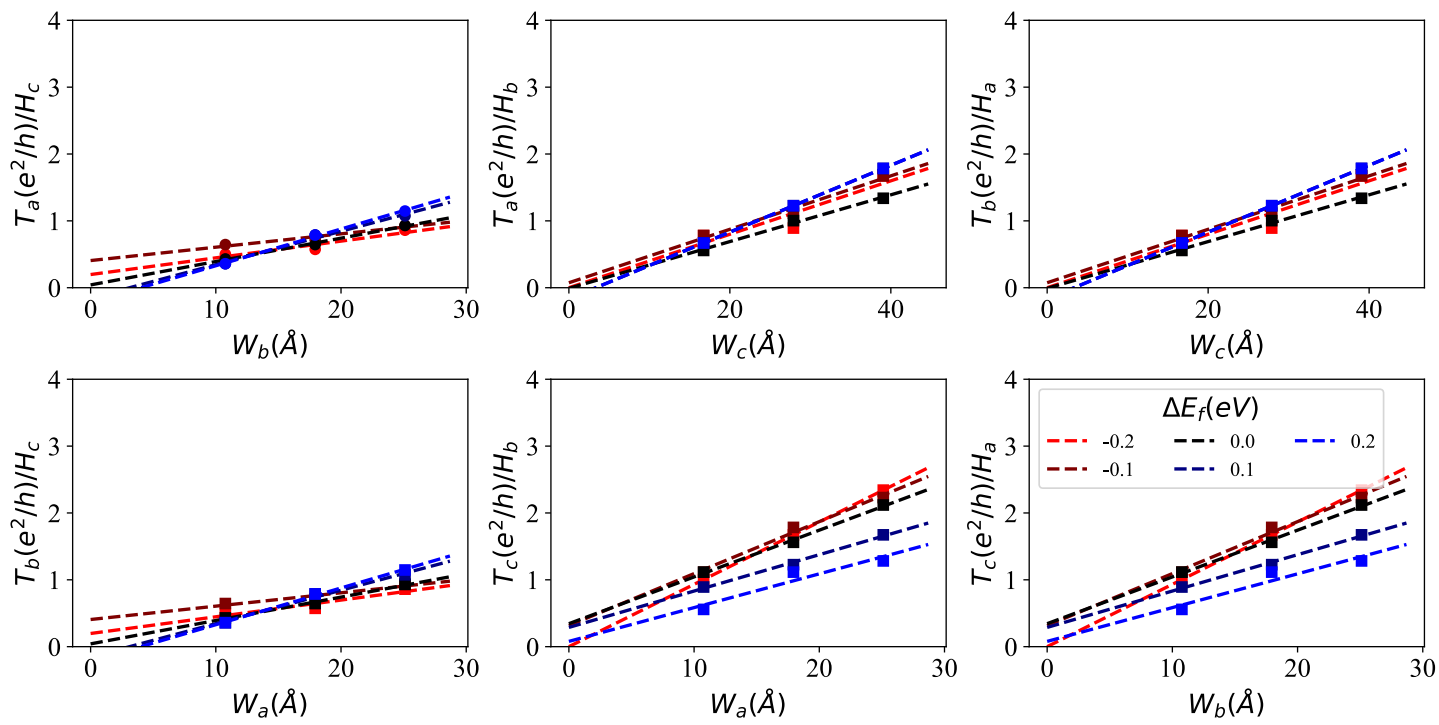

Compound: InGaSe<sub>2</sub>  
Materials Project ID: 1095059

Lattice (conventional cell):

| Parameter        | Value   | Unit |
|------------------|---------|------|
| a                | 8.1411  | Å    |
| b                | 8.1411  | Å    |
| c                | 6.4253  | Å    |
| $\alpha$ (alpha) | 90.0000 | °    |
| $\beta$ (beta)   | 90.0000 | °    |
| $\gamma$ (gamma) | 90.0000 | °    |

Crystal structure (conventional cell):

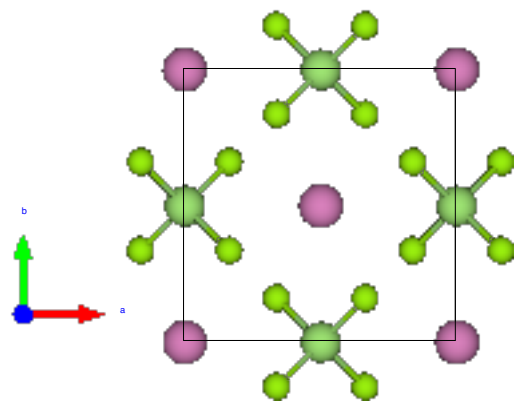

Nanowire Transmission:

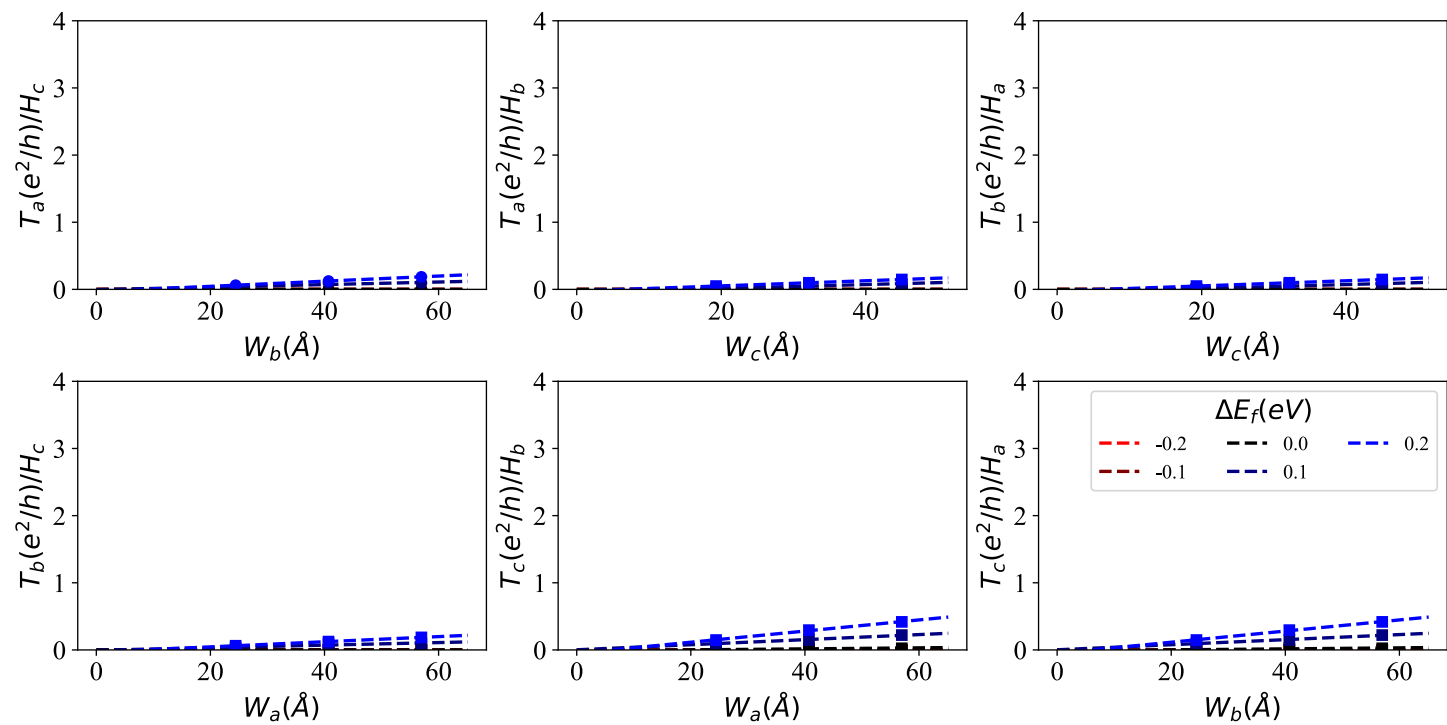



Compound: InTe  
Materials Project ID: 20320

Lattice (conventional cell):

| Parameter        | Value   | Unit |
|------------------|---------|------|
| a                | 8.6274  | Å    |
| b                | 8.6274  | Å    |
| c                | 7.2267  | Å    |
| $\alpha$ (alpha) | 90.0000 | °    |
| $\beta$ (beta)   | 90.0000 | °    |
| $\gamma$ (gamma) | 90.0000 | °    |

Crystal structure (conventional cell):

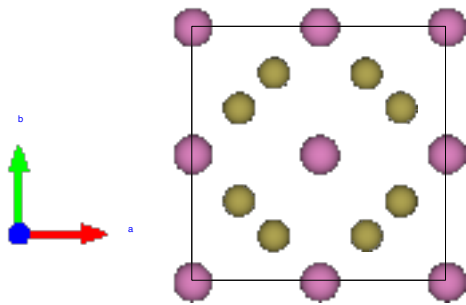

Nanowire Transmission:

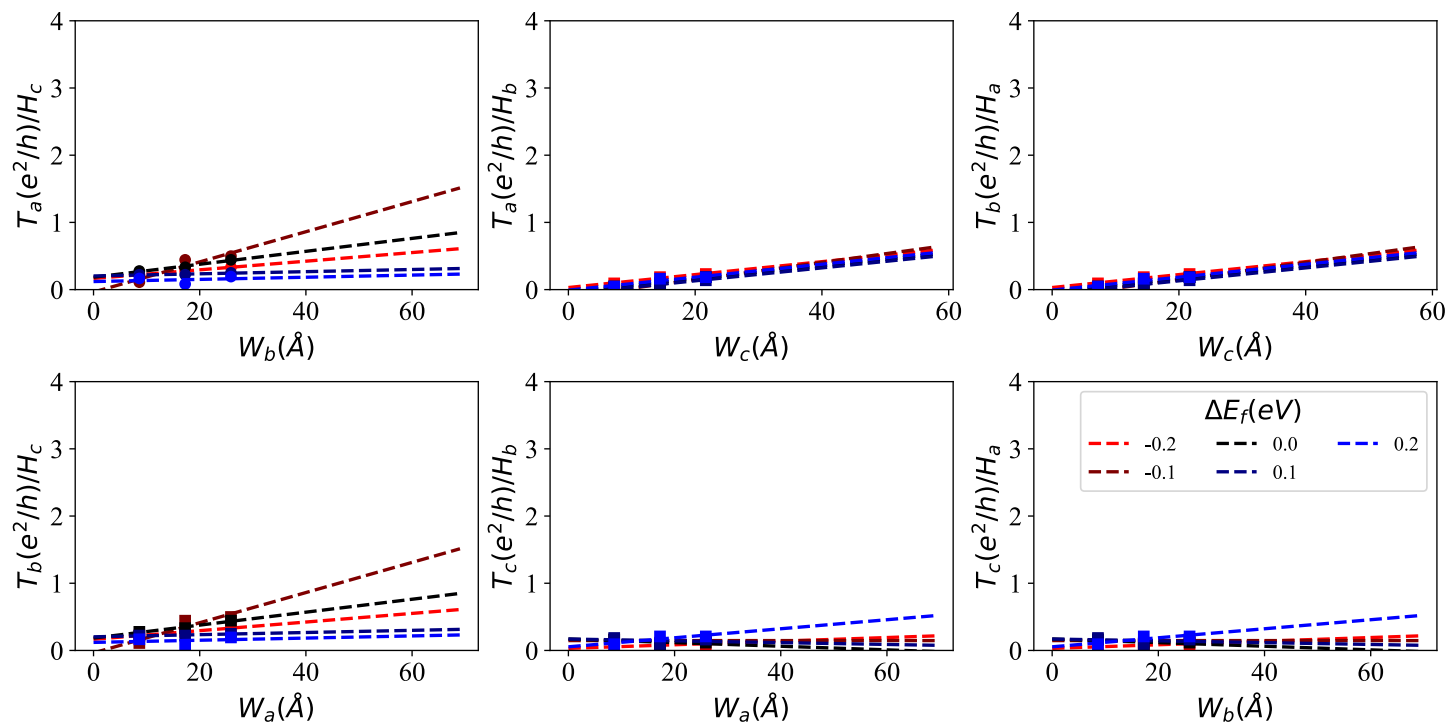

Compound: Ir  
Materials Project ID: 101

Lattice (conventional cell):

| Parameter        | Value   | Unit |
|------------------|---------|------|
| a                | 3.8757  | Å    |
| b                | 3.8757  | Å    |
| c                | 3.8757  | Å    |
| $\alpha$ (alpha) | 90.0000 | °    |
| $\beta$ (beta)   | 90.0000 | °    |
| $\gamma$ (gamma) | 90.0000 | °    |

Crystal structure (conventional cell):

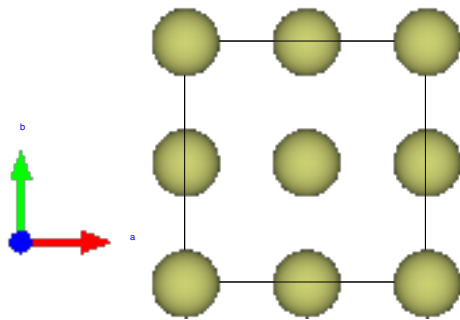

Nanowire Transmission:

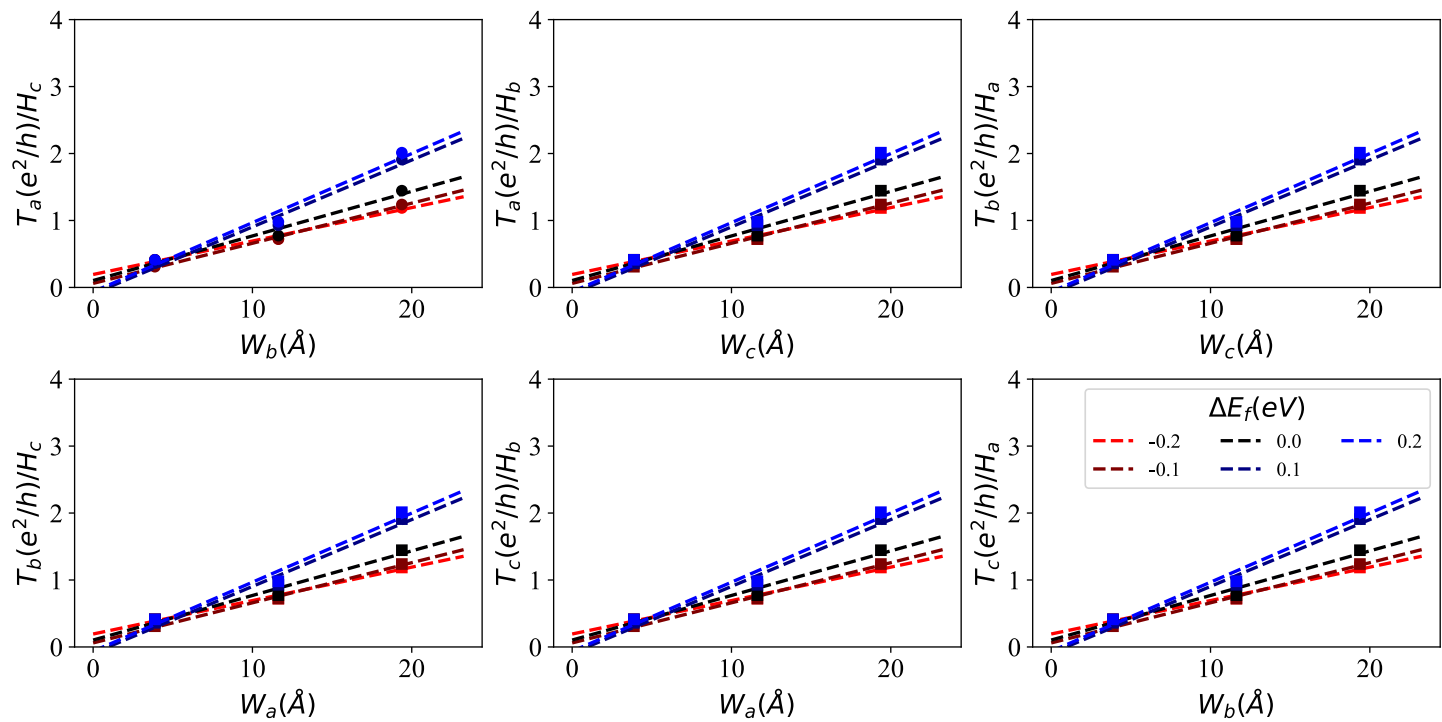

Compound: LaBiPt  
Materials Project ID: 1018136

Lattice (conventional cell):

| Parameter        | Value   | Unit |
|------------------|---------|------|
| a                | 6.9689  | Å    |
| b                | 6.9689  | Å    |
| c                | 6.9689  | Å    |
| $\alpha$ (alpha) | 90.0000 | °    |
| $\beta$ (beta)   | 90.0000 | °    |
| $\gamma$ (gamma) | 90.0000 | °    |

Crystal structure (conventional cell):

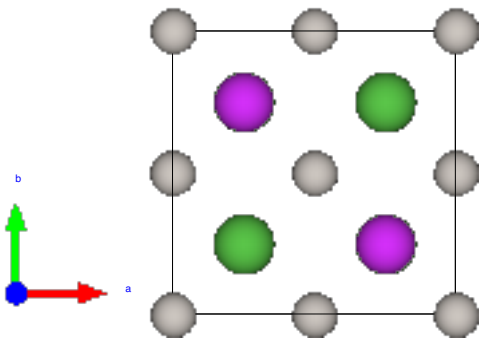

Nanowire Transmission:

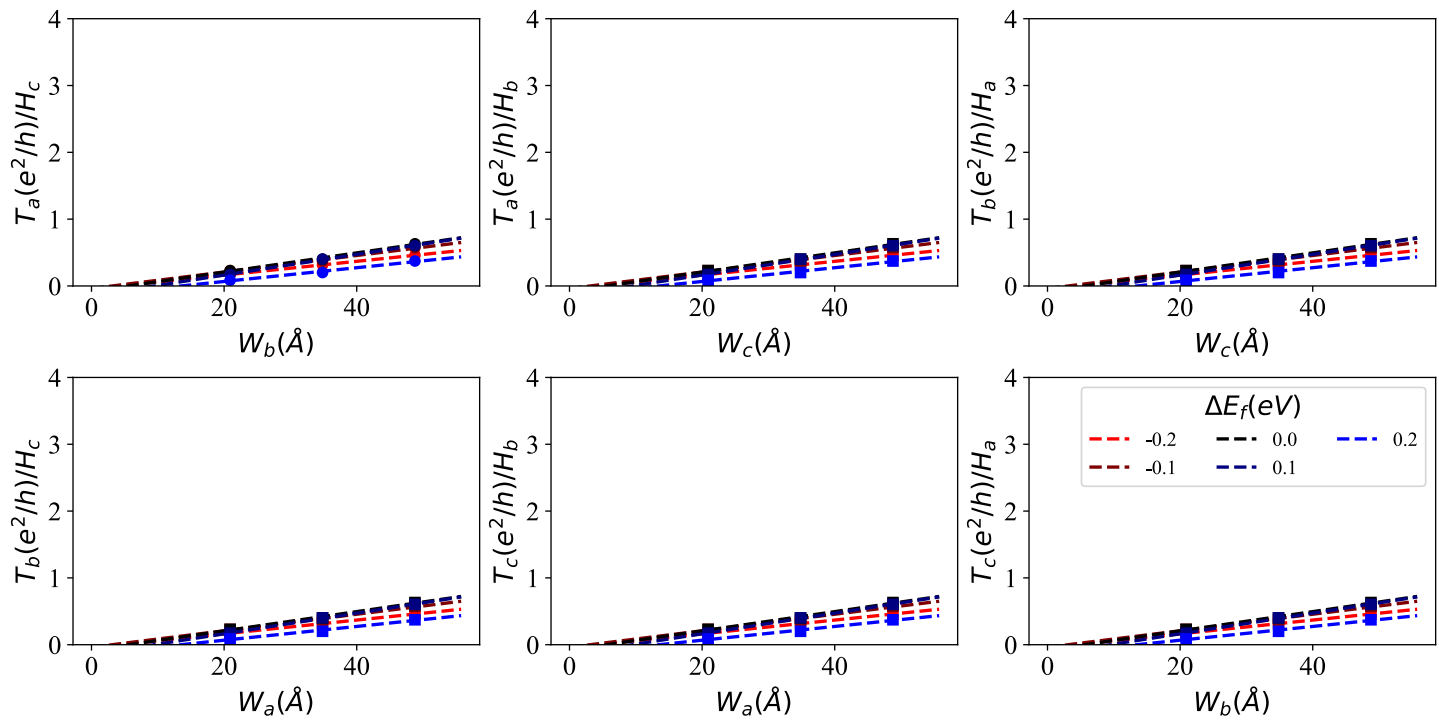

Compound: LaPIr  
Materials Project ID: 12919

Lattice (conventional cell):

| Parameter        | Value   | Unit |
|------------------|---------|------|
| a                | 4.1709  | Å    |
| b                | 4.1709  | Å    |
| c                | 14.3855 | Å    |
| $\alpha$ (alpha) | 90.0000 | °    |
| $\beta$ (beta)   | 90.0000 | °    |
| $\gamma$ (gamma) | 90.0000 | °    |

Crystal structure (conventional cell):

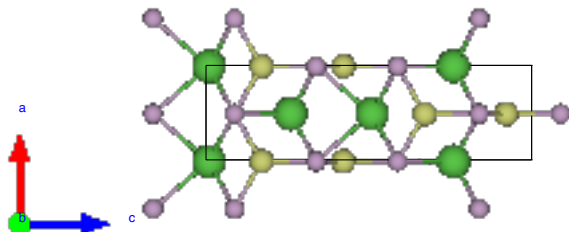

Nanowire Transmission:

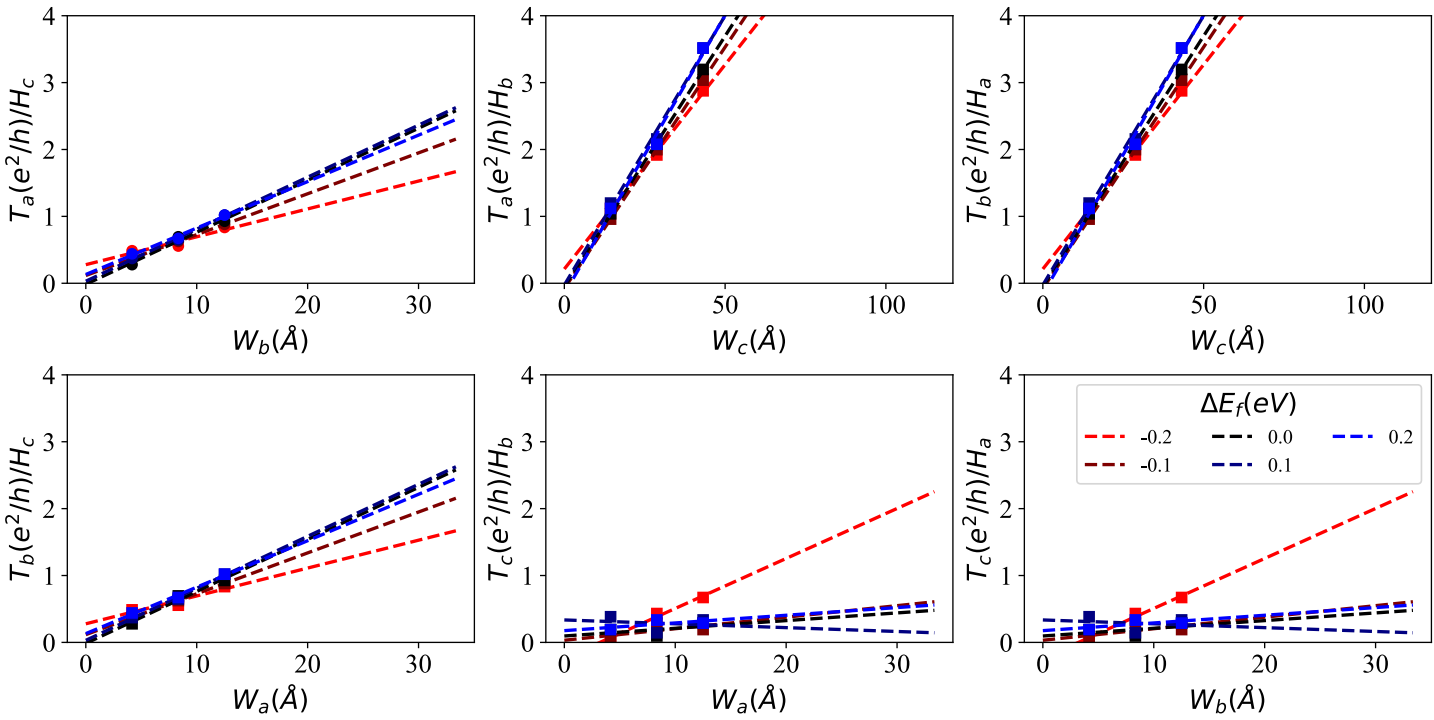

Compound: LiClO2  
Materials Project ID: 31367

Lattice (conventional cell):

| Parameter        | Value   | Unit |
|------------------|---------|------|
| a                | 4.8313  | Å    |
| b                | 4.8313  | Å    |
| c                | 10.6884 | Å    |
| $\alpha$ (alpha) | 90.0000 | °    |
| $\beta$ (beta)   | 90.0000 | °    |
| $\gamma$ (gamma) | 90.0000 | °    |

Crystal structure (conventional cell):

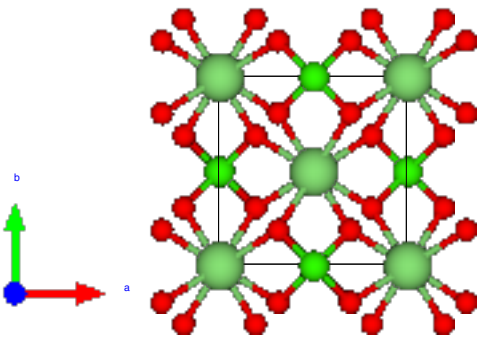

Nanowire Transmission:

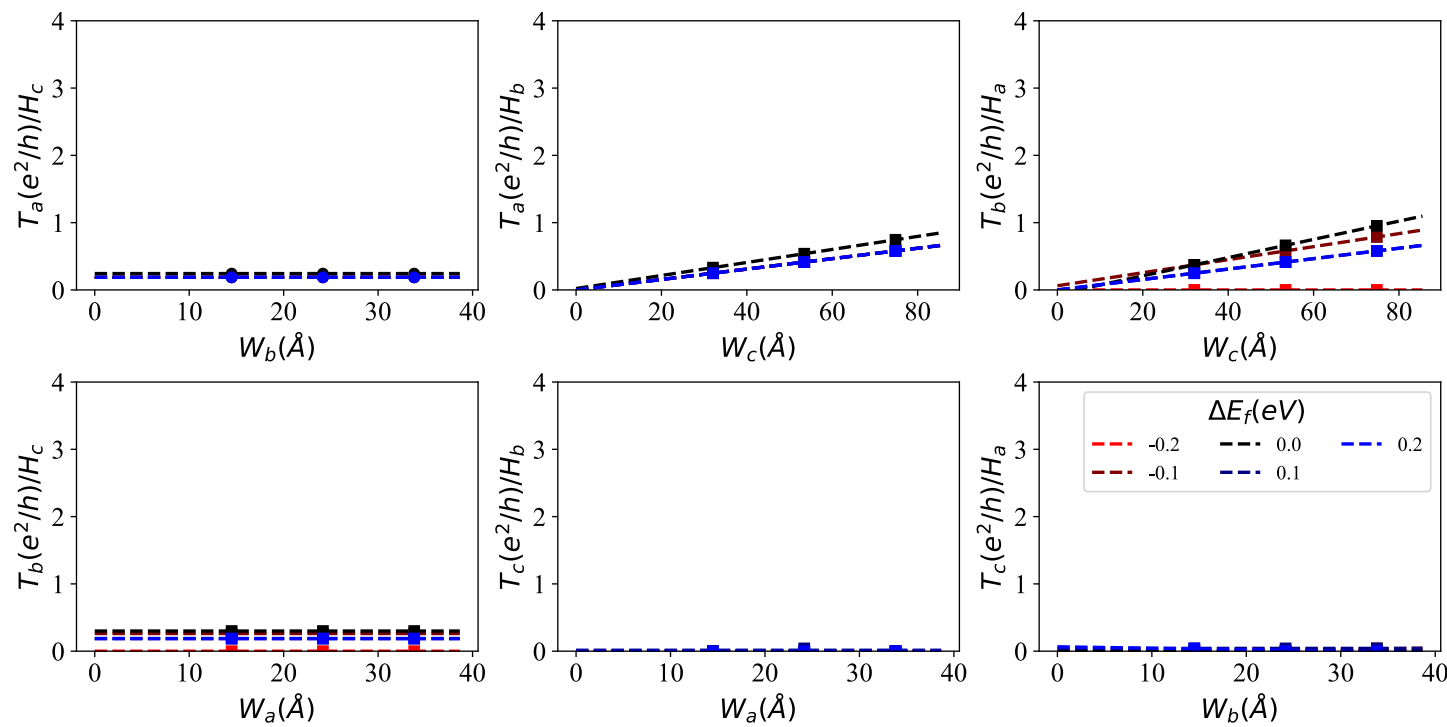

Compound: LiHO  
Materials Project ID: 23856

Lattice (conventional cell):

| Parameter        | Value   | Unit |
|------------------|---------|------|
| a                | 3.5914  | Å    |
| b                | 3.5914  | Å    |
| c                | 4.4105  | Å    |
| $\alpha$ (alpha) | 90.0000 | °    |
| $\beta$ (beta)   | 90.0000 | °    |
| $\gamma$ (gamma) | 90.0000 | °    |

Crystal structure (conventional cell):

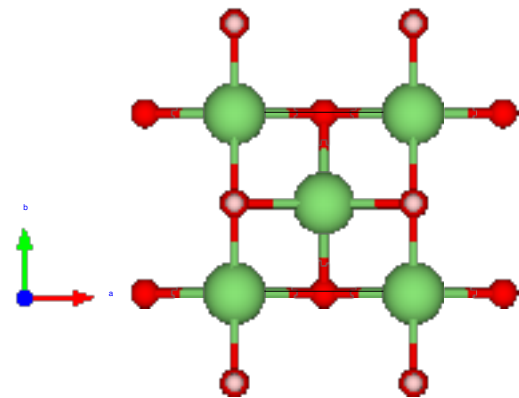

Nanowire Transmission:

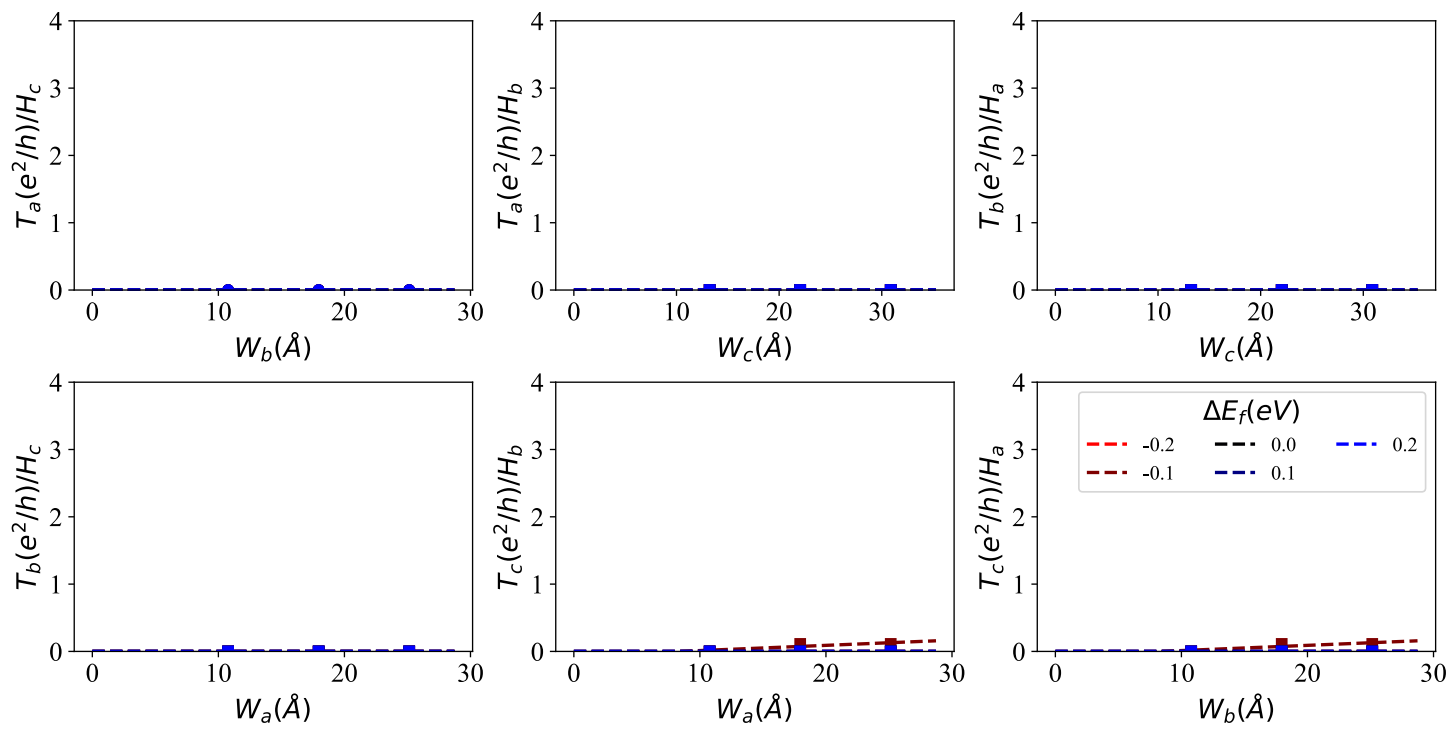

Compound: LiYGe  
Materials Project ID: 14209

Lattice (conventional cell):

| Parameter        | Value    | Unit |
|------------------|----------|------|
| a                | 7.0924   | Å    |
| b                | 7.0924   | Å    |
| c                | 4.2591   | Å    |
| $\alpha$ (alpha) | 90.0000  | °    |
| $\beta$ (beta)   | 90.0000  | °    |
| $\gamma$ (gamma) | 120.0000 | °    |

Crystal structure (conventional cell):

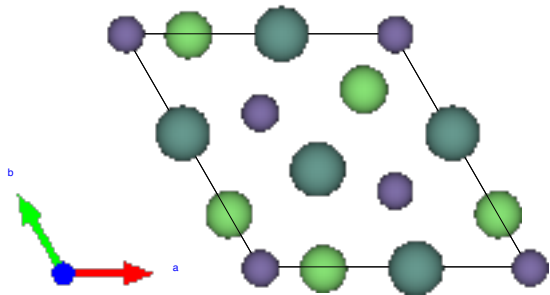

Nanowire Transmission:

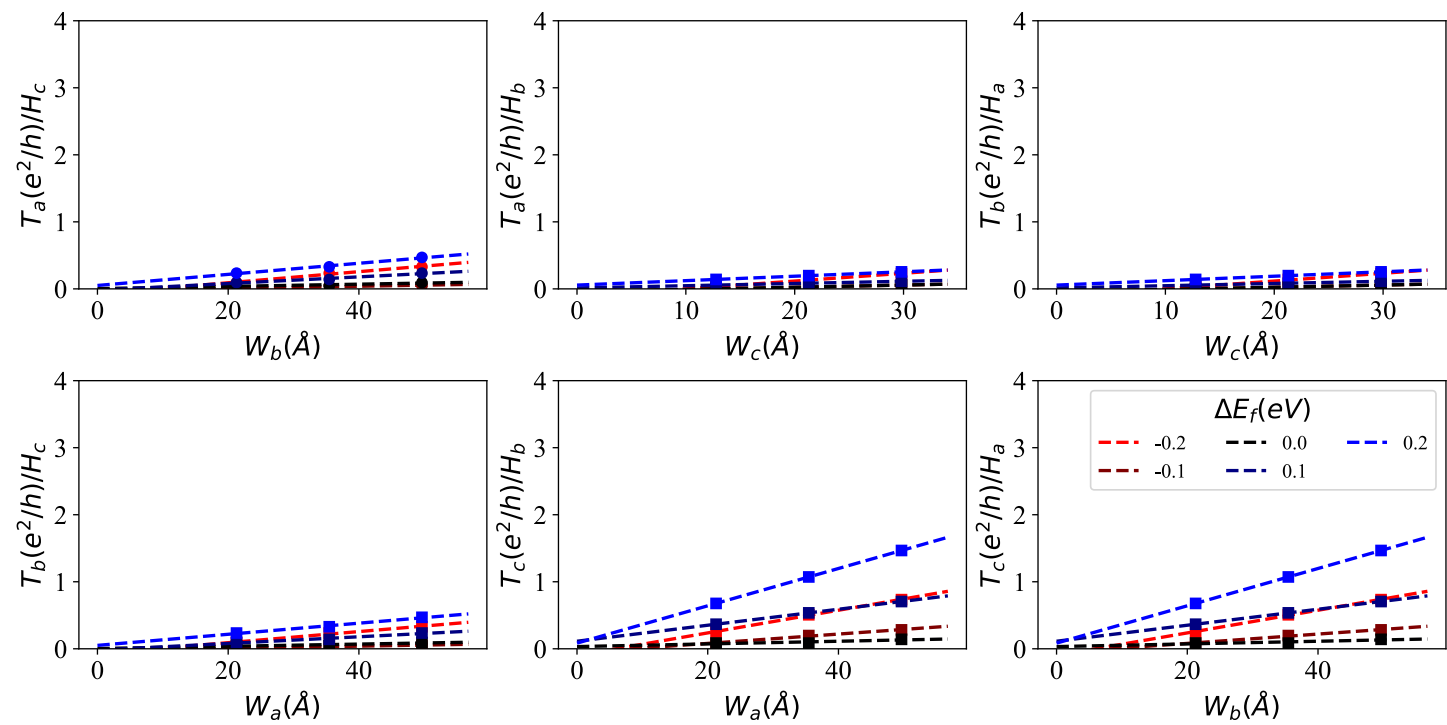

Compound: LiYSi

Materials Project ID: 14208

Lattice (conventional cell):

| Parameter        | Value    | Unit |
|------------------|----------|------|
| a                | 7.0152   | Å    |
| b                | 7.0152   | Å    |
| c                | 4.2400   | Å    |
| $\alpha$ (alpha) | 90.0000  | °    |
| $\beta$ (beta)   | 90.0000  | °    |
| $\gamma$ (gamma) | 120.0000 | °    |

Crystal structure (conventional cell):

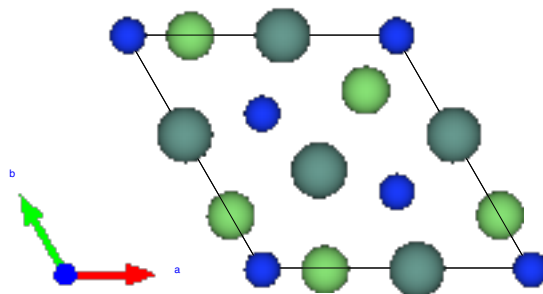

Nanowire Transmission:

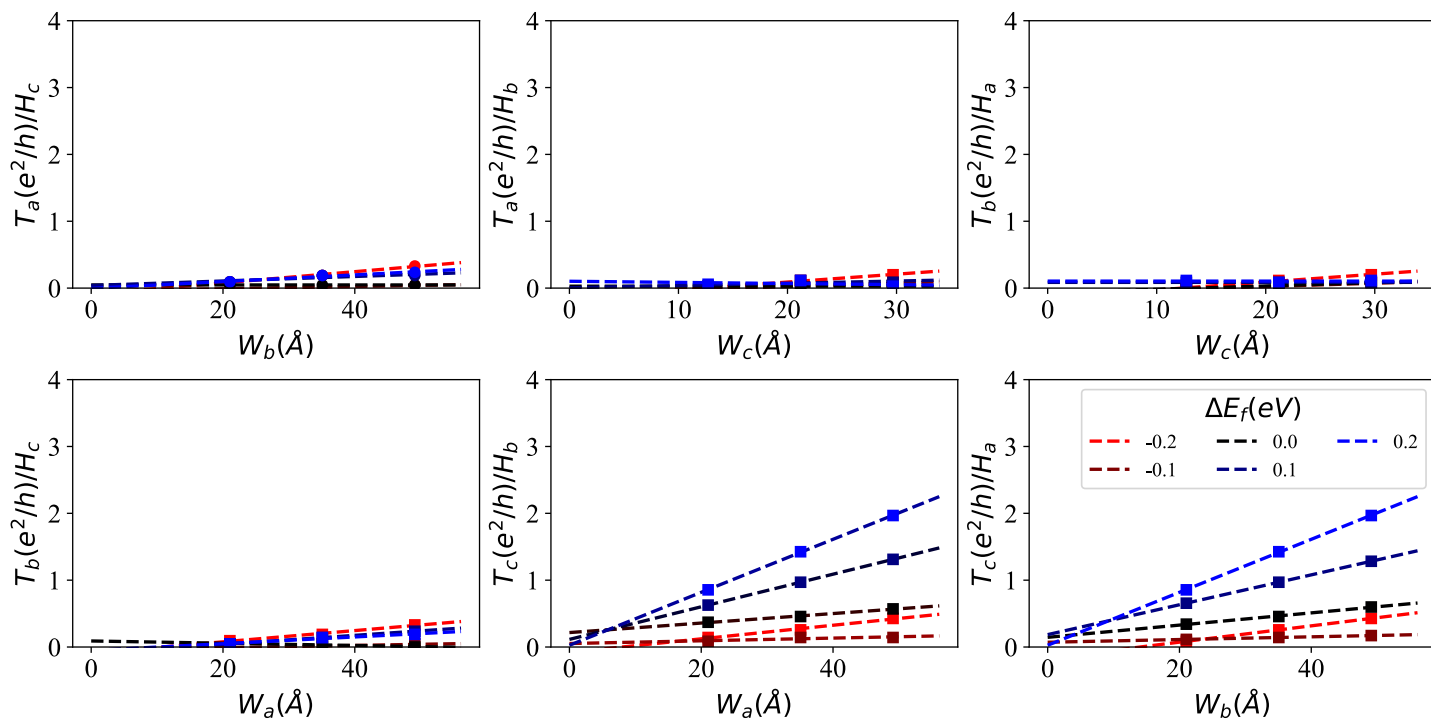



Compound: Mo  
Materials Project ID: 129

Lattice (conventional cell):

| Parameter        | Value   | Unit |
|------------------|---------|------|
| a                | 3.1676  | Å    |
| b                | 3.1676  | Å    |
| c                | 3.1676  | Å    |
| $\alpha$ (alpha) | 90.0000 | °    |
| $\beta$ (beta)   | 90.0000 | °    |
| $\gamma$ (gamma) | 90.0000 | °    |

Crystal structure (conventional cell):

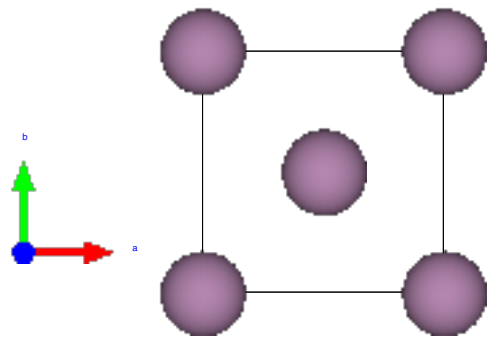

Nanowire Transmission:

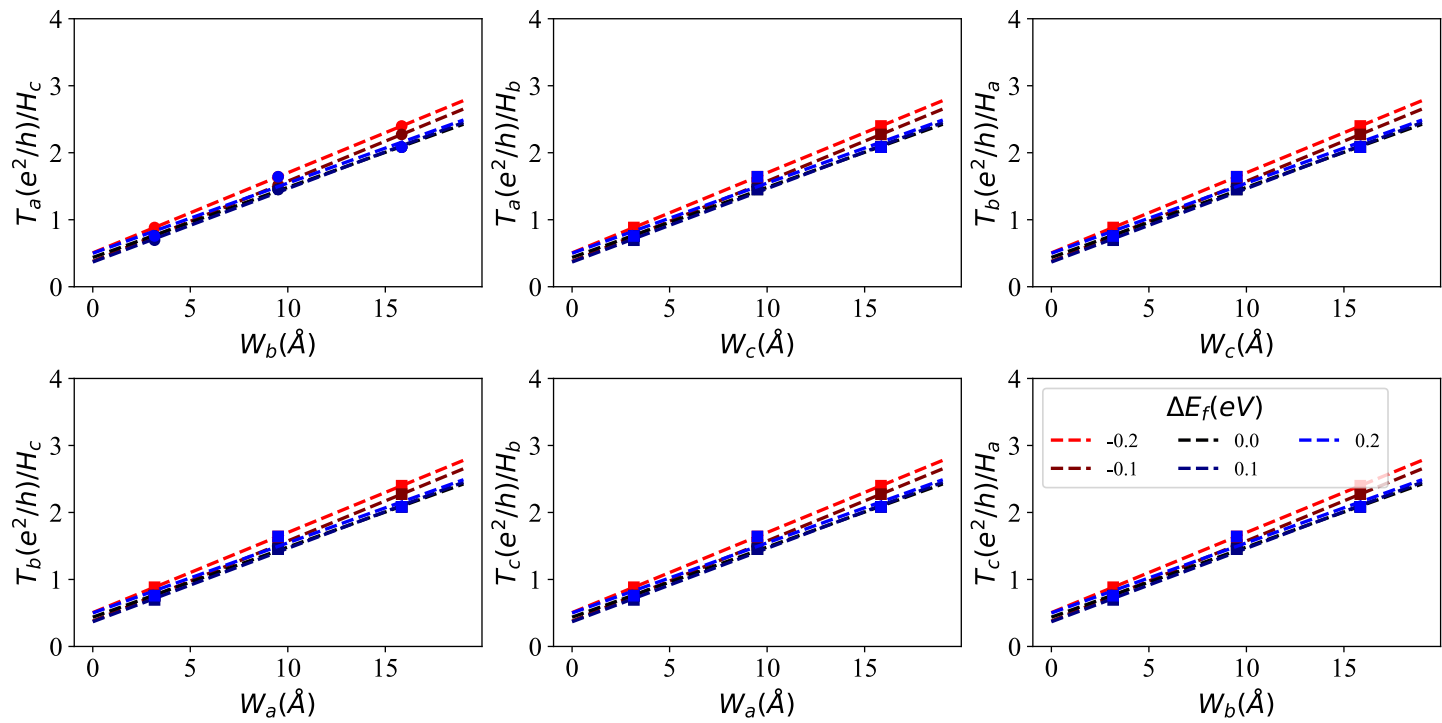

Compound: MoC  
Materials Project ID: 2305

Lattice (conventional cell):

| Parameter        | Value    | Unit |
|------------------|----------|------|
| a                | 2.9241   | Å    |
| b                | 2.9241   | Å    |
| c                | 2.8351   | Å    |
| $\alpha$ (alpha) | 90.0000  | °    |
| $\beta$ (beta)   | 90.0000  | °    |
| $\gamma$ (gamma) | 120.0000 | °    |

Crystal structure (conventional cell):

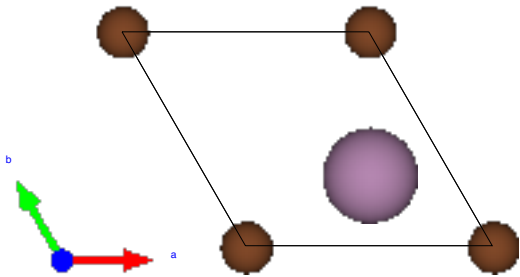

Nanowire Transmission:

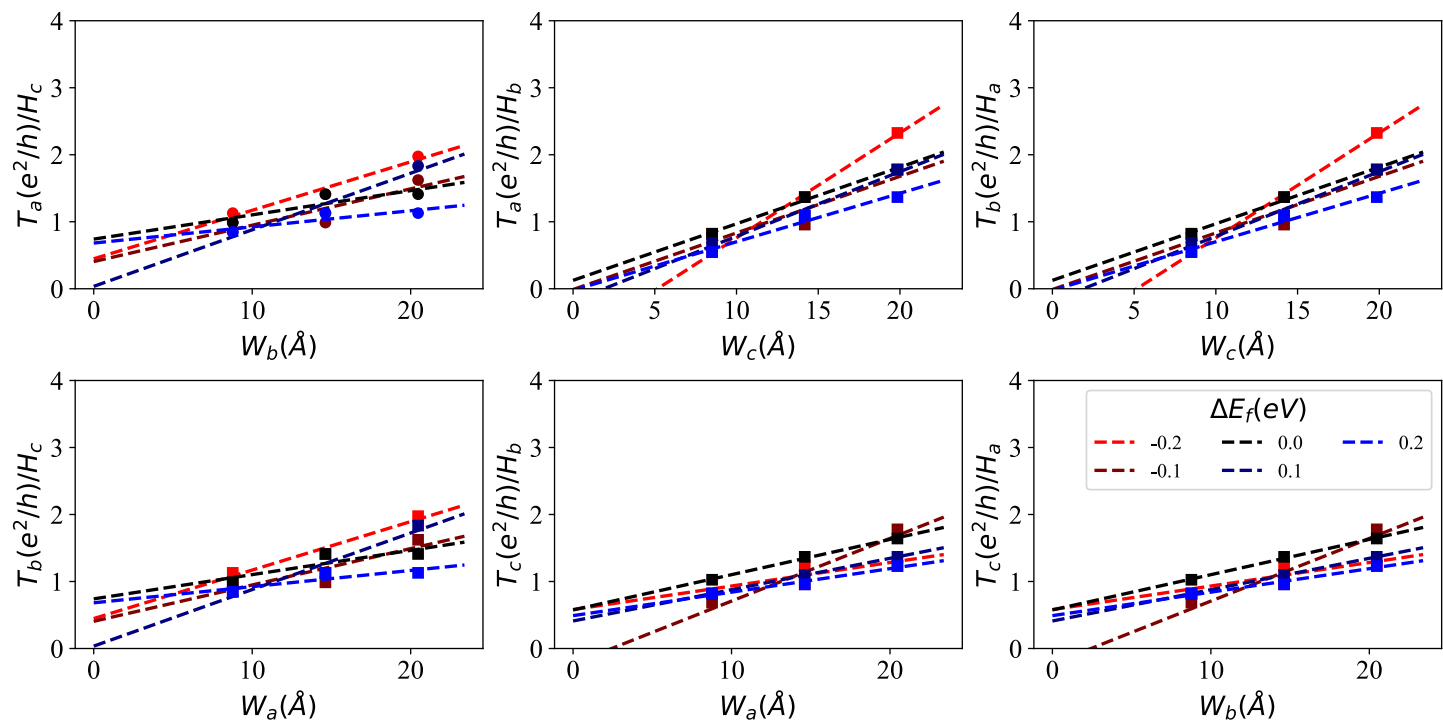

Materials Project ID: 13036

Lattice (conventional cell):

| Parameter        | Value    | Unit |
|------------------|----------|------|
| a                | 2.8858   | Å    |
| b                | 2.8858   | Å    |
| c                | 2.8561   | Å    |
| $\alpha$ (alpha) | 90.0000  | °    |
| $\beta$ (beta)   | 90.0000  | °    |
| $\gamma$ (gamma) | 120.0000 | °    |

Crystal structure (conventional cell):

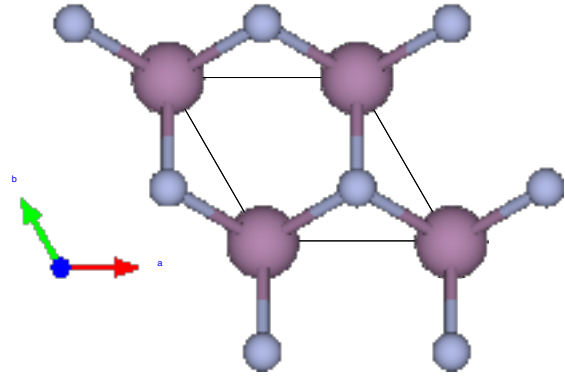

### Nanowire Transmission:

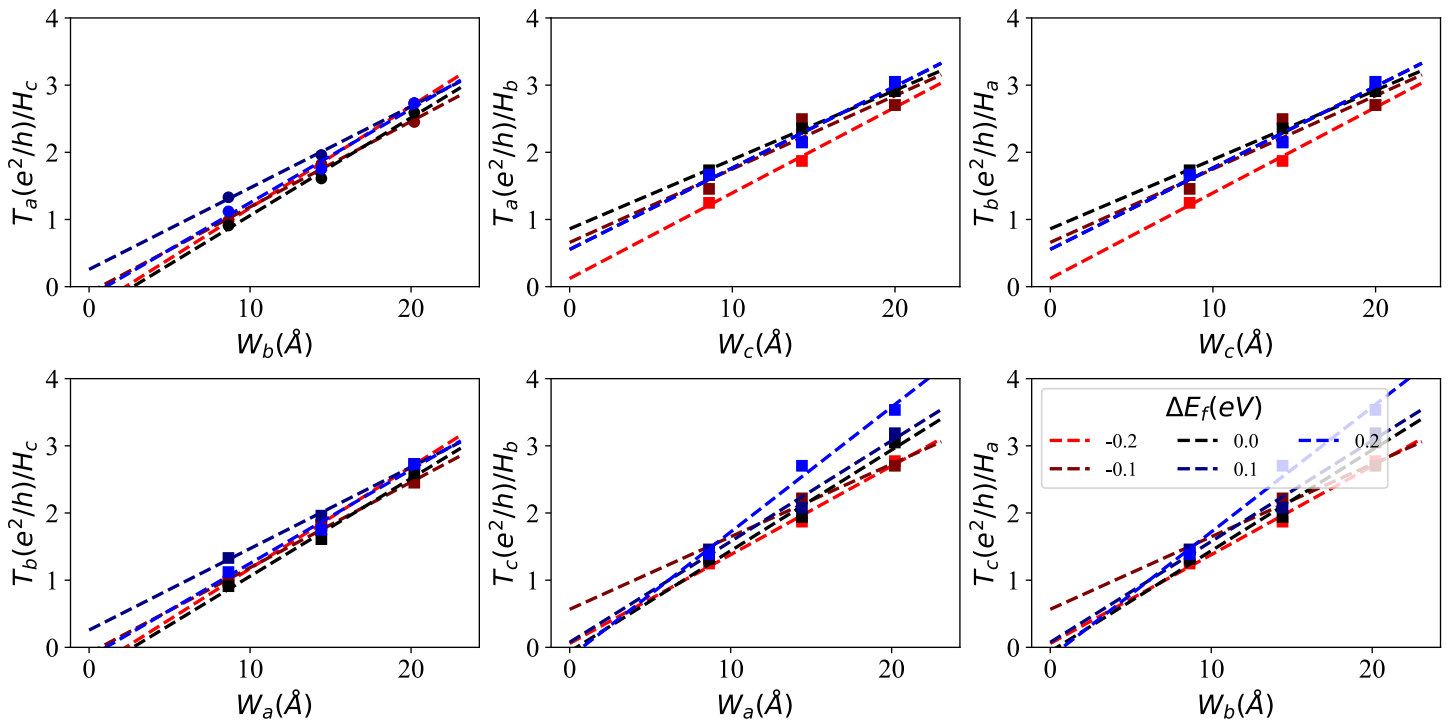

Compound: MoP  
Materials Project ID: 219

Lattice (conventional cell):

| Parameter        | Value    | Unit |
|------------------|----------|------|
| a                | 3.2446   | Å    |
| b                | 3.2446   | Å    |
| c                | 3.2005   | Å    |
| $\alpha$ (alpha) | 90.0000  | °    |
| $\beta$ (beta)   | 90.0000  | °    |
| $\gamma$ (gamma) | 120.0000 | °    |

Crystal structure (conventional cell):

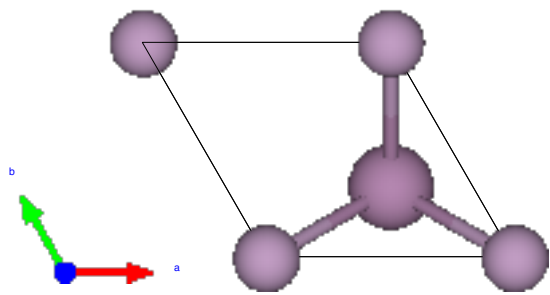

Nanowire Transmission:

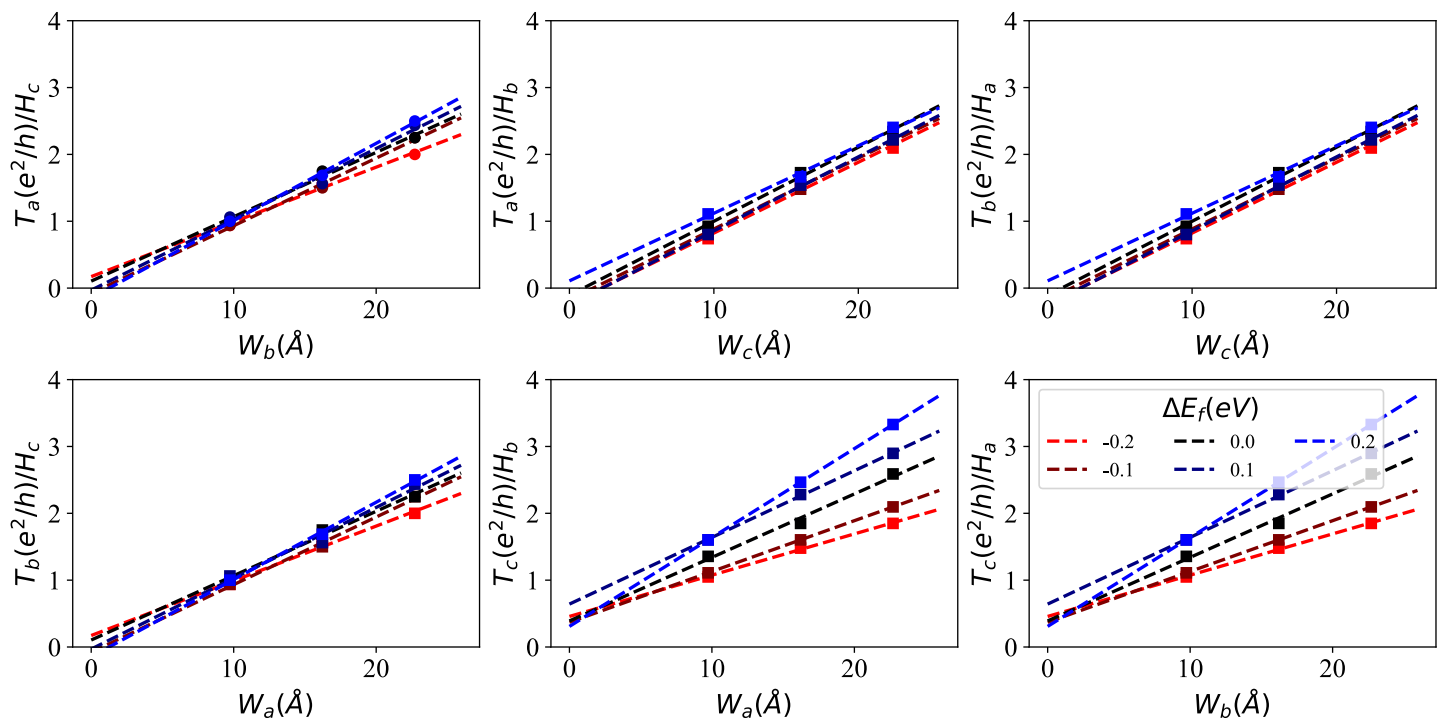

Compound: NbAs  
Materials Project ID: 2059

Lattice (conventional cell):

| Parameter        | Value   | Unit |
|------------------|---------|------|
| a                | 3.4847  | Å    |
| b                | 3.4847  | Å    |
| c                | 11.7615 | Å    |
| $\alpha$ (alpha) | 90.0000 | °    |
| $\beta$ (beta)   | 90.0000 | °    |
| $\gamma$ (gamma) | 90.0000 | °    |

Crystal structure (conventional cell):

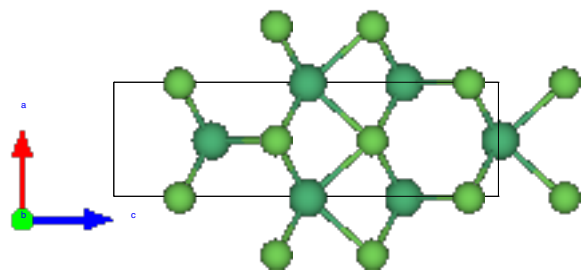

Nanowire Transmission:

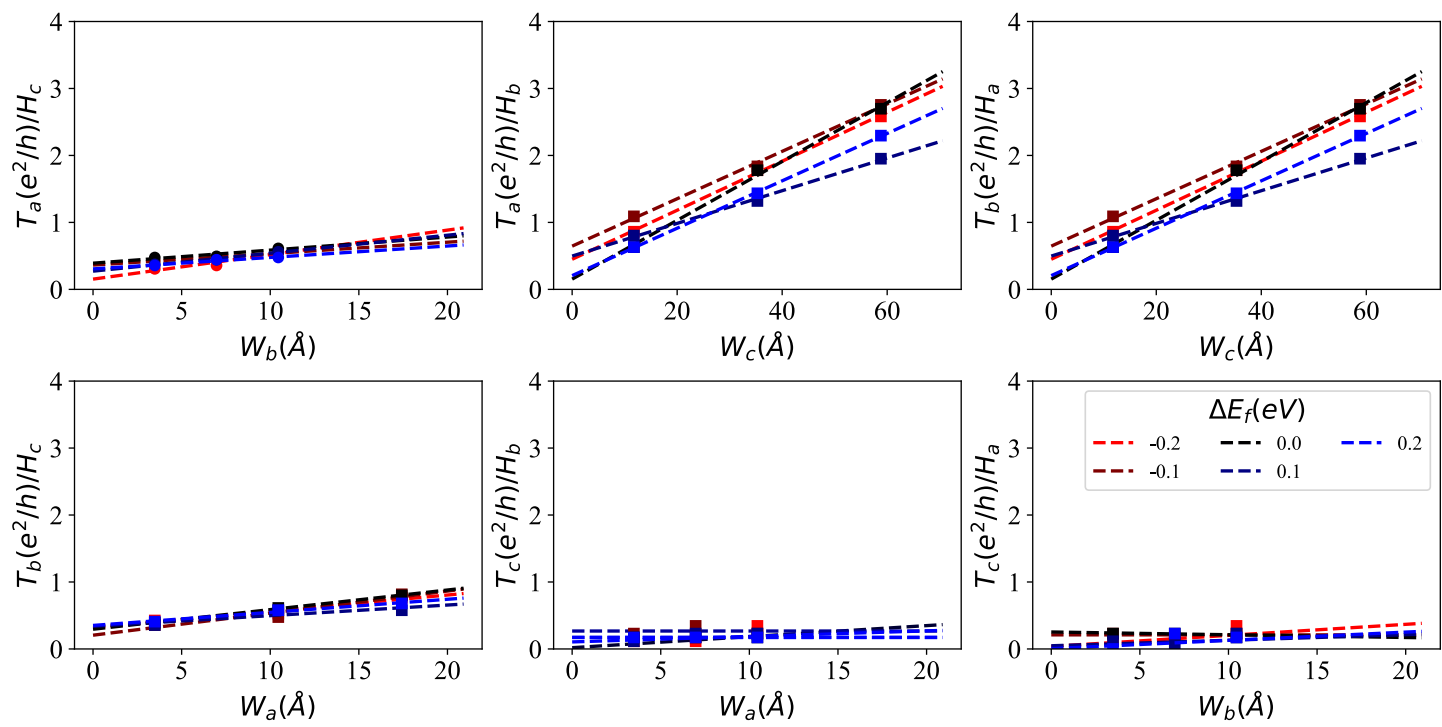

Compound: NbAs<sub>2</sub>  
Materials Project ID: 7598

Lattice (conventional cell):

| Parameter | Value    | Unit |
|-----------|----------|------|
| a         | 9.4518   | Å    |
| b         | 3.4178   | Å    |
| c         | 7.8850   | Å    |
| α (alpha) | 90.0000  | °    |
| β (beta)  | 119.3863 | °    |
| γ (gamma) | 90.0000  | °    |

Crystal structure (conventional cell):

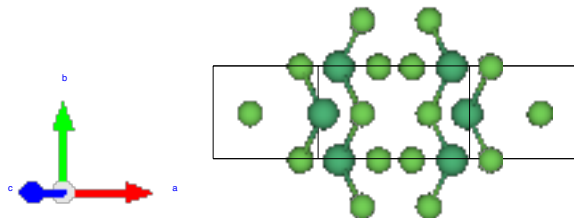

Nanowire Transmission:

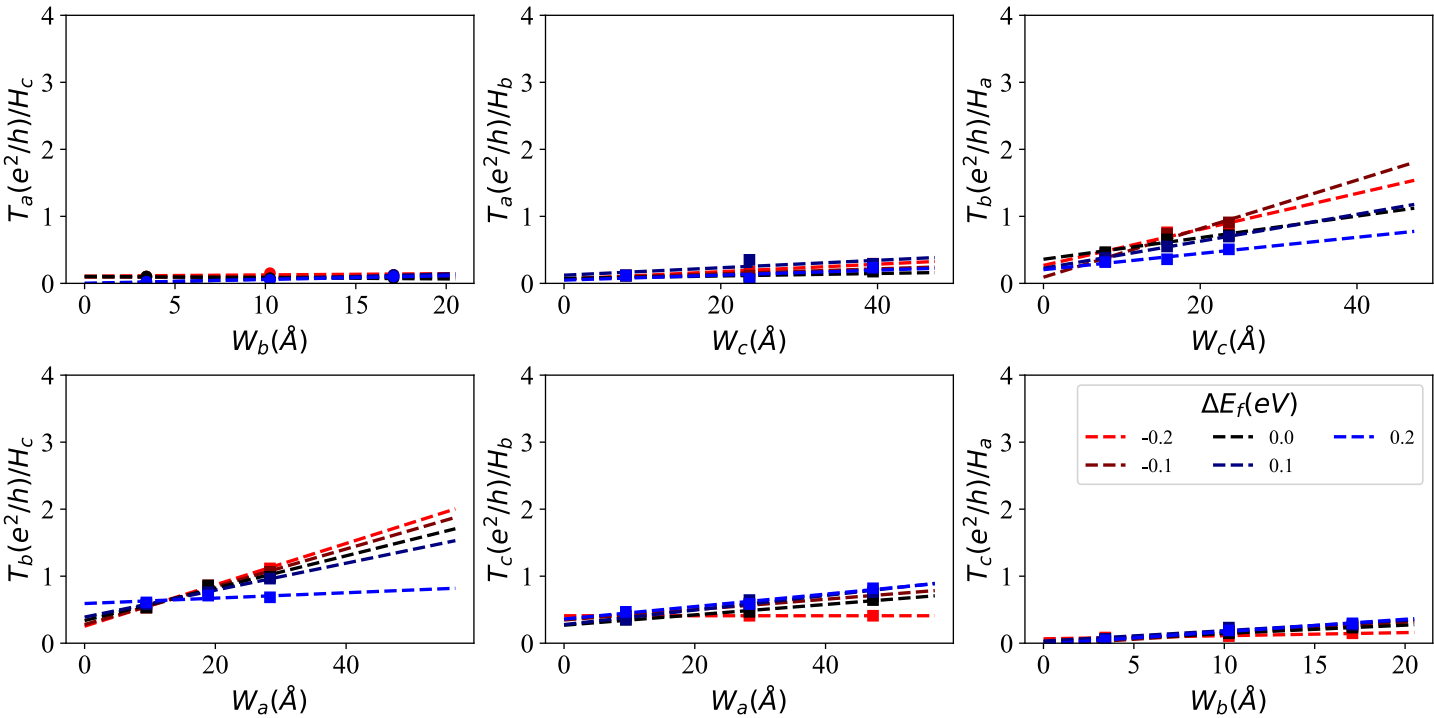

Compound: NbInSe<sub>2</sub>  
Materials Project ID: 20279

Lattice (conventional cell):

| Parameter | Value    | Unit |
|-----------|----------|------|
| a         | 3.4646   | Å    |
| b         | 3.4646   | Å    |
| c         | 9.3914   | Å    |
| α (alpha) | 90.0000  | °    |
| β (beta)  | 90.0000  | °    |
| γ (gamma) | 120.0000 | °    |

Crystal structure (conventional cell):

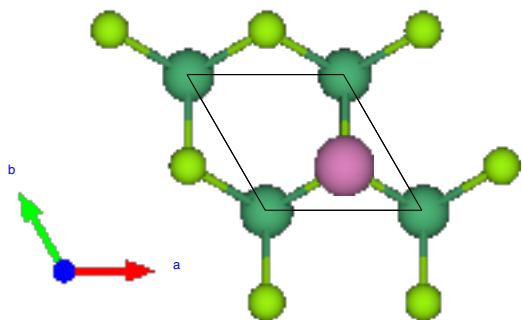

Nanowire Transmission:

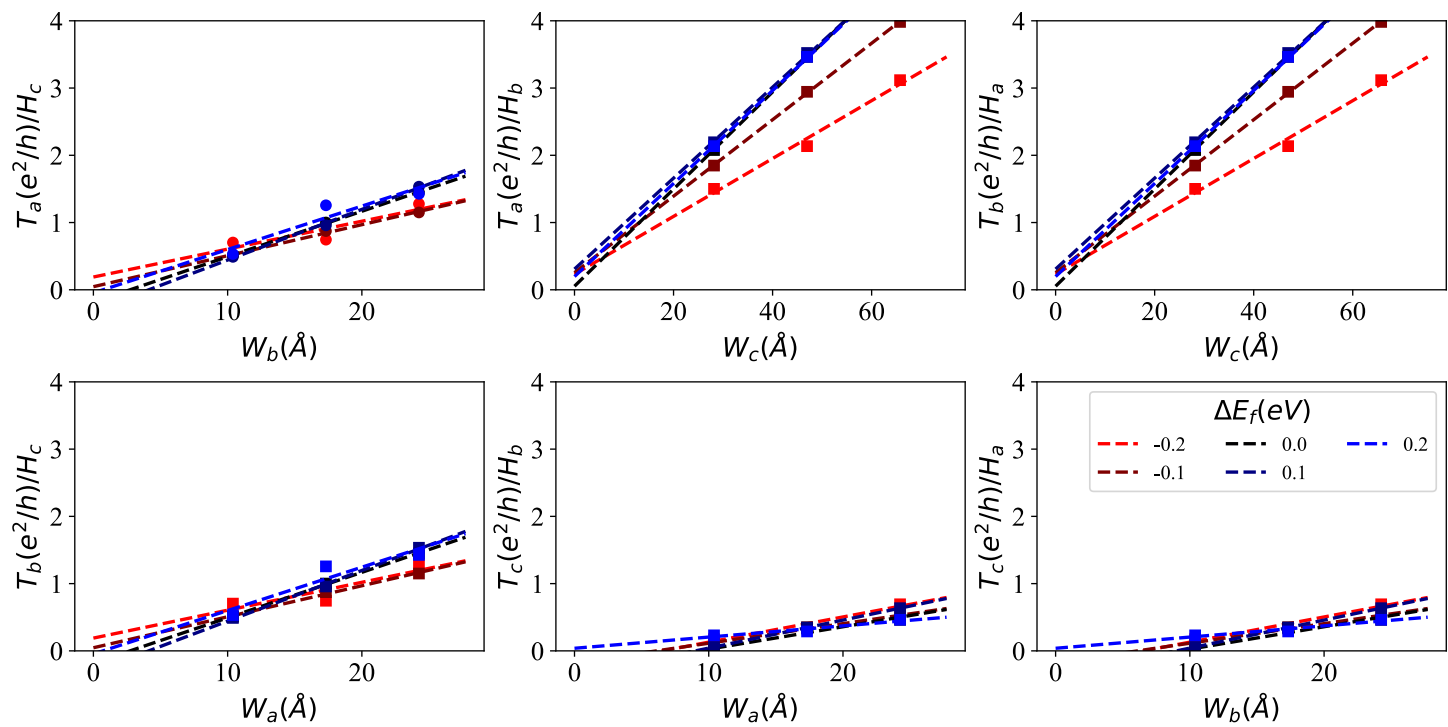

Compound: NbN  
Materials Project ID: 2634

Lattice (conventional cell):

| Parameter        | Value    | Unit |
|------------------|----------|------|
| a                | 2.9762   | Å    |
| b                | 2.9762   | Å    |
| c                | 2.8987   | Å    |
| $\alpha$ (alpha) | 90.0000  | °    |
| $\beta$ (beta)   | 90.0000  | °    |
| $\gamma$ (gamma) | 120.0000 | °    |

Crystal structure (conventional cell):

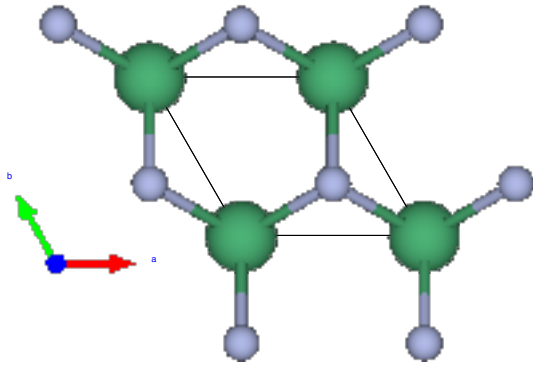

Nanowire Transmission:

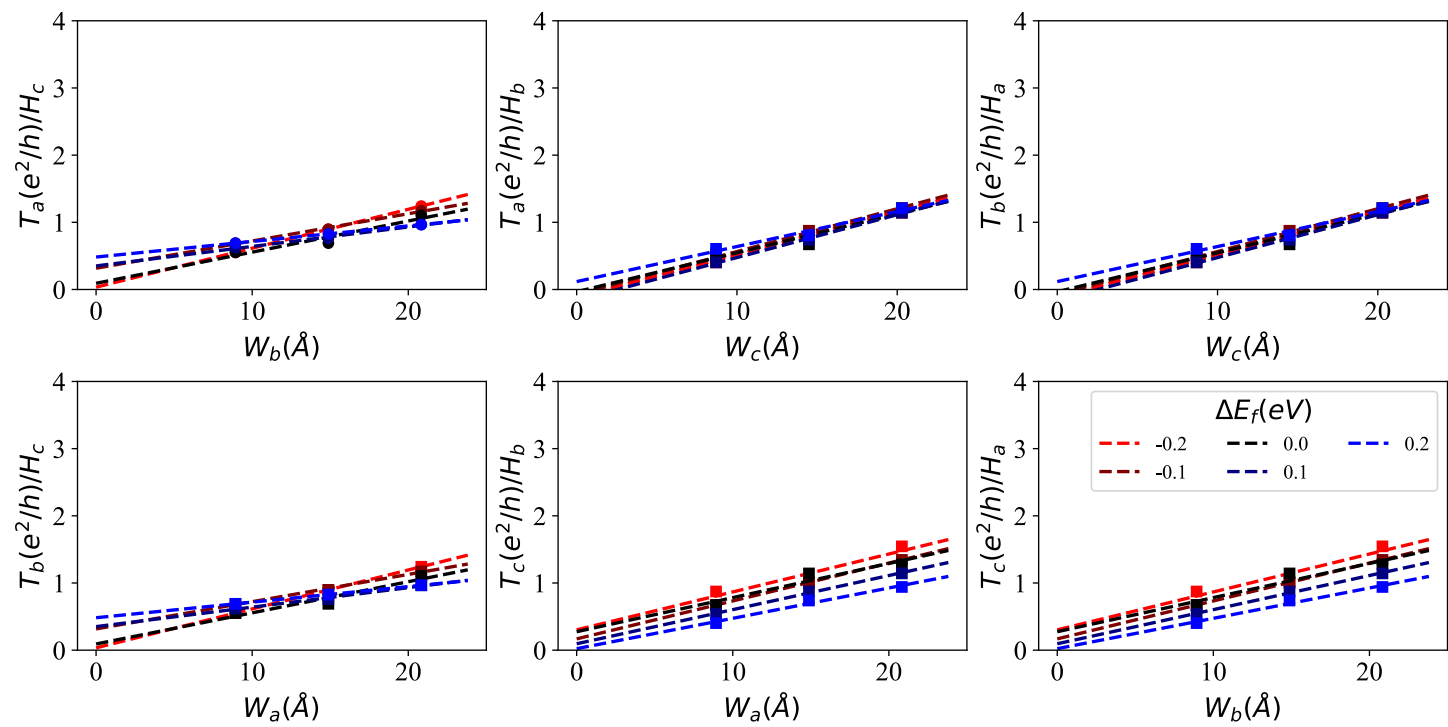



Compound: NbP  
Materials Project ID: 9339

Lattice (conventional cell):

| Parameter        | Value   | Unit |
|------------------|---------|------|
| a                | 3.3564  | Å    |
| b                | 3.3564  | Å    |
| c                | 11.4365 | Å    |
| $\alpha$ (alpha) | 90.0000 | °    |
| $\beta$ (beta)   | 90.0000 | °    |
| $\gamma$ (gamma) | 90.0000 | °    |

Crystal structure (conventional cell):

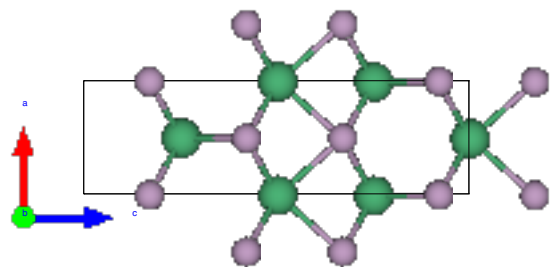

Nanowire Transmission:

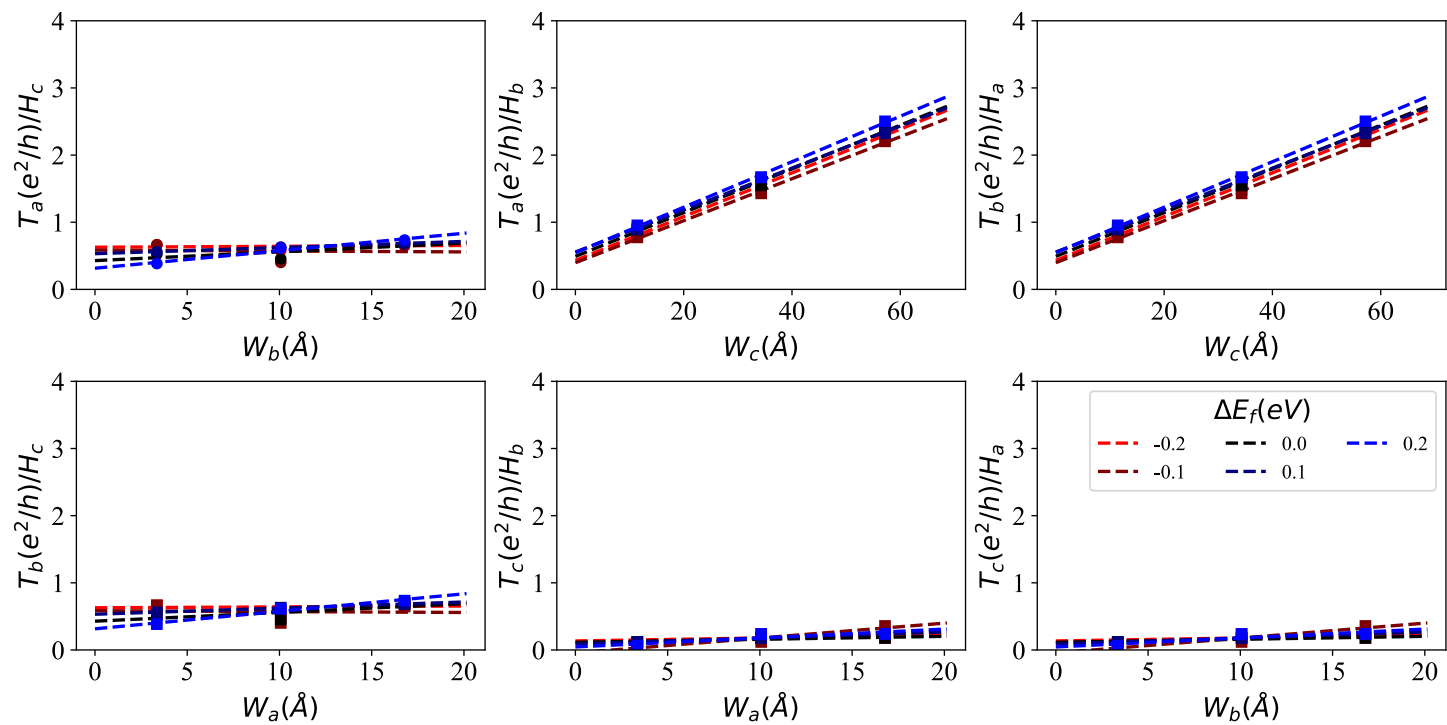

Compound: NbP<sub>2</sub>  
Materials Project ID: 1077116

Lattice (conventional cell):

| Parameter        | Value    | Unit |
|------------------|----------|------|
| a                | 8.9129   | Å    |
| b                | 3.2925   | Å    |
| c                | 7.5664   | Å    |
| $\alpha$ (alpha) | 90.0000  | °    |
| $\beta$ (beta)   | 118.9943 | °    |
| $\gamma$ (gamma) | 90.0000  | °    |

Crystal structure (conventional cell):

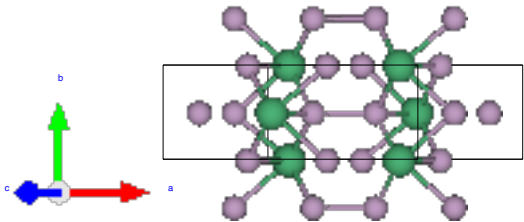

Nanowire Transmission:

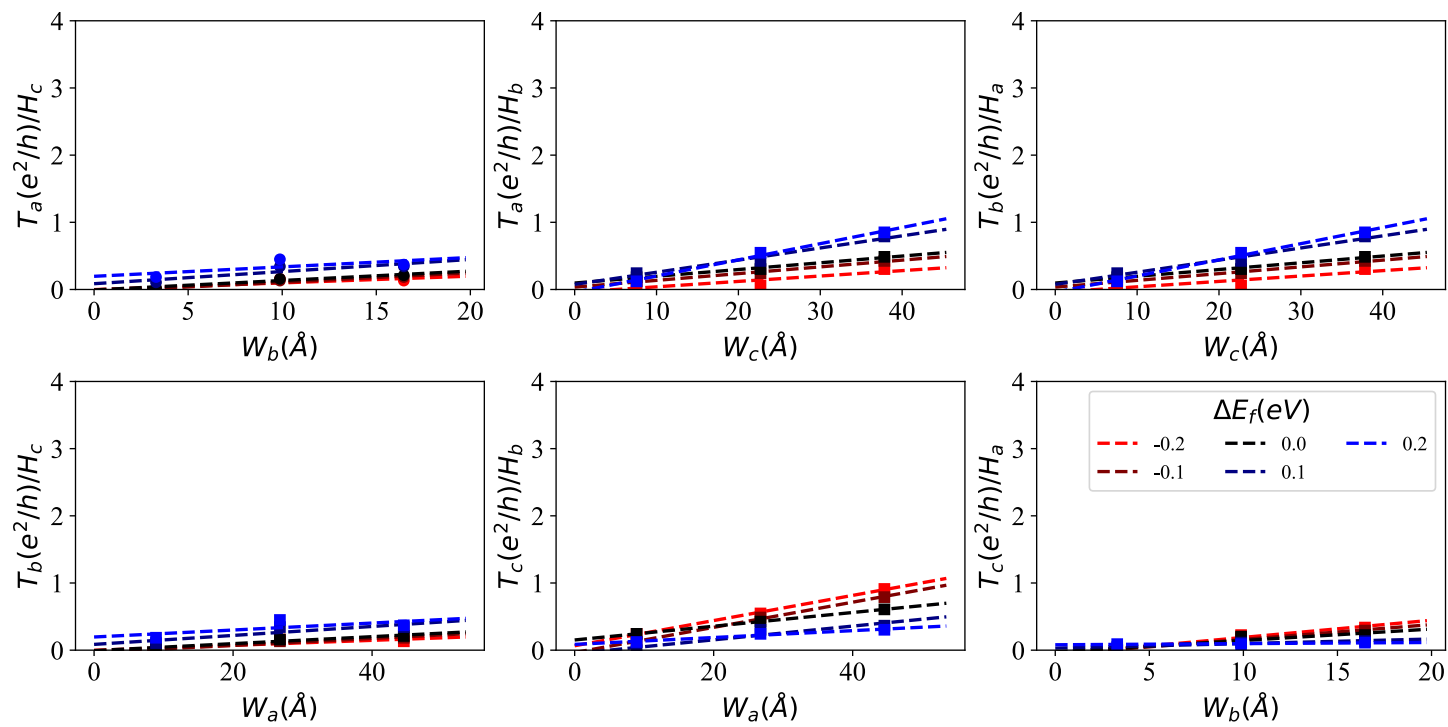

Compound: NbS  
Materials Project ID: 2243

Lattice (conventional cell):

| Parameter        | Value    | Unit |
|------------------|----------|------|
| a                | 3.3186   | Å    |
| b                | 3.3186   | Å    |
| c                | 3.3243   | Å    |
| $\alpha$ (alpha) | 90.0000  | °    |
| $\beta$ (beta)   | 90.0000  | °    |
| $\gamma$ (gamma) | 120.0000 | °    |

Crystal structure (conventional cell):

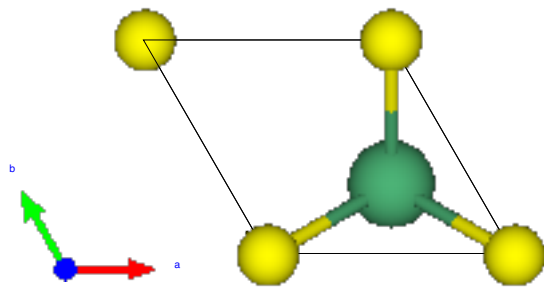

Nanowire Transmission:

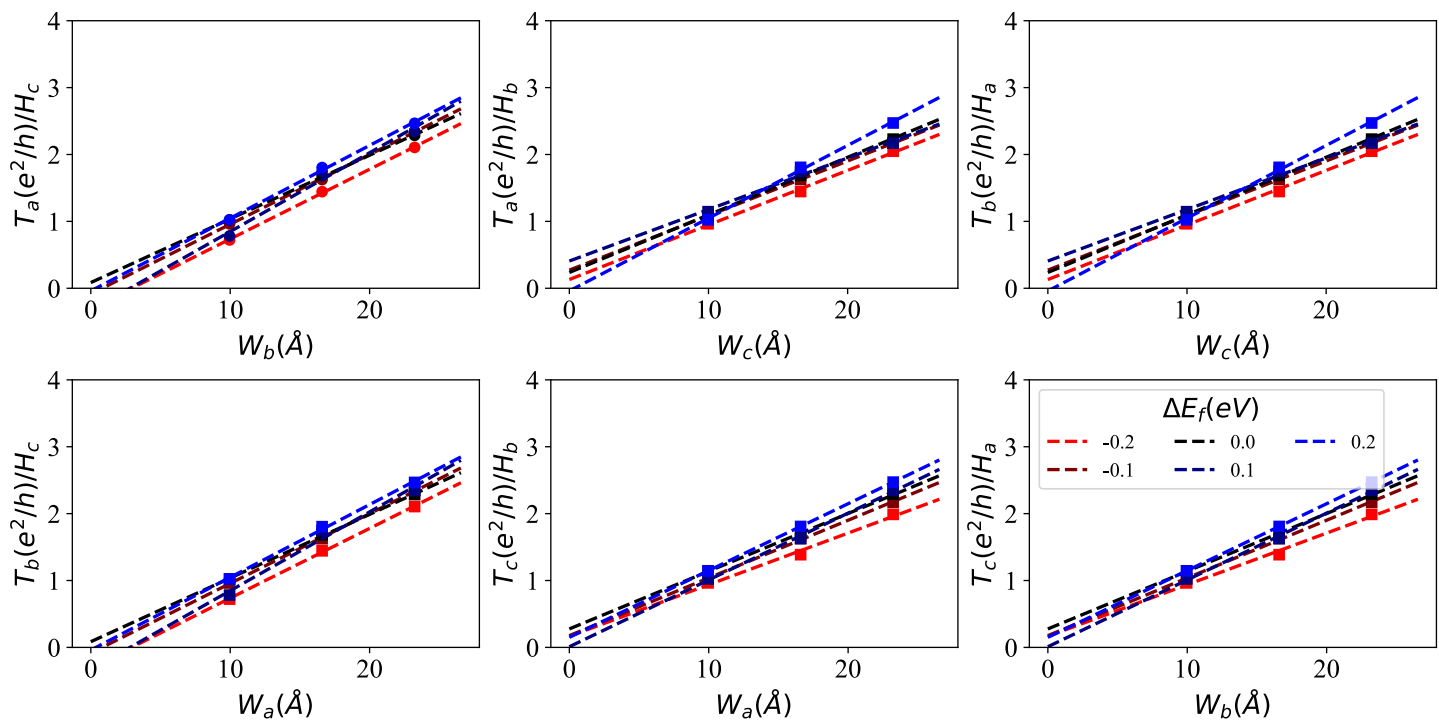

Compound: NbSe<sub>4</sub>  
Materials Project ID: 1078815

Lattice (conventional cell):

| Parameter | Value   | Unit |
|-----------|---------|------|
| a         | 5.9708  | Å    |
| b         | 5.9708  | Å    |
| c         | 6.5262  | Å    |
| α (alpha) | 90.0000 | °    |
| β (beta)  | 90.0000 | °    |
| γ (gamma) | 90.0000 | °    |

Crystal structure (conventional cell):

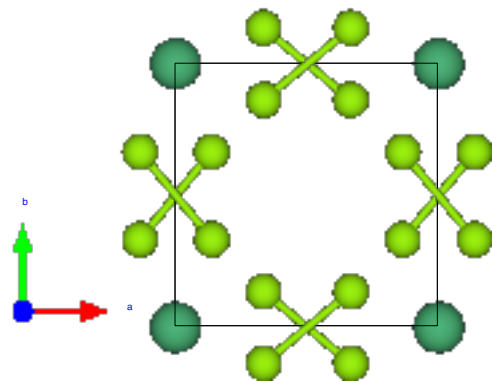

Nanowire Transmission:

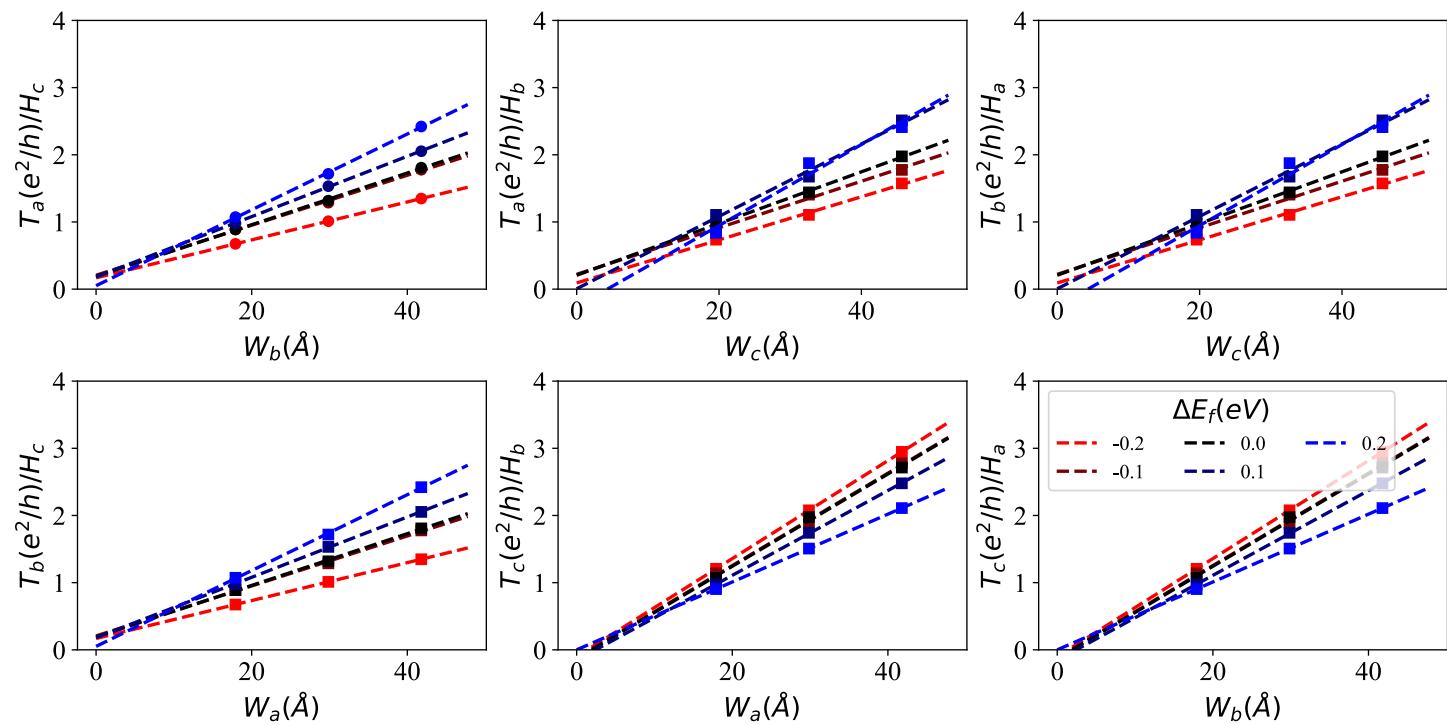

Compound: NbSiAs  
Materials Project ID: 21907

Lattice (conventional cell):

| Parameter        | Value   | Unit |
|------------------|---------|------|
| a                | 3.5165  | Å    |
| b                | 3.5165  | Å    |
| c                | 7.9705  | Å    |
| $\alpha$ (alpha) | 90.0000 | °    |
| $\beta$ (beta)   | 90.0000 | °    |
| $\gamma$ (gamma) | 90.0000 | °    |

Crystal structure (conventional cell):

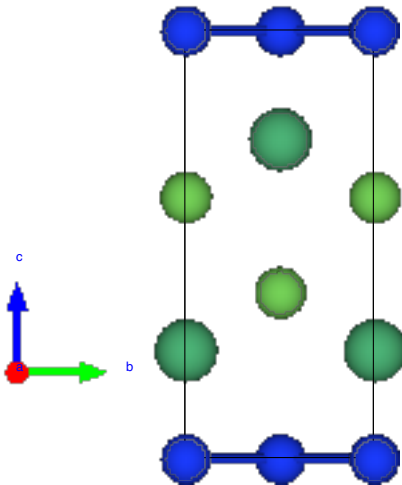

Nanowire Transmission:

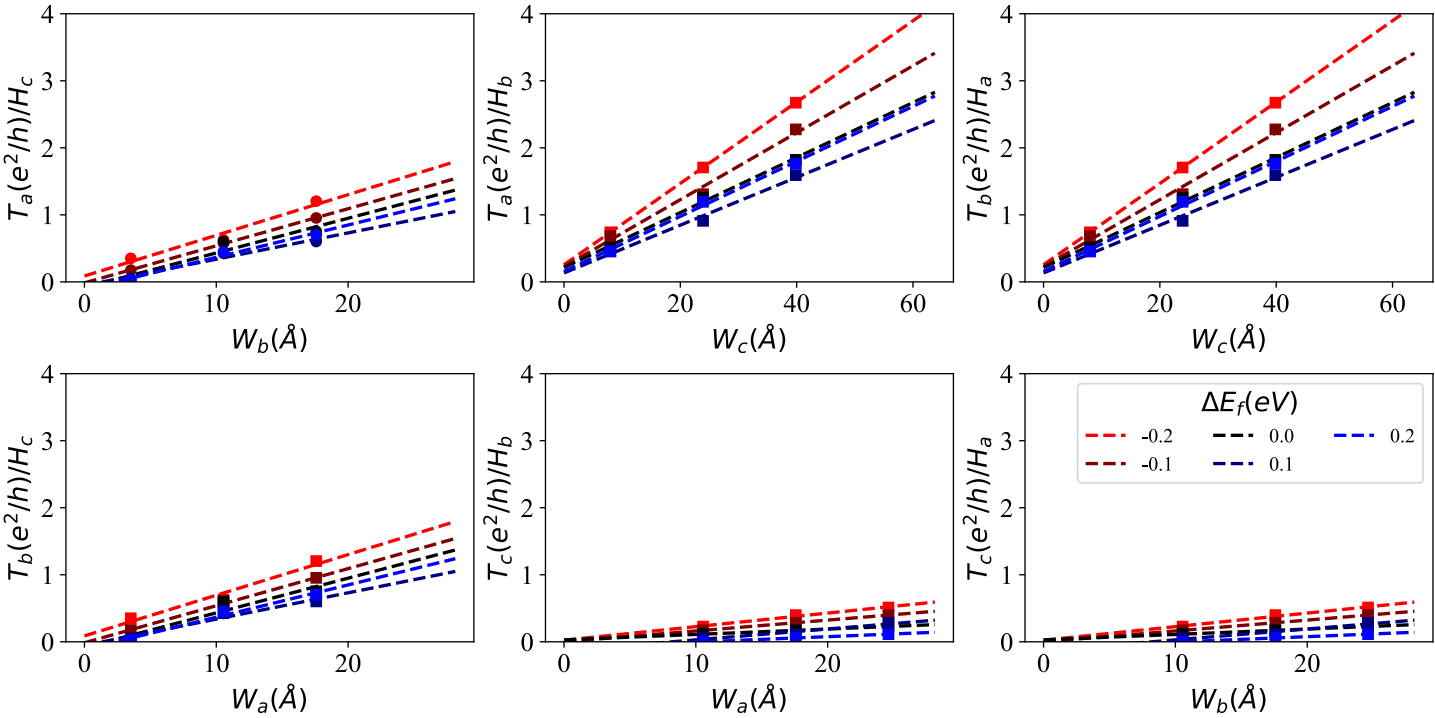

Compound: Ni(BMo)<sub>2</sub>  
Materials Project ID: 9999

Lattice (conventional cell):

| Parameter        | Value   | Unit |
|------------------|---------|------|
| a                | 3.1850  | Å    |
| b                | 4.5764  | Å    |
| c                | 7.1383  | Å    |
| $\alpha$ (alpha) | 90.0000 | °    |
| $\beta$ (beta)   | 90.0000 | °    |
| $\gamma$ (gamma) | 90.0000 | °    |

Crystal structure (conventional cell):

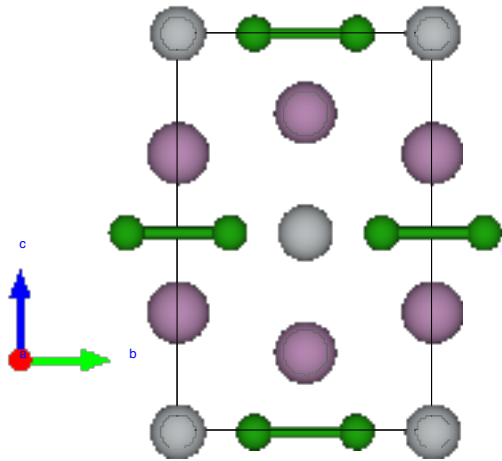

Nanowire Transmission:

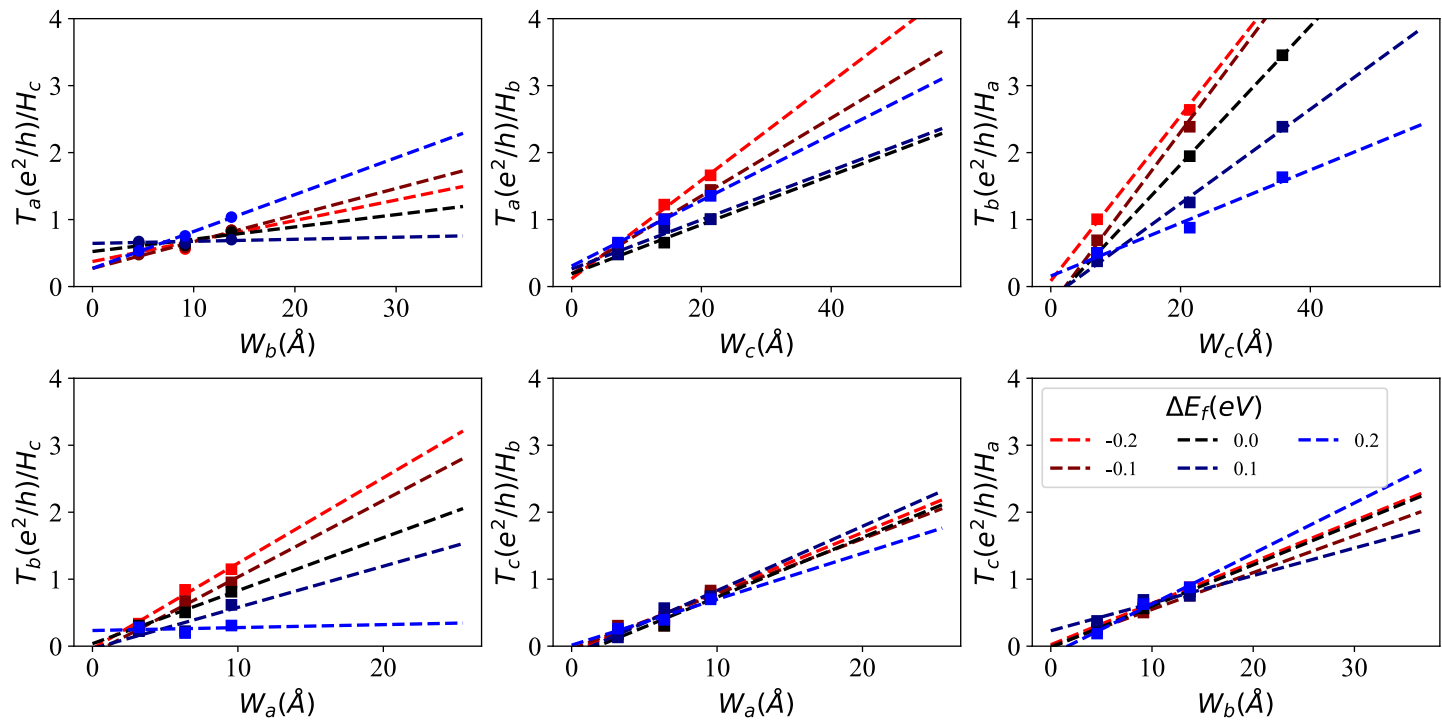

Compound: NiS  
Materials Project ID: 1547

Lattice (conventional cell):

| Parameter        | Value    | Unit |
|------------------|----------|------|
| a                | 9.5644   | Å    |
| b                | 9.5644   | Å    |
| c                | 3.1260   | Å    |
| $\alpha$ (alpha) | 90.0000  | °    |
| $\beta$ (beta)   | 90.0000  | °    |
| $\gamma$ (gamma) | 120.0000 | °    |

Crystal structure (conventional cell):

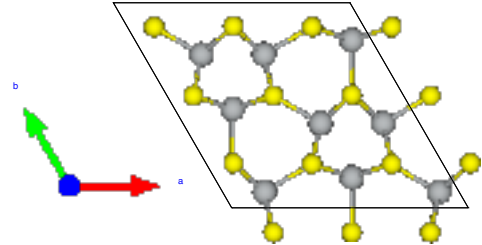

Nanowire Transmission:

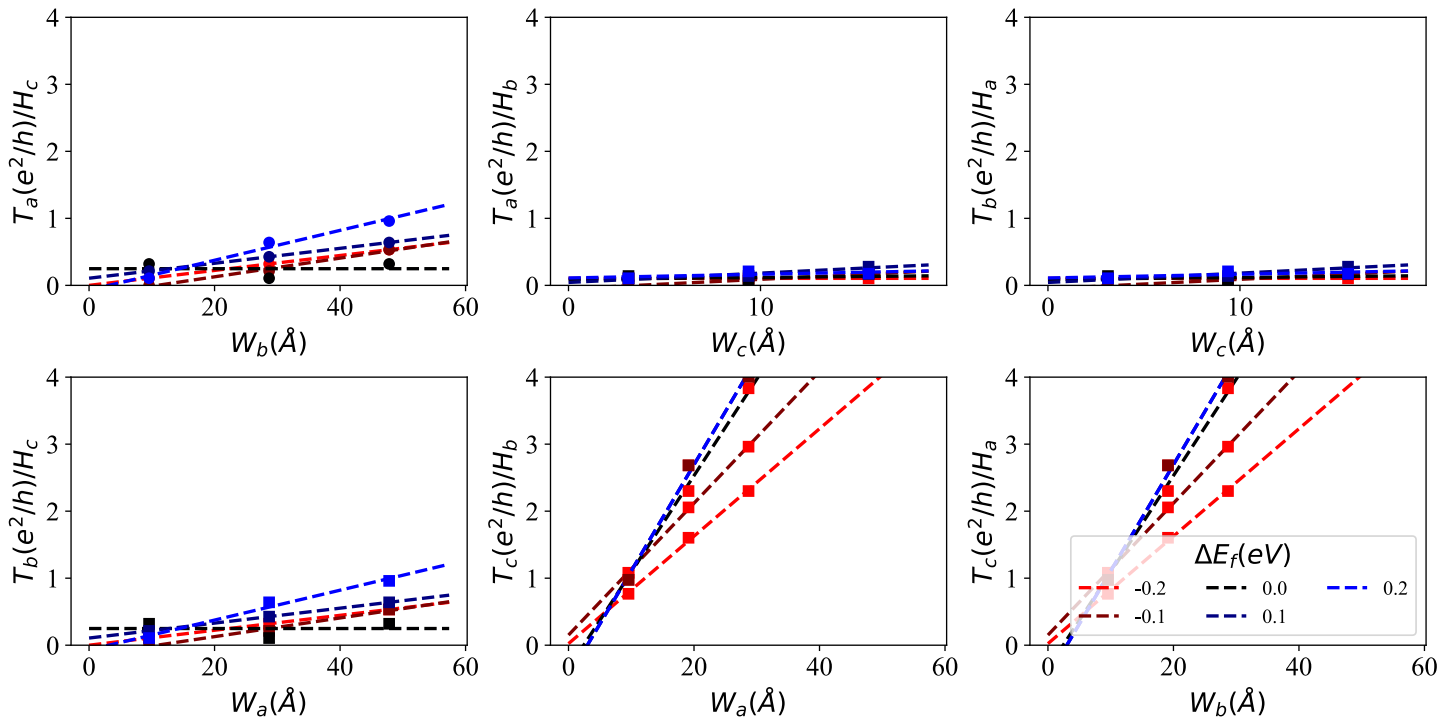

Compound: NiSe  
Materials Project ID: 15651

Lattice (conventional cell):

| Parameter        | Value    | Unit |
|------------------|----------|------|
| a                | 10.0013  | Å    |
| b                | 10.0013  | Å    |
| c                | 3.3350   | Å    |
| $\alpha$ (alpha) | 90.0000  | °    |
| $\beta$ (beta)   | 90.0000  | °    |
| $\gamma$ (gamma) | 120.0000 | °    |

Crystal structure (conventional cell):

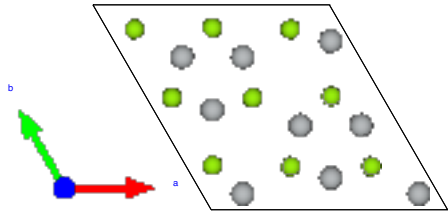

Nanowire Transmission:

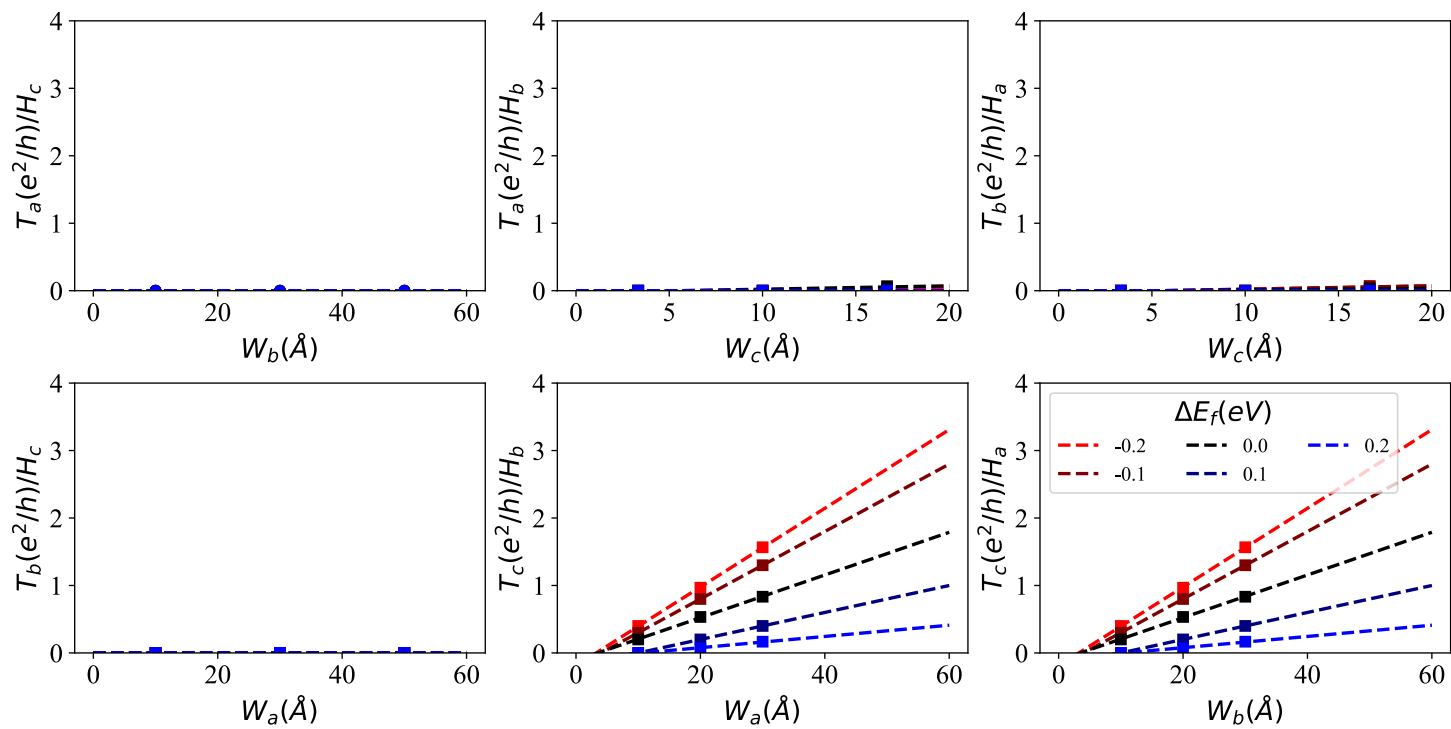



Compound: Pd<sub>2</sub>N  
Materials Project ID: 510087

Lattice (conventional cell):

| Parameter        | Value   | Unit |
|------------------|---------|------|
| a                | 2.9424  | Å    |
| b                | 4.8726  | Å    |
| c                | 5.4625  | Å    |
| $\alpha$ (alpha) | 90.0000 | °    |
| $\beta$ (beta)   | 90.0000 | °    |
| $\gamma$ (gamma) | 90.0000 | °    |

Crystal structure (conventional cell):

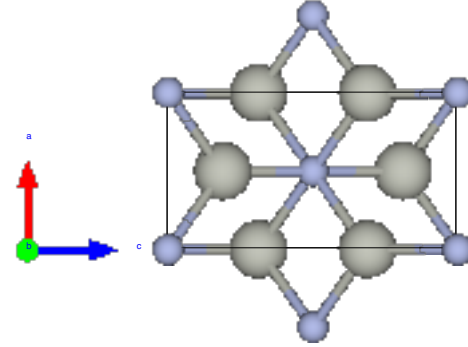

Nanowire Transmission:

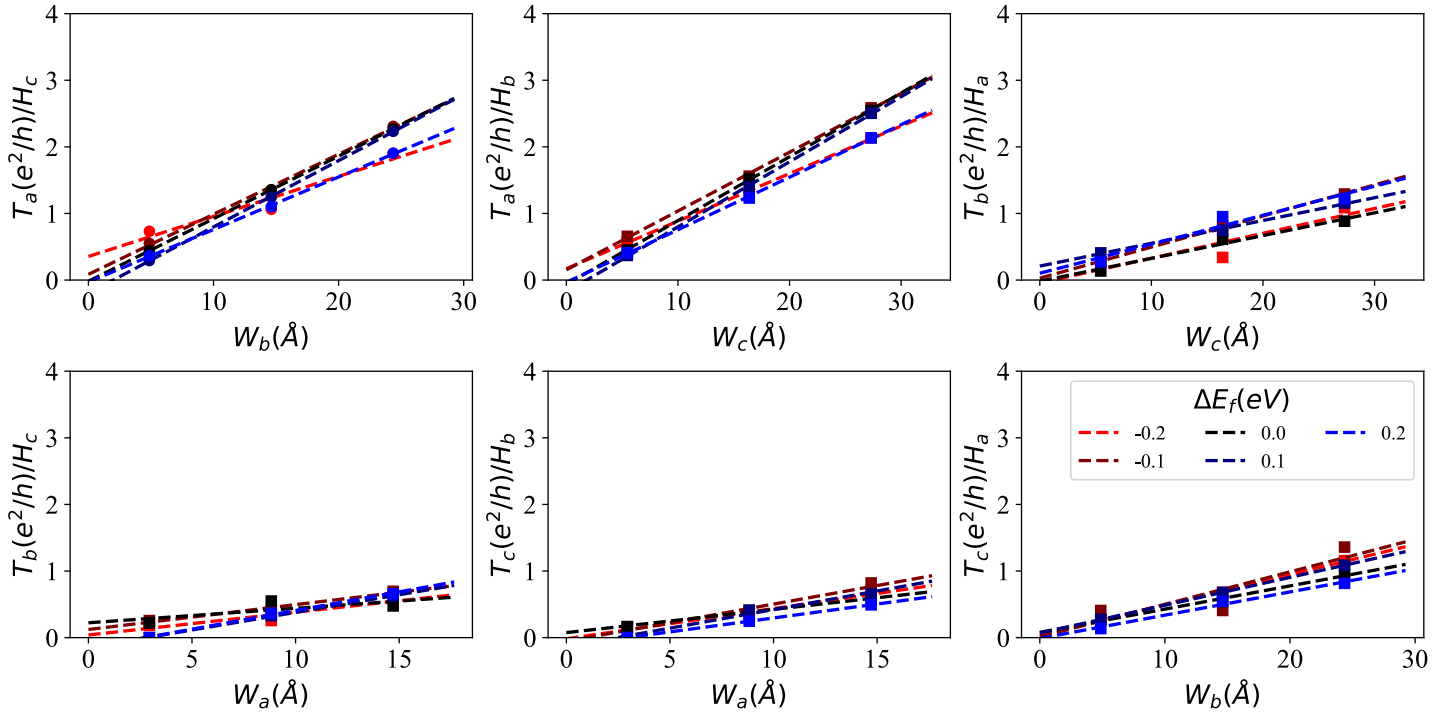

Compound: Re  
Materials Project ID: 8

Lattice (conventional cell):

| Parameter        | Value    | Unit |
|------------------|----------|------|
| a                | 2.7811   | Å    |
| b                | 2.7811   | Å    |
| c                | 4.4971   | Å    |
| $\alpha$ (alpha) | 90.0000  | °    |
| $\beta$ (beta)   | 90.0000  | °    |
| $\gamma$ (gamma) | 120.0000 | °    |

Crystal structure (conventional cell):

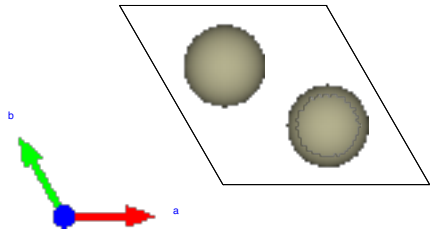

Nanowire Transmission:

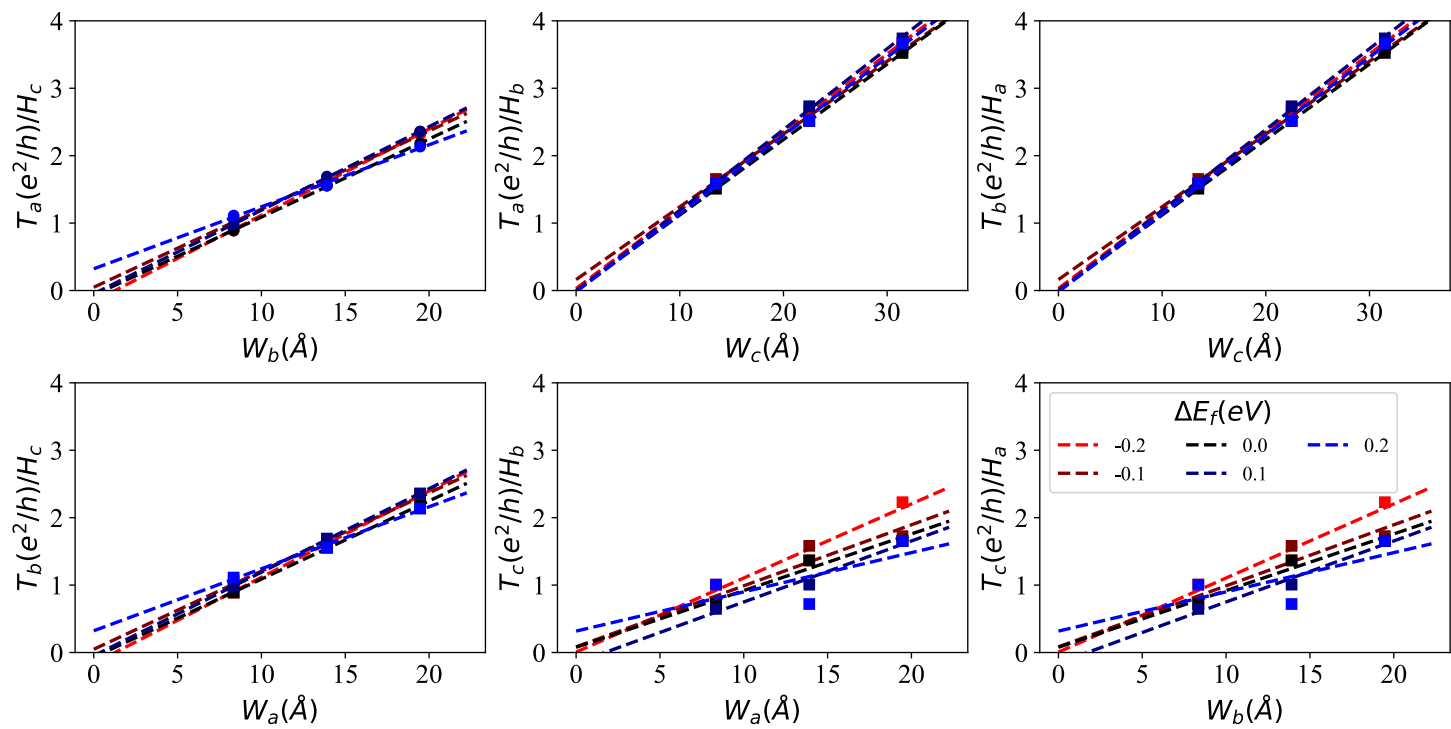

Compound: Ru  
Materials Project ID: 33

Lattice (conventional cell):

| Parameter        | Value    | Unit |
|------------------|----------|------|
| a                | 2.7329   | Å    |
| b                | 2.7329   | Å    |
| c                | 4.3139   | Å    |
| $\alpha$ (alpha) | 90.0000  | °    |
| $\beta$ (beta)   | 90.0000  | °    |
| $\gamma$ (gamma) | 120.0000 | °    |

Crystal structure (conventional cell):

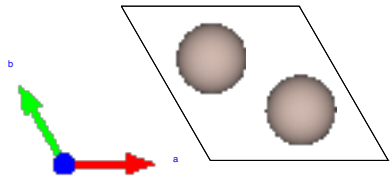

Nanowire Transmission:

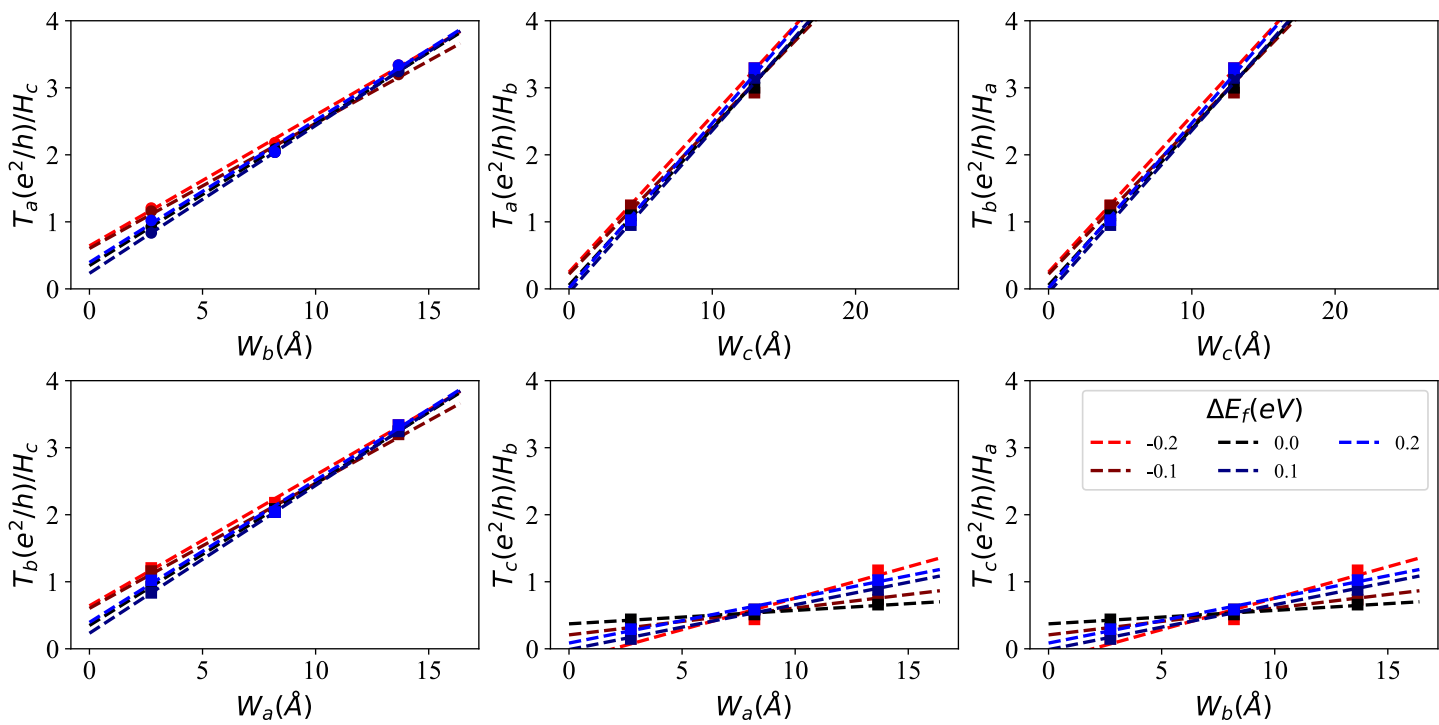

Compound: ScGa<sub>3</sub>  
Materials Project ID: 932

Lattice (conventional cell):

| Parameter        | Value   | Unit |
|------------------|---------|------|
| a                | 4.1216  | Å    |
| b                | 4.1216  | Å    |
| c                | 4.1216  | Å    |
| $\alpha$ (alpha) | 90.0000 | °    |
| $\beta$ (beta)   | 90.0000 | °    |
| $\gamma$ (gamma) | 90.0000 | °    |

Crystal structure (conventional cell):

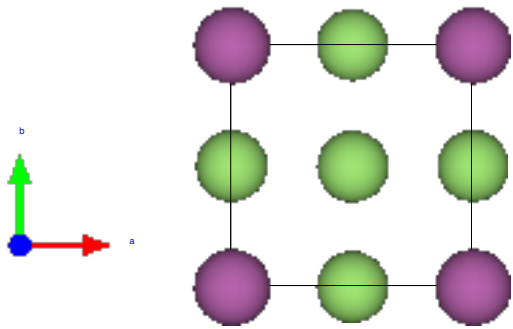

Nanowire Transmission:

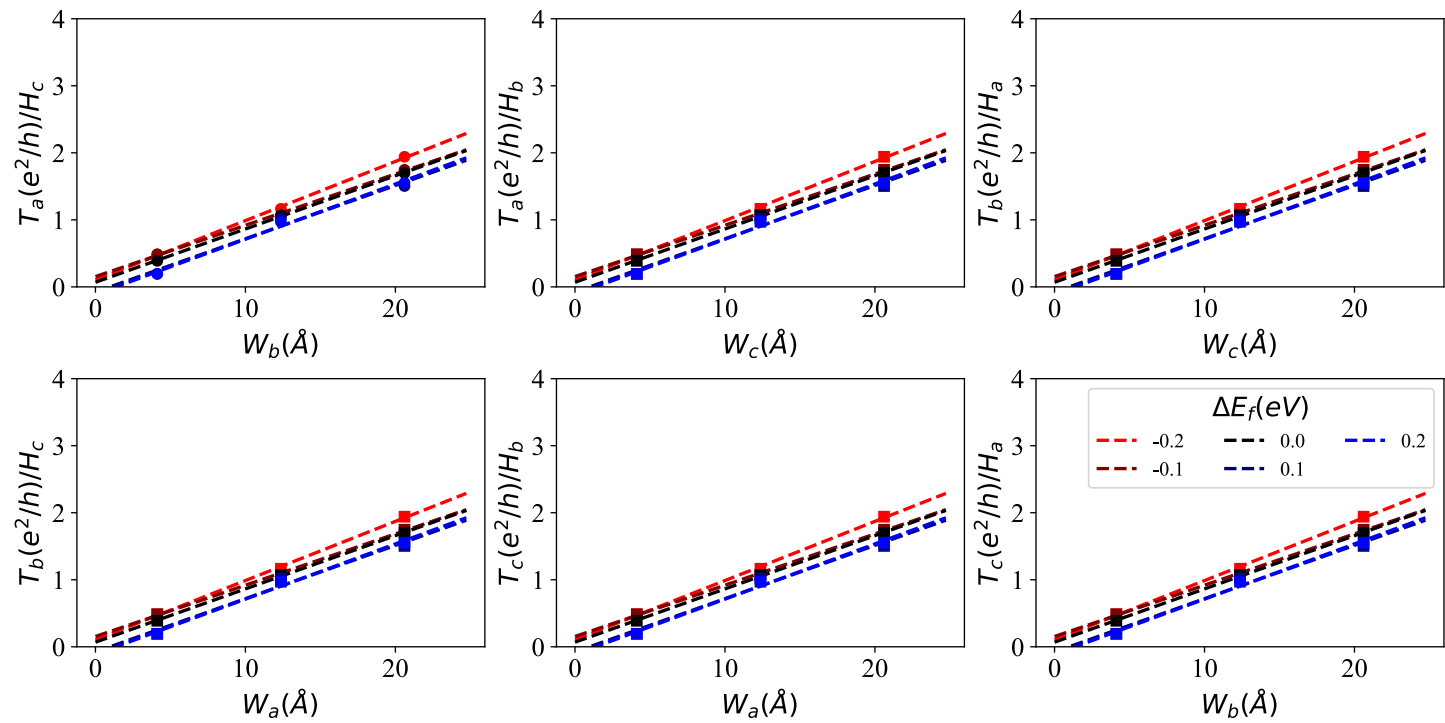

Compound: Se  
Materials Project ID: 14

Lattice (conventional cell):

| Parameter        | Value    | Unit |
|------------------|----------|------|
| a                | 4.5195   | Å    |
| b                | 4.5195   | Å    |
| c                | 5.0500   | Å    |
| $\alpha$ (alpha) | 90.0000  | °    |
| $\beta$ (beta)   | 90.0000  | °    |
| $\gamma$ (gamma) | 120.0000 | °    |

Crystal structure (conventional cell):

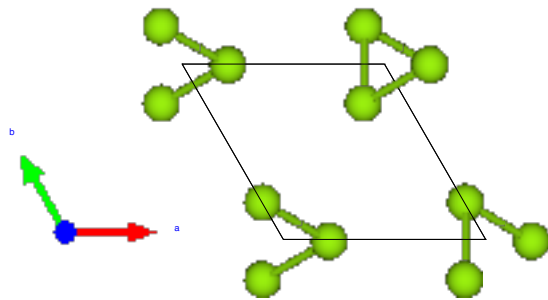

Nanowire Transmission:

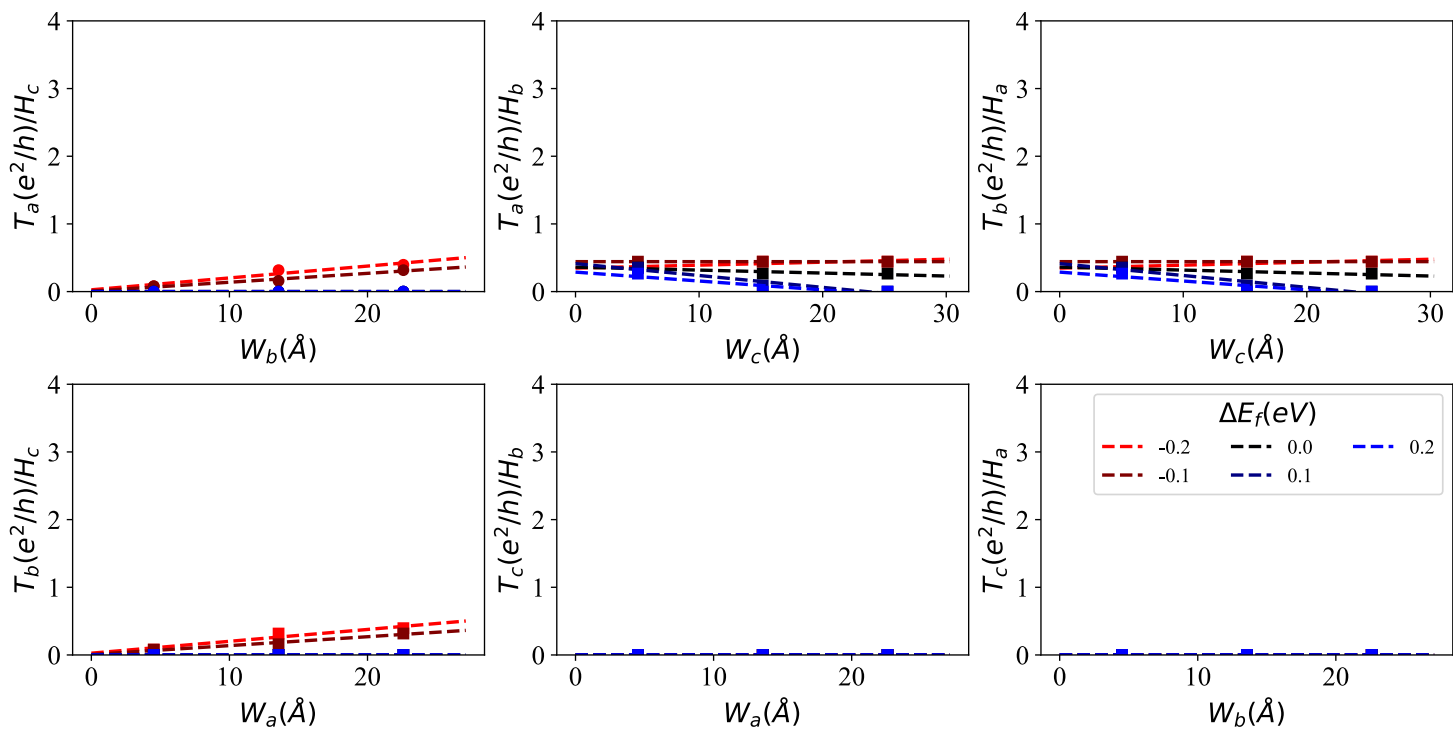

Compound: SiRh  
Materials Project ID: 1483

Lattice (conventional cell):

| Parameter        | Value   | Unit |
|------------------|---------|------|
| a                | 4.7295  | Å    |
| b                | 4.7295  | Å    |
| c                | 4.7295  | Å    |
| $\alpha$ (alpha) | 90.0000 | °    |
| $\beta$ (beta)   | 90.0000 | °    |
| $\gamma$ (gamma) | 90.0000 | °    |

Crystal structure (conventional cell):

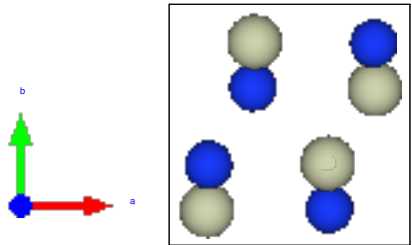

Nanowire Transmission:

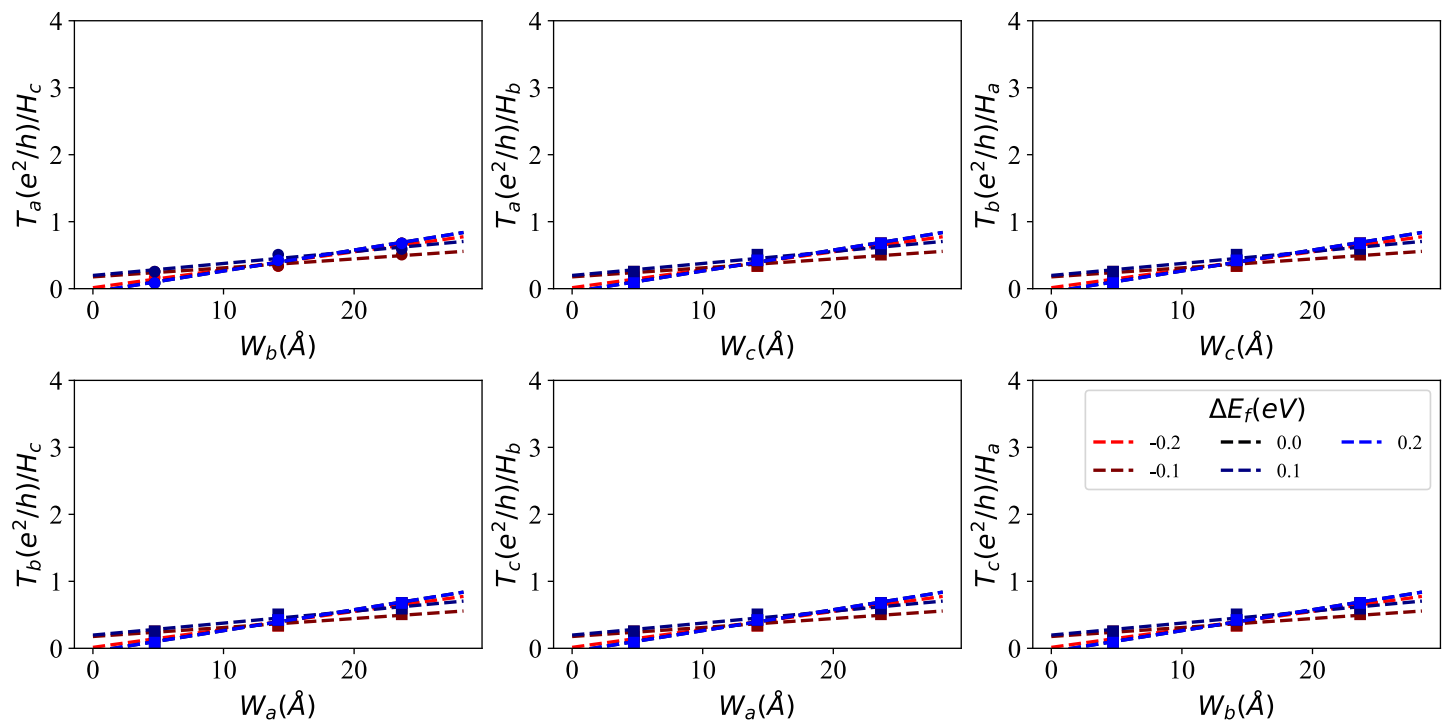

Compound: ScCuGe  
Materials Project ID: 1078430

Lattice (conventional cell):

| Parameter        | Value   | Unit |
|------------------|---------|------|
| a                | 6.5606  | Å    |
| b                | 6.5606  | Å    |
| c                | 3.9977  | Å    |
| $\alpha$ (alpha) | 90.0000 | °    |
| $\beta$ (beta)   | 90.0000 | °    |

Crystal structure (conventional cell):

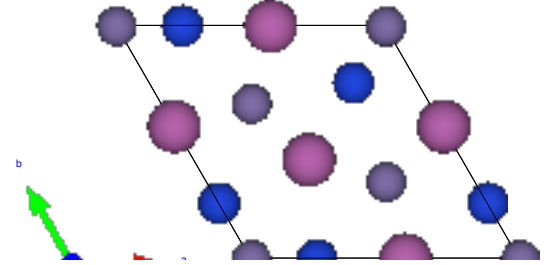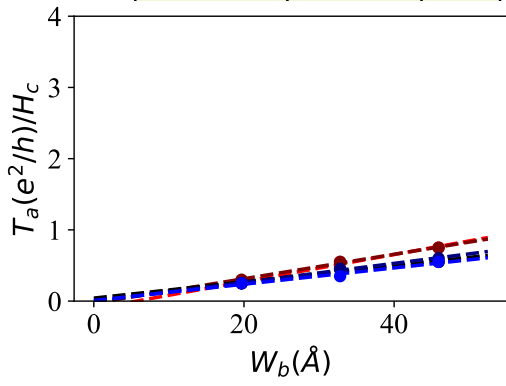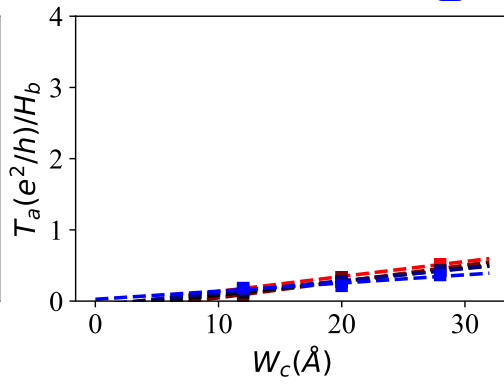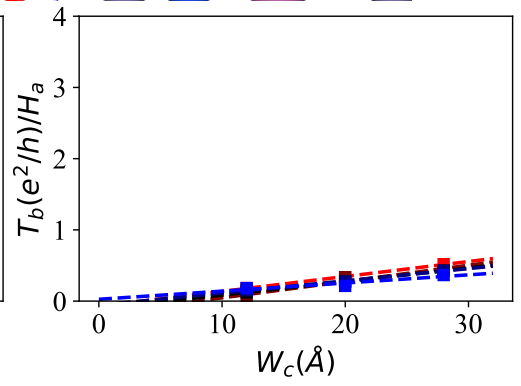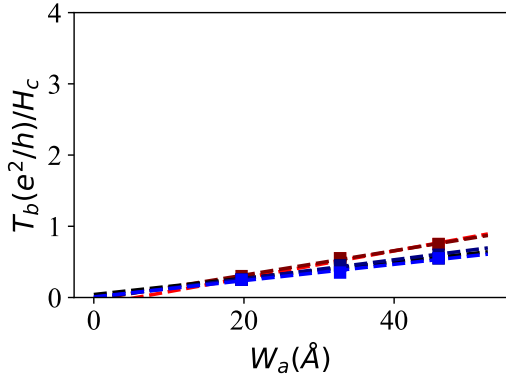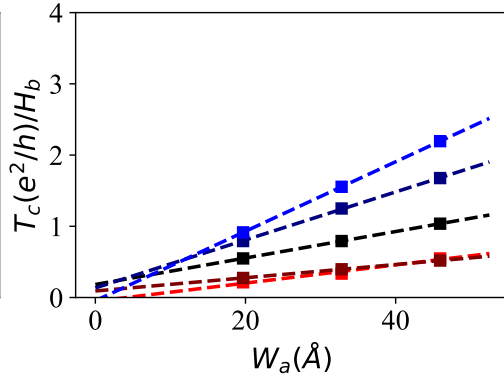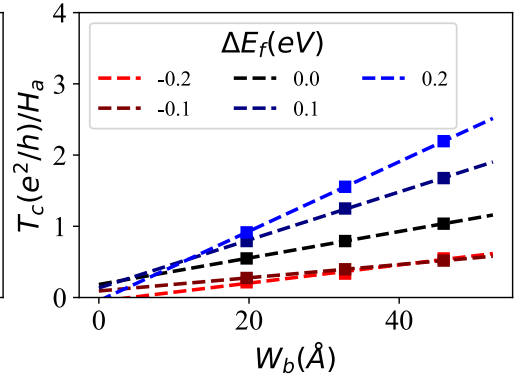

Compound: SnH4  
Materials Project ID: 1080725

Lattice (conventional cell):

| Parameter        | Value    | Unit |
|------------------|----------|------|
| a                | 3.9522   | Å    |
| b                | 3.9522   | Å    |
| c                | 6.4992   | Å    |
| $\alpha$ (alpha) | 90.0000  | °    |
| $\beta$ (beta)   | 90.0000  | °    |
| $\gamma$ (gamma) | 120.0000 | °    |

Crystal structure (conventional cell):

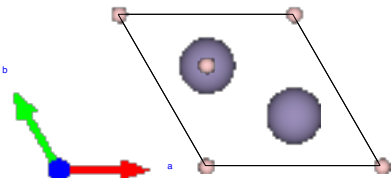

Nanowire Transmission:

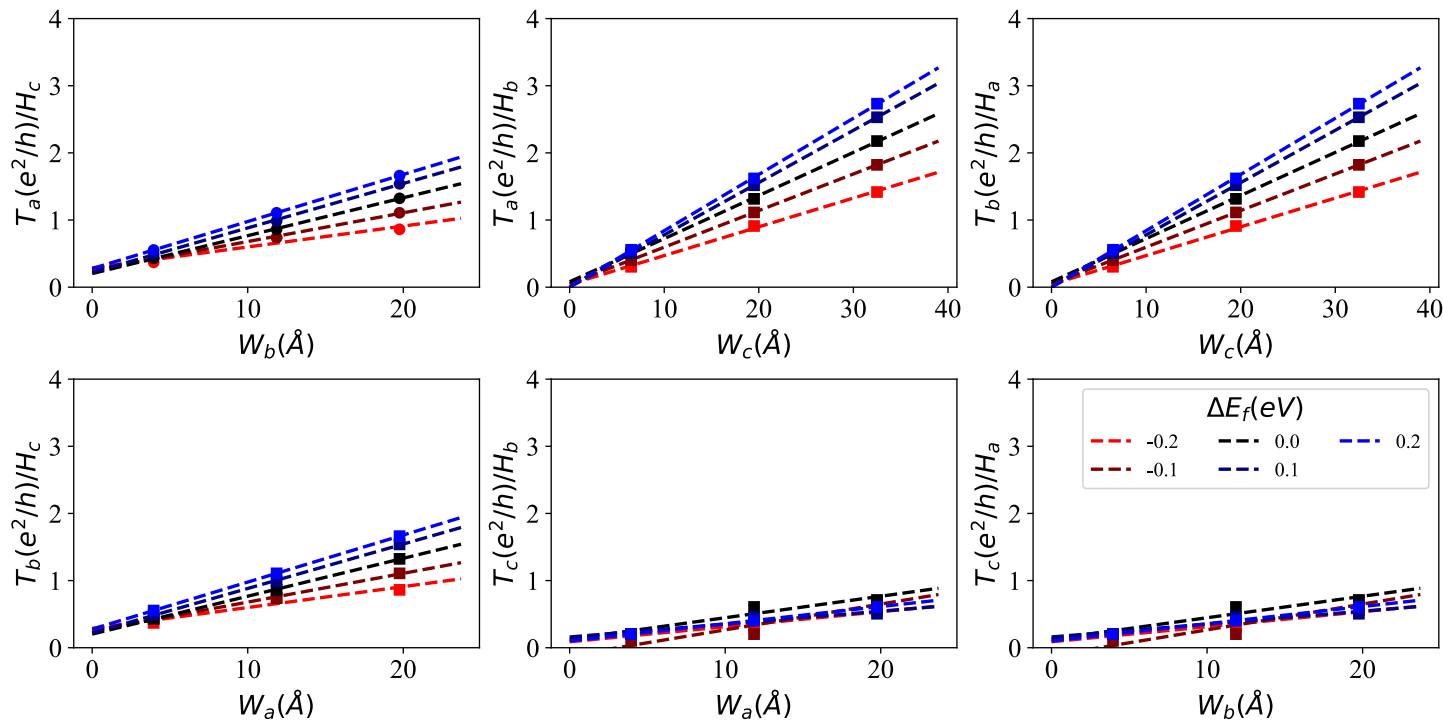



Compound:  $\text{Sn}(\text{HgSe}_2)_2$   
Materials Project ID: 10955

Lattice (conventional cell):

| Parameter        | Value   | Unit |
|------------------|---------|------|
| a                | 5.9365  | Å    |
| b                | 5.9365  | Å    |
| c                | 11.9940 | Å    |
| $\alpha$ (alpha) | 90.0000 | °    |
| $\beta$ (beta)   | 90.0000 | °    |
| $\gamma$ (gamma) | 90.0000 | °    |

Crystal structure (conventional cell):

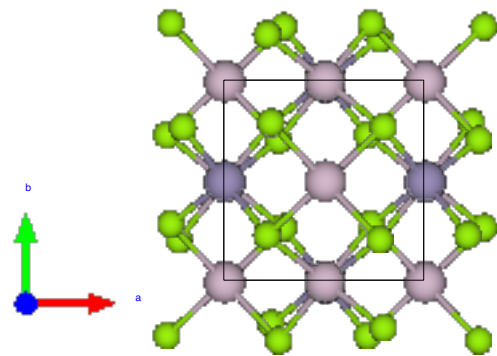

Nanowire Transmission:

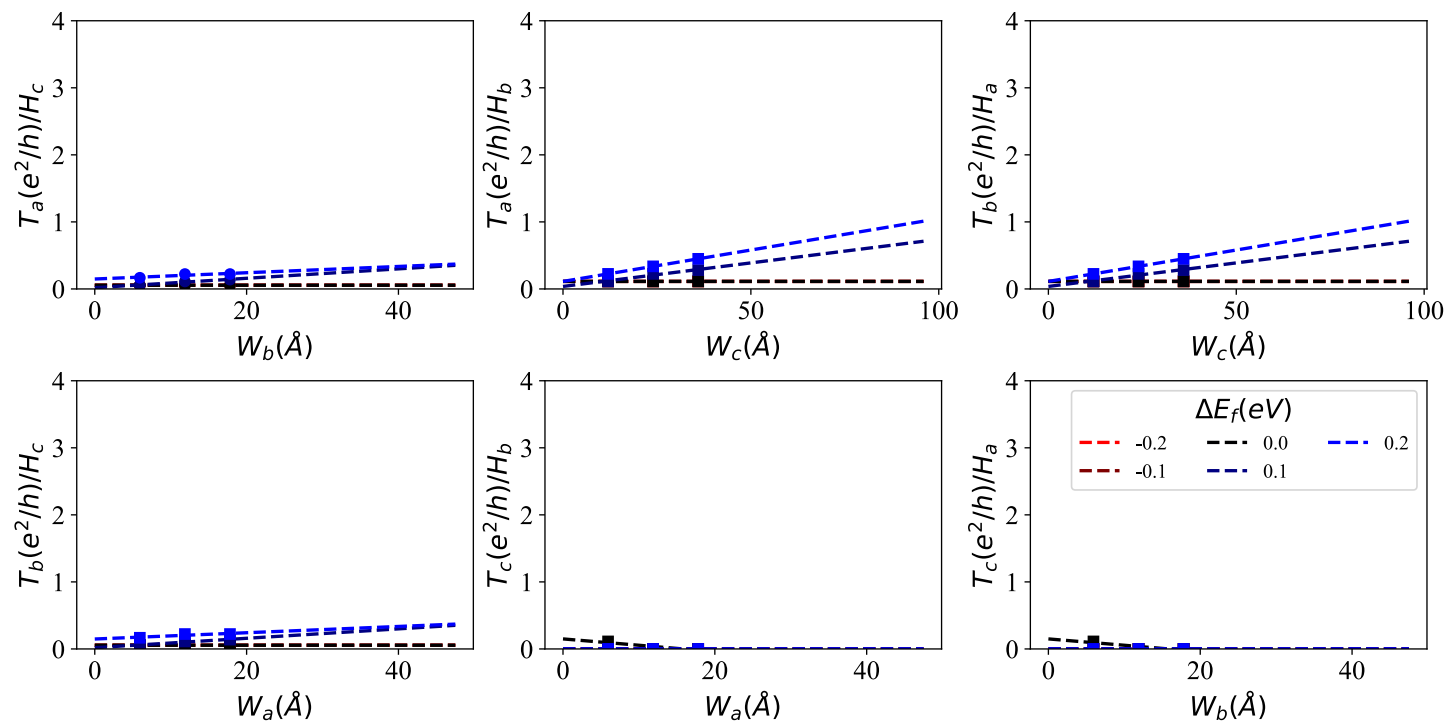

Compound:  $\text{Sr}(\text{CdSb})_2$   
Materials Project ID: 7432

Lattice (conventional cell):

| Parameter        | Value    | Unit |
|------------------|----------|------|
| a                | 4.7972   | Å    |
| b                | 4.7972   | Å    |
| c                | 7.9056   | Å    |
| $\alpha$ (alpha) | 90.0000  | °    |
| $\beta$ (beta)   | 90.0000  | °    |
| $\gamma$ (gamma) | 120.0000 | °    |

Crystal structure (conventional cell):

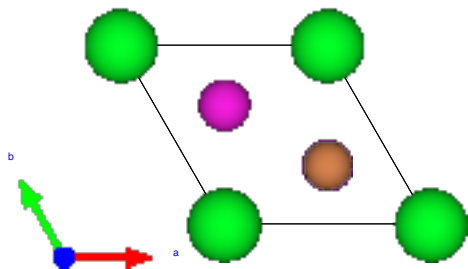

Nanowire Transmission:

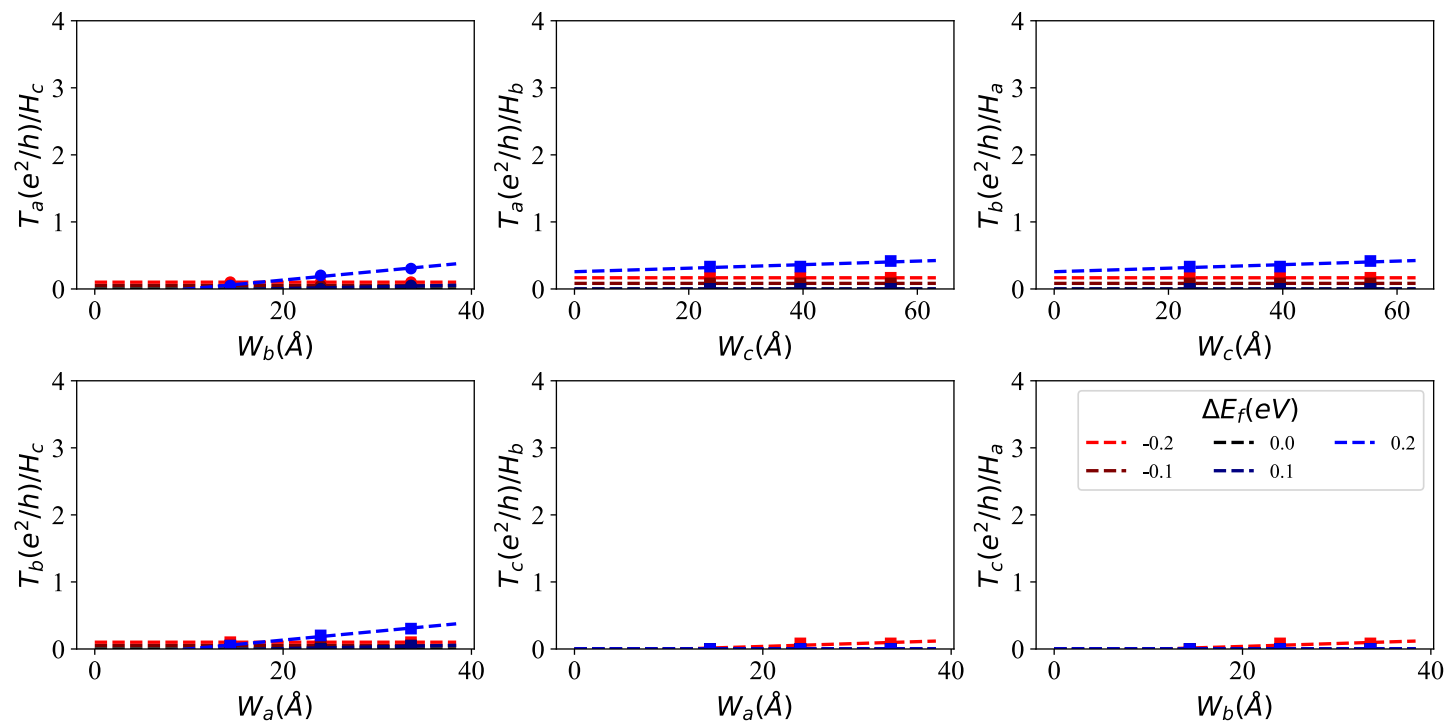

Compound:  $\text{Sr}_3(\text{AlGe})_2$   
Materials Project ID: 571216

Lattice (conventional cell):

| Parameter        | Value    | Unit |
|------------------|----------|------|
| a                | 12.7411  | Å    |
| b                | 4.2166   | Å    |
| c                | 8.9551   | Å    |
| $\alpha$ (alpha) | 90.0000  | °    |
| $\beta$ (beta)   | 110.1782 | °    |
| $\gamma$ (gamma) | 90.0000  | °    |

Crystal structure (conventional cell):

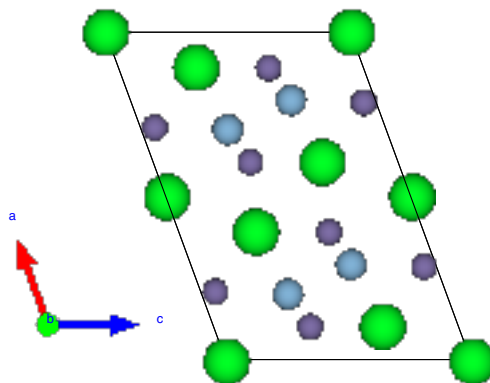

Nanowire Transmission:

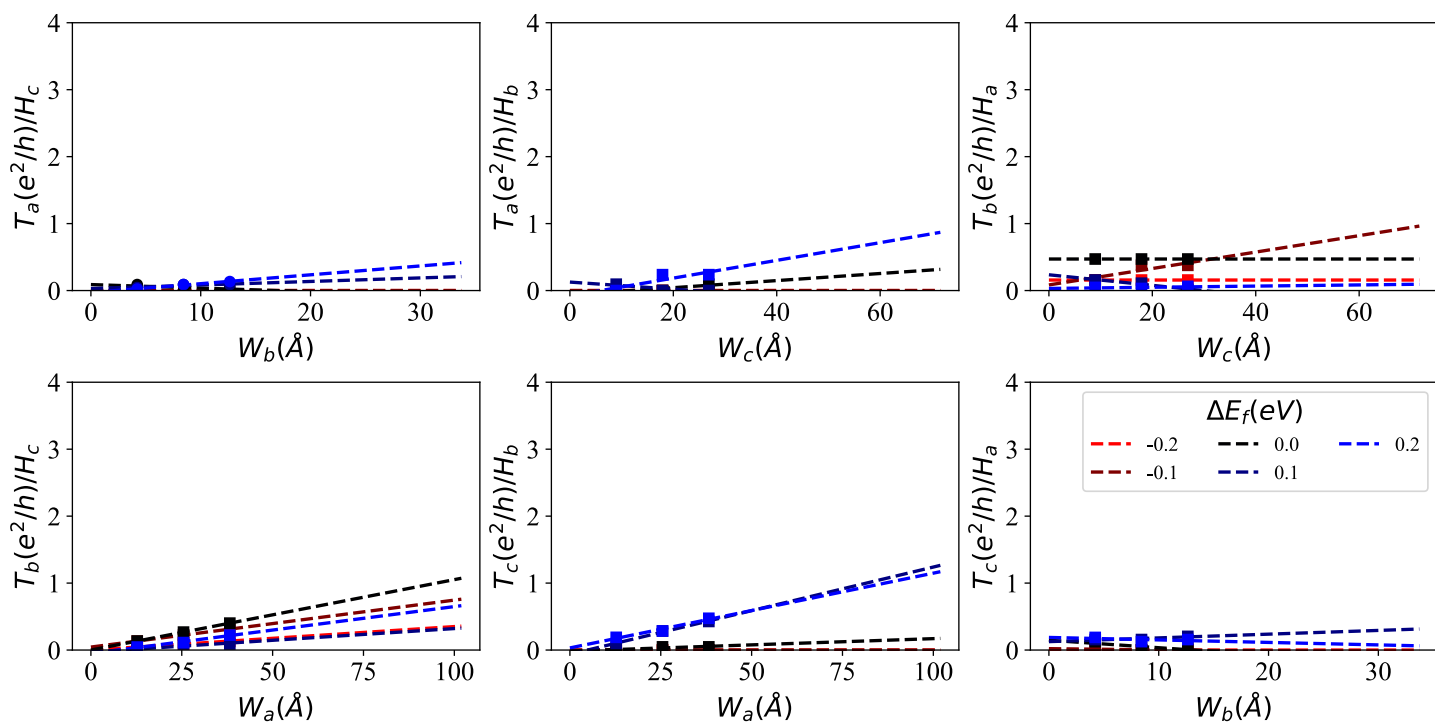

Compound: SrAs<sub>3</sub>  
Materials Project ID: 9907

Lattice (conventional cell):

| Parameter        | Value    | Unit |
|------------------|----------|------|
| a                | 9.7449   | Å    |
| b                | 7.7486   | Å    |
| c                | 5.9535   | Å    |
| $\alpha$ (alpha) | 90.0000  | °    |
| $\beta$ (beta)   | 112.9053 | °    |
| $\gamma$ (gamma) | 90.0000  | °    |

Crystal structure (conventional cell):

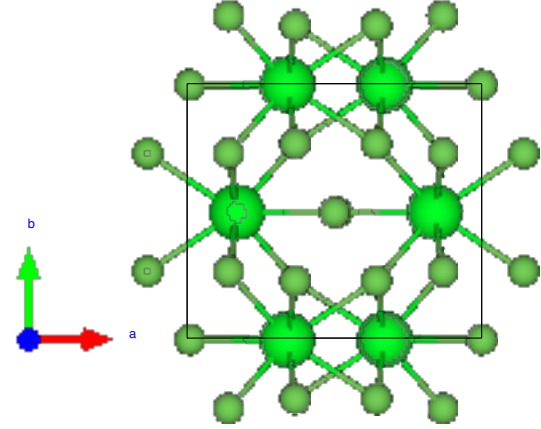

Nanowire Transmission:

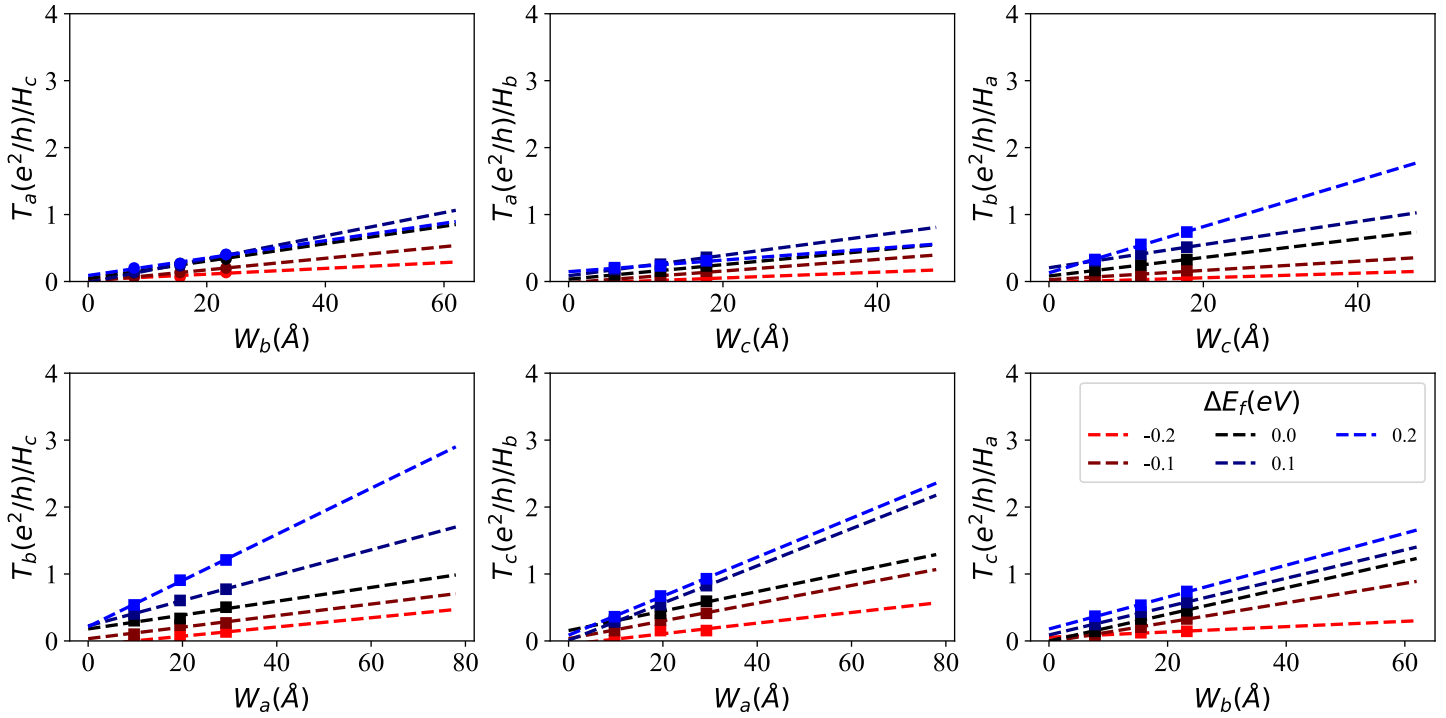

Compound:  $\text{Sr}_2\text{Bi}$   
Materials Project ID: 29619

Lattice (conventional cell):

| Parameter        | Value   | Unit |
|------------------|---------|------|
| a                | 5.1526  | Å    |
| b                | 5.1526  | Å    |
| c                | 18.1556 | Å    |
| $\alpha$ (alpha) | 90.0000 | °    |
| $\beta$ (beta)   | 90.0000 | °    |
| $\gamma$ (gamma) | 90.0000 | °    |

Crystal structure (conventional cell):

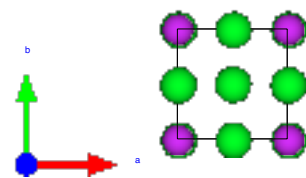

Nanowire Transmission:

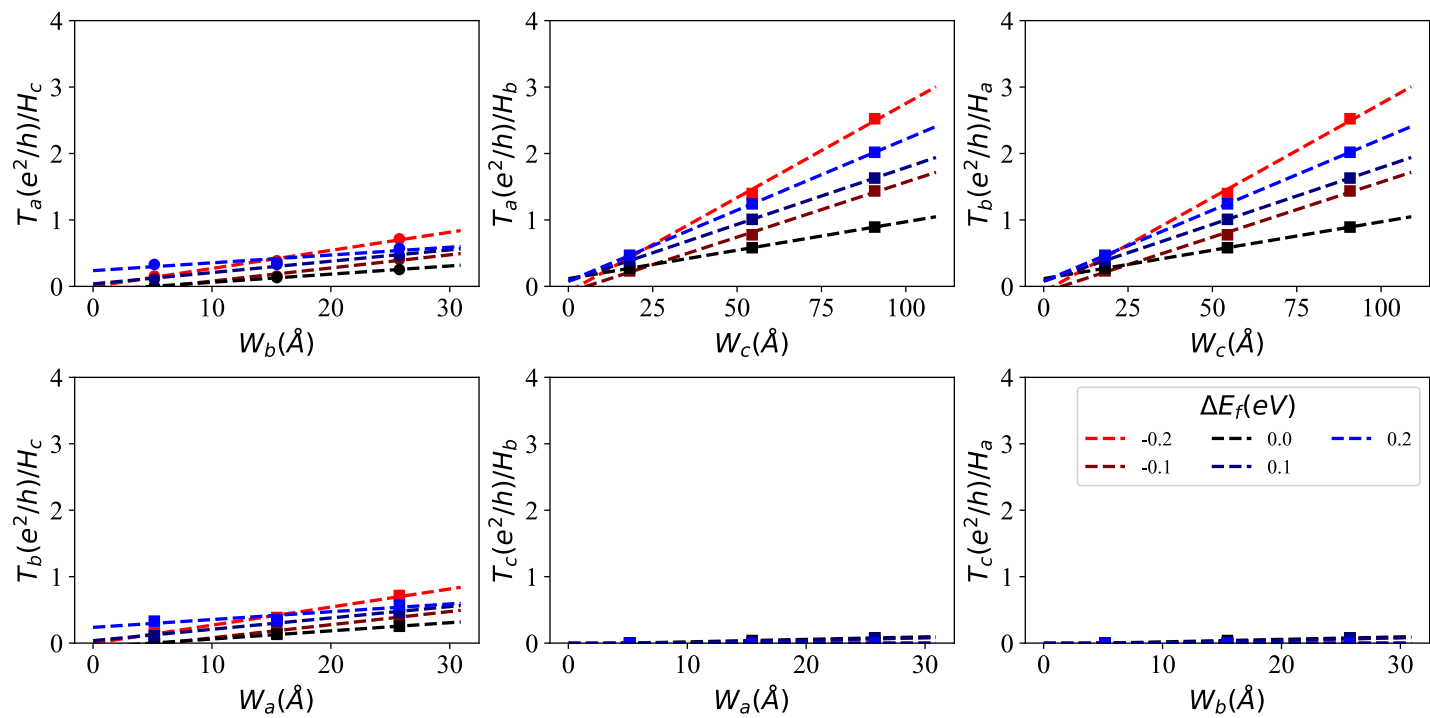

Compound: SrGe<sub>2</sub>  
Materials Project ID: 7390

Lattice (conventional cell):

| Parameter | Value    | Unit |
|-----------|----------|------|
| a         | 4.1699   | Å    |
| b         | 4.1699   | Å    |
| c         | 5.1991   | Å    |
| α (alpha) | 90.0000  | °    |
| β (beta)  | 90.0000  | °    |
| γ (gamma) | 120.0000 | °    |

Crystal structure (conventional cell):

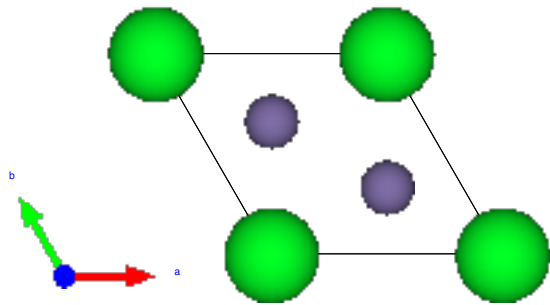

Nanowire Transmission:

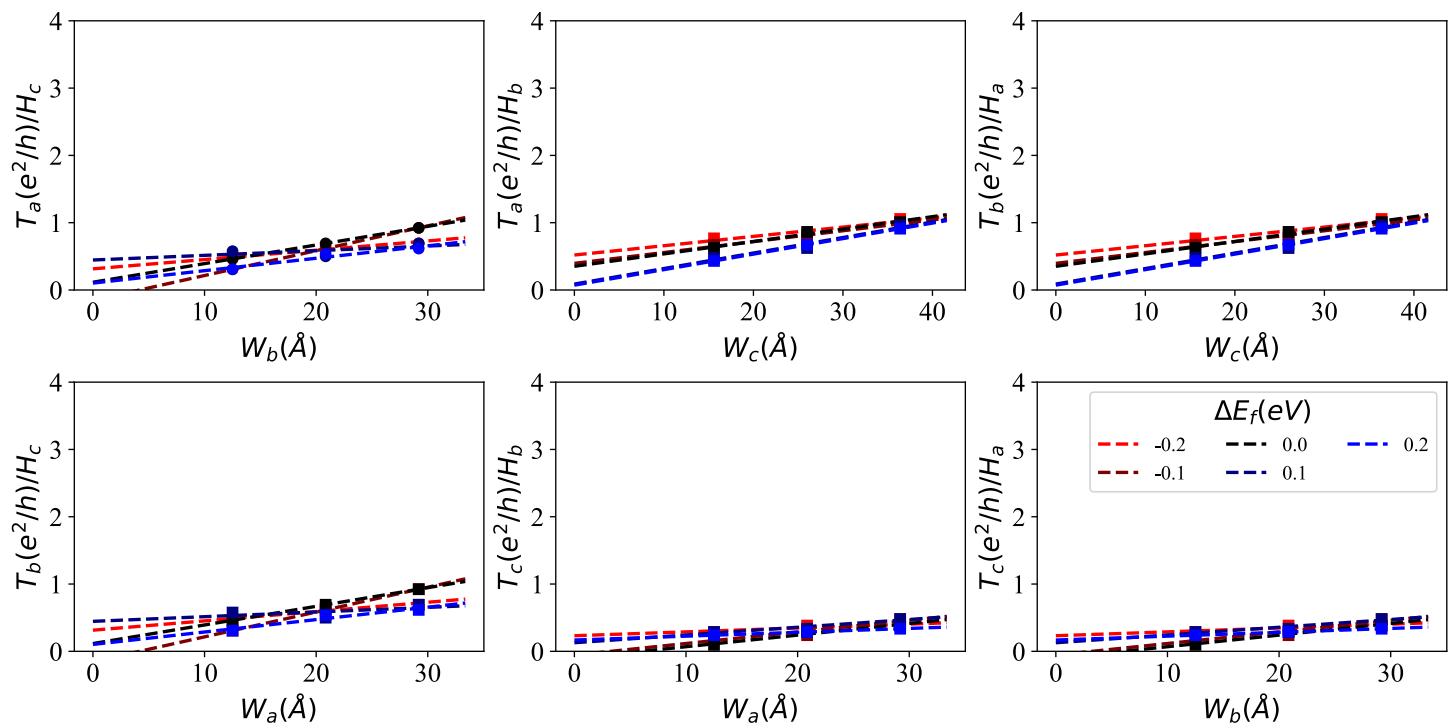

Compound:  $\text{SrMnSb}_2$   
Materials Project ID: 1079721

Lattice (conventional cell):

| Parameter        | Value   | Unit |
|------------------|---------|------|
| a                | 4.4170  | Å    |
| b                | 4.4170  | Å    |
| c                | 11.7201 | Å    |
| $\alpha$ (alpha) | 90.0000 | °    |
| $\beta$ (beta)   | 90.0000 | °    |
| $\gamma$ (gamma) | 90.0000 | °    |

Crystal structure (conventional cell):

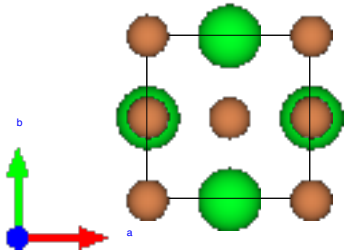

Nanowire Transmission:

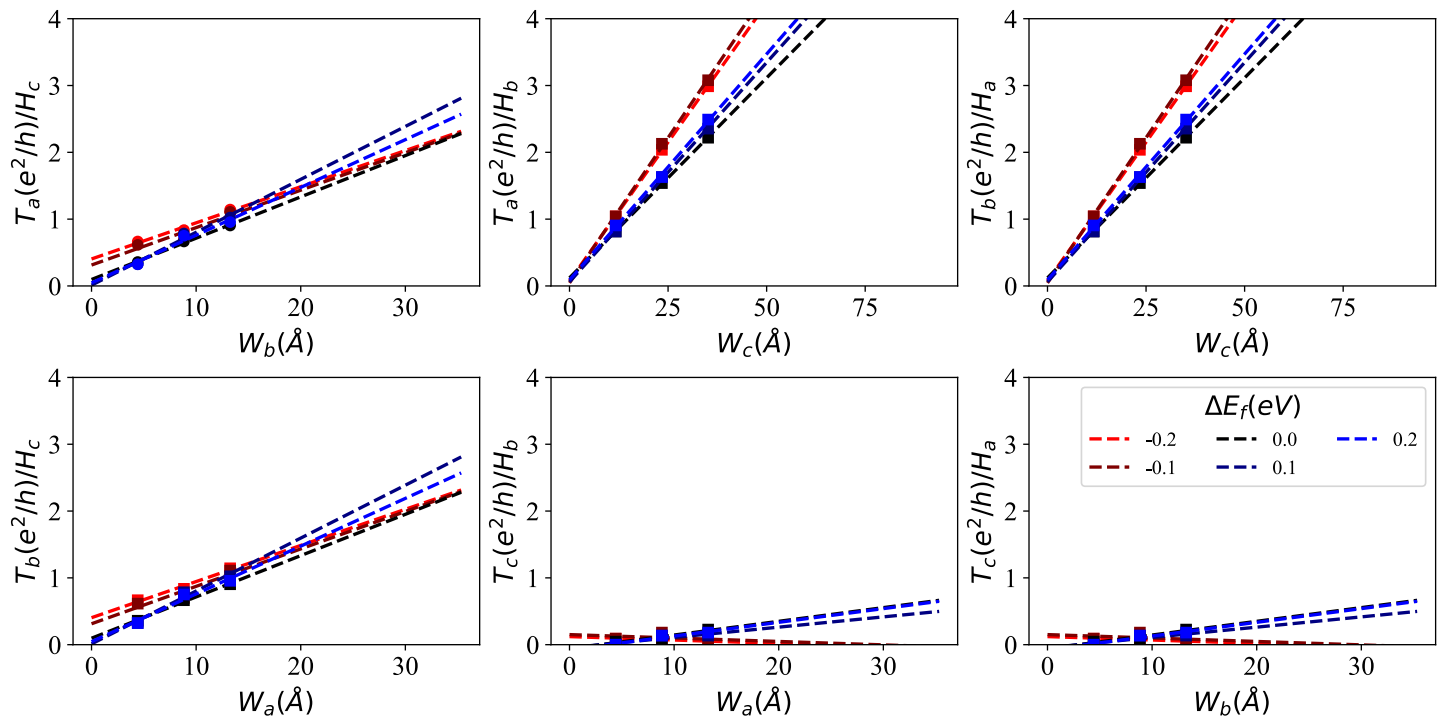

Compound:  $\text{SrSi}_2$   
Materials Project ID: 1727

Lattice (conventional cell):

| Parameter        | Value   | Unit |
|------------------|---------|------|
| a                | 4.4377  | Å    |
| b                | 4.4377  | Å    |
| c                | 13.9661 | Å    |
| $\alpha$ (alpha) | 90.0000 | °    |
| $\beta$ (beta)   | 90.0000 | °    |
| $\gamma$ (gamma) | 90.0000 | °    |

Crystal structure (conventional cell):

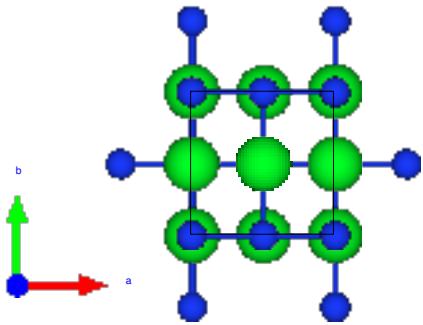

Nanowire Transmission:

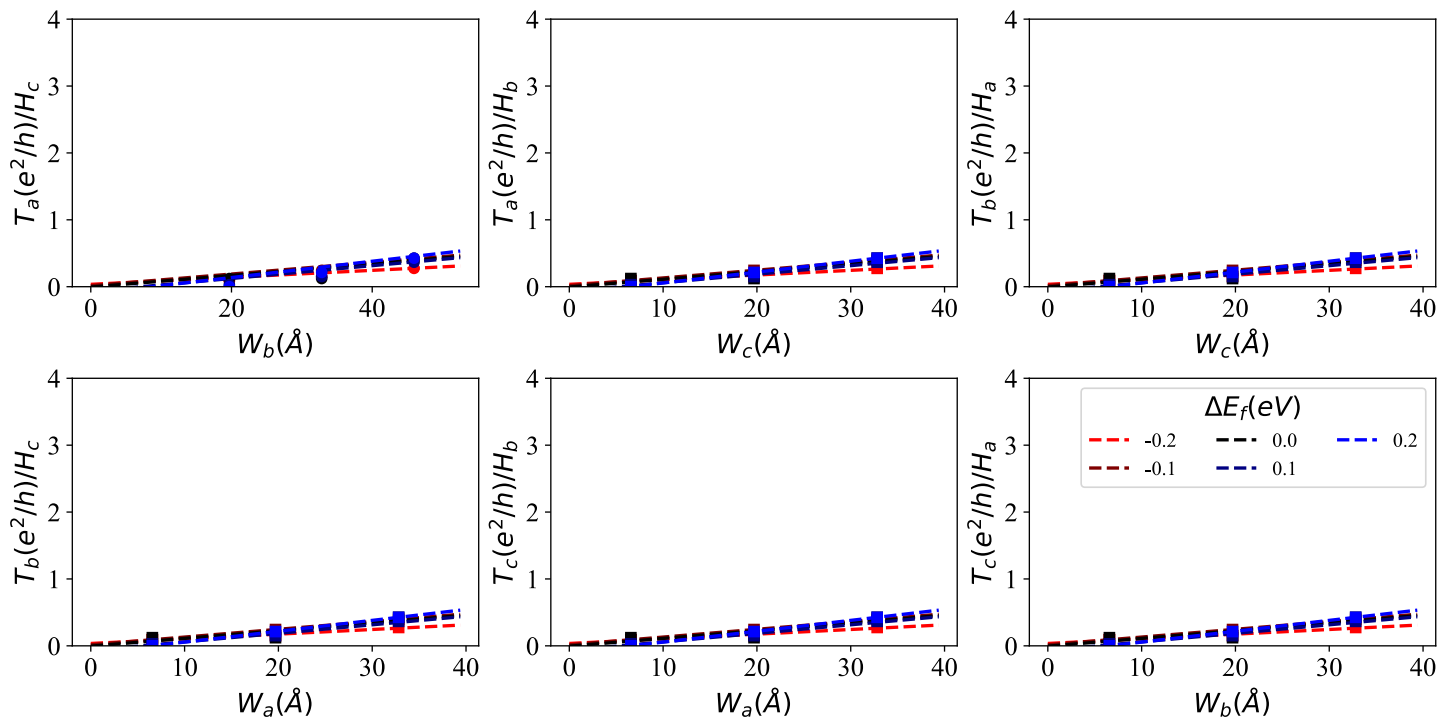



Compound: SrSnHg  
Materials Project ID: 1019259

Lattice (conventional cell):

| Parameter        | Value    | Unit |
|------------------|----------|------|
| a                | 5.0060   | Å    |
| b                | 5.0060   | Å    |
| c                | 8.3087   | Å    |
| $\alpha$ (alpha) | 90.0000  | °    |
| $\beta$ (beta)   | 90.0000  | °    |
| $\gamma$ (gamma) | 120.0000 | °    |

Crystal structure (conventional cell):

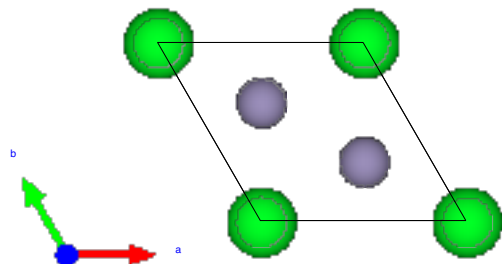

Nanowire Transmission:

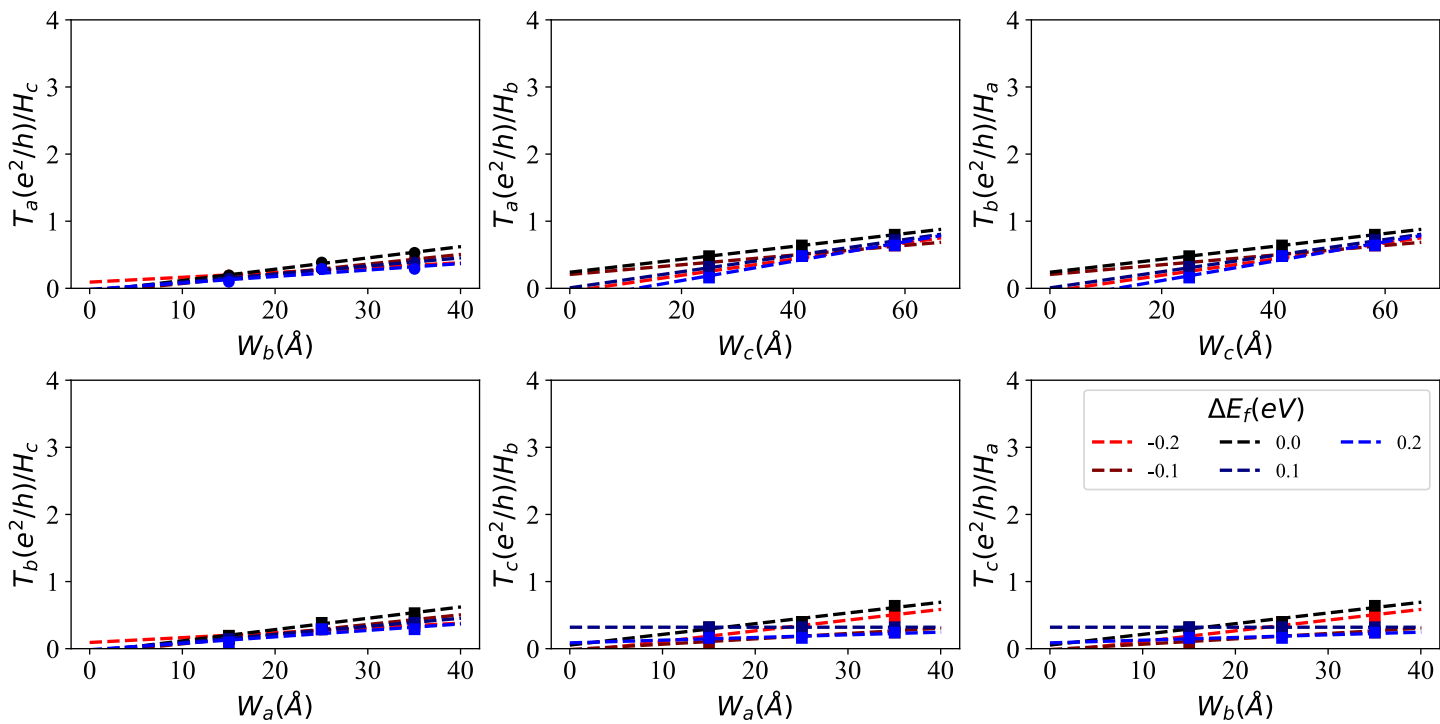

Compound: TaAs  
Materials Project ID: 1936

Lattice (conventional cell):

| Parameter        | Value   | Unit |
|------------------|---------|------|
| a                | 3.4696  | Å    |
| b                | 3.4696  | Å    |
| c                | 11.7349 | Å    |
| $\alpha$ (alpha) | 90.0000 | °    |
| $\beta$ (beta)   | 90.0000 | °    |
| $\gamma$ (gamma) | 90.0000 | °    |

Crystal structure (conventional cell):

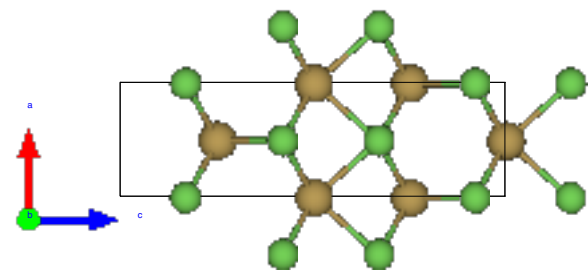

Nanowire Transmission:

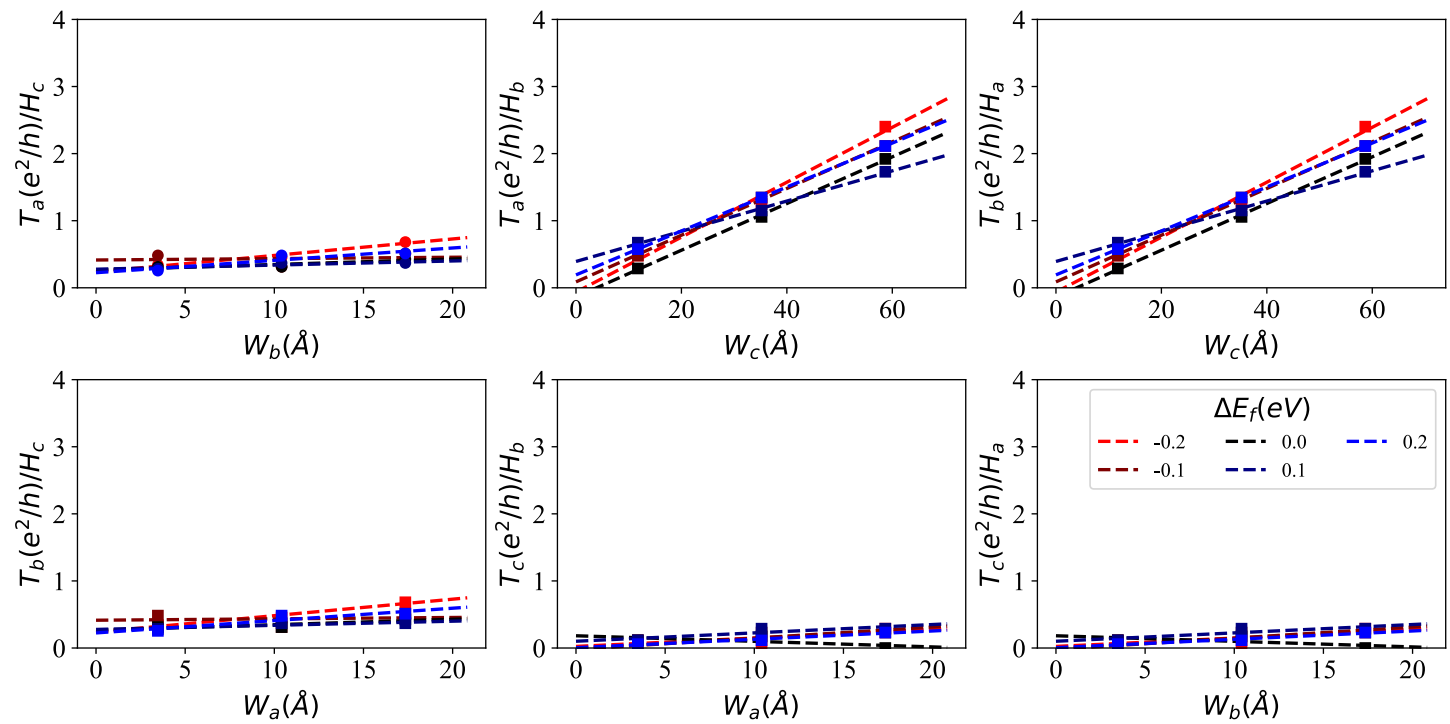

Compound: TaAs<sub>2</sub>  
Materials Project ID: 12561

Lattice (conventional cell):

| Parameter | Value    | Unit |
|-----------|----------|------|
| a         | 9.4399   | Å    |
| b         | 3.4259   | Å    |
| c         | 7.8478   | Å    |
| α (alpha) | 90.0000  | °    |
| β (beta)  | 119.7016 | °    |
| γ (gamma) | 90.0000  | °    |

Crystal structure (conventional cell):

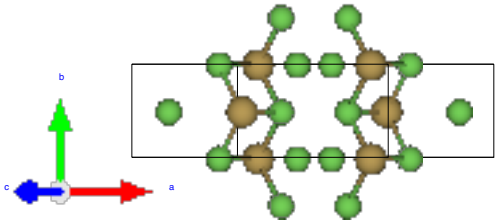

Nanowire Transmission:

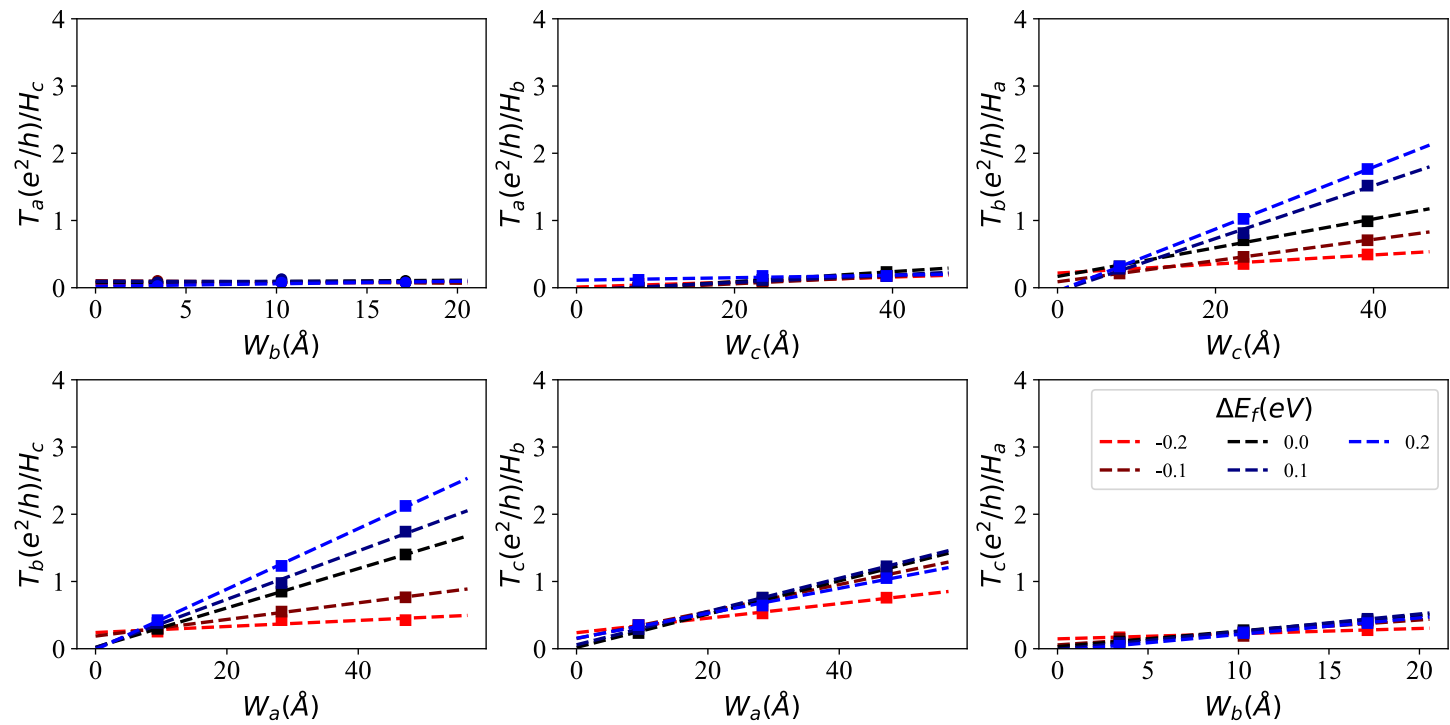

Compound: TaInS<sub>2</sub>  
Materials Project ID: 22332

Lattice (conventional cell):

| Parameter        | Value    | Unit |
|------------------|----------|------|
| a                | 3.3249   | Å    |
| b                | 3.3249   | Å    |
| c                | 8.9364   | Å    |
| $\alpha$ (alpha) | 90.0000  | °    |
| $\beta$ (beta)   | 90.0000  | °    |
| $\gamma$ (gamma) | 120.0000 | °    |

Crystal structure (conventional cell):

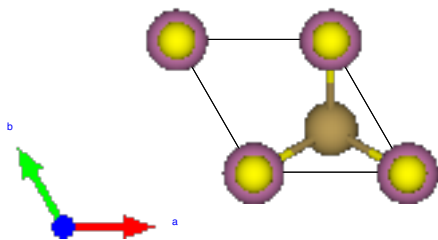

Nanowire Transmission:

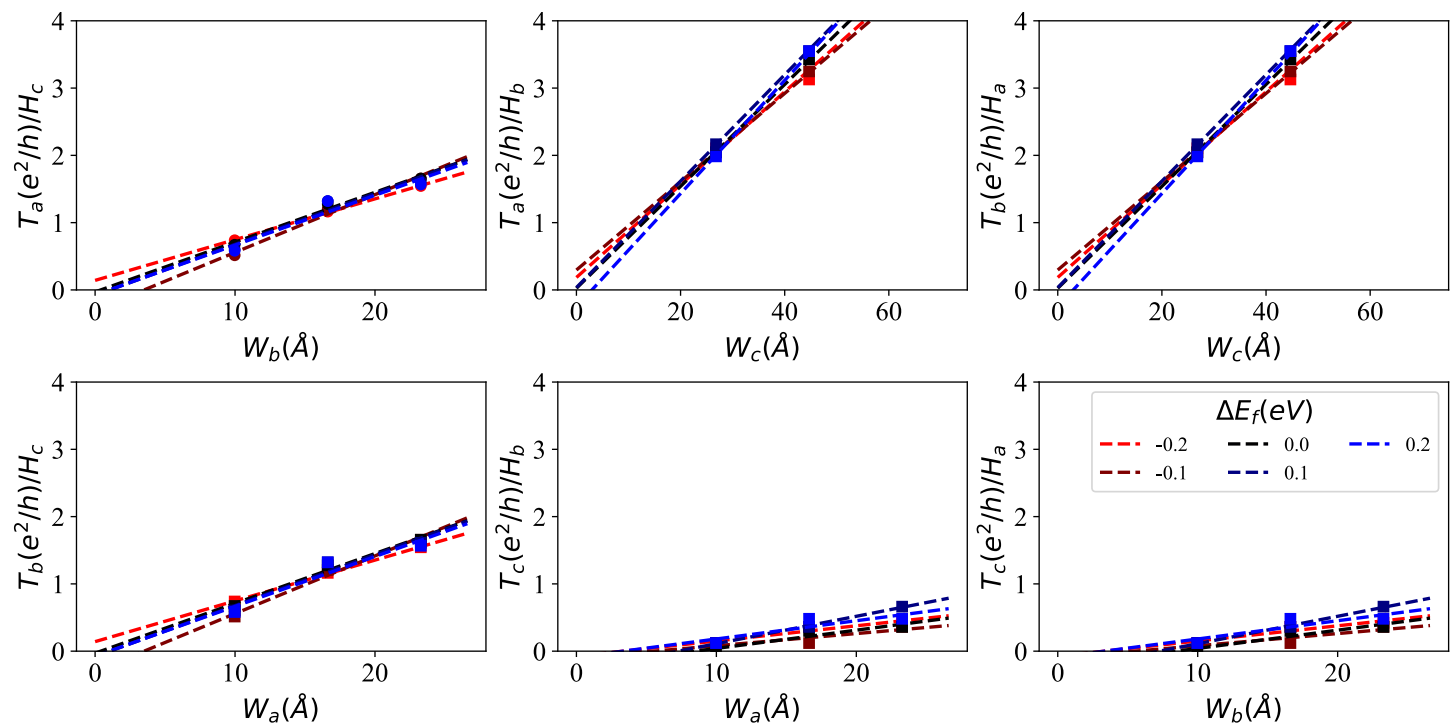

Compound: TaN  
Materials Project ID: 1459

Lattice (conventional cell):

| Parameter        | Value    | Unit |
|------------------|----------|------|
| a                | 2.9540   | Å    |
| b                | 2.9540   | Å    |
| c                | 2.9015   | Å    |
| $\alpha$ (alpha) | 90.0000  | °    |
| $\beta$ (beta)   | 90.0000  | °    |
| $\gamma$ (gamma) | 120.0000 | °    |

Crystal structure (conventional cell):

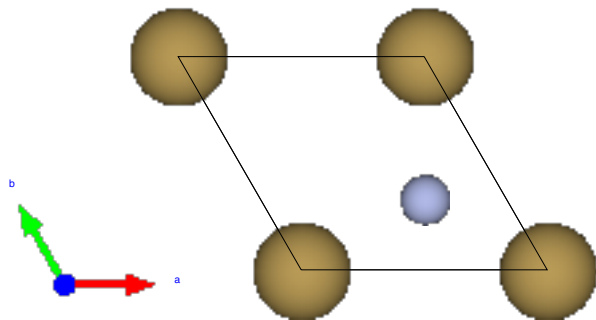

Nanowire Transmission:

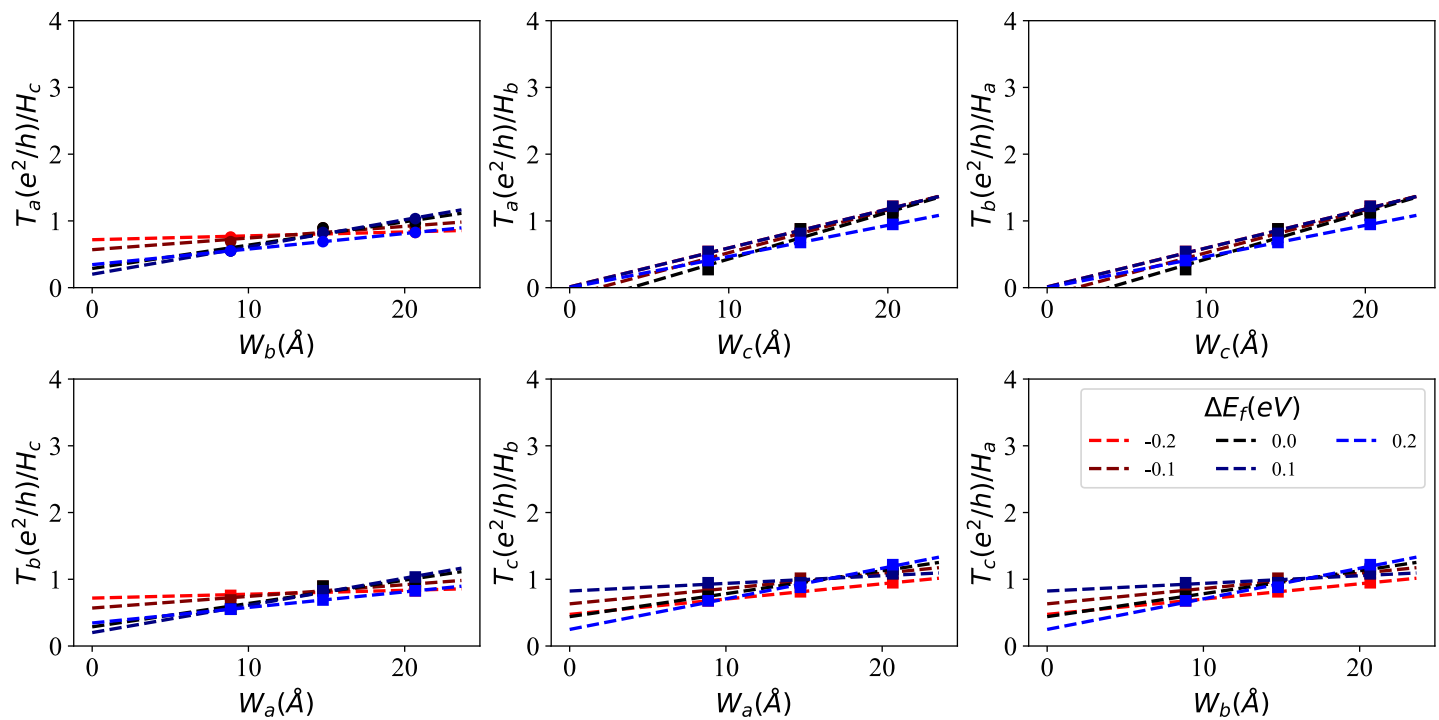

Compound: TaP  
Materials Project ID: 1067587

Lattice (conventional cell):

| Parameter        | Value   | Unit |
|------------------|---------|------|
| a                | 3.3402  | Å    |
| b                | 3.3402  | Å    |
| c                | 11.4036 | Å    |
| $\alpha$ (alpha) | 90.0000 | °    |
| $\beta$ (beta)   | 90.0000 | °    |
| $\gamma$ (gamma) | 90.0000 | °    |

Crystal structure (conventional cell):

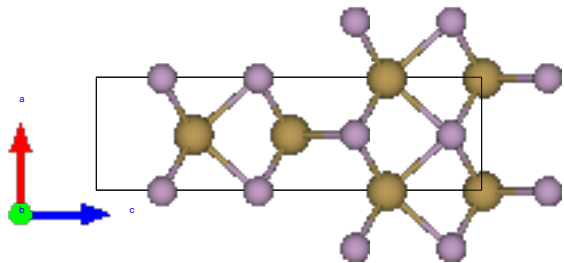

Nanowire Transmission:

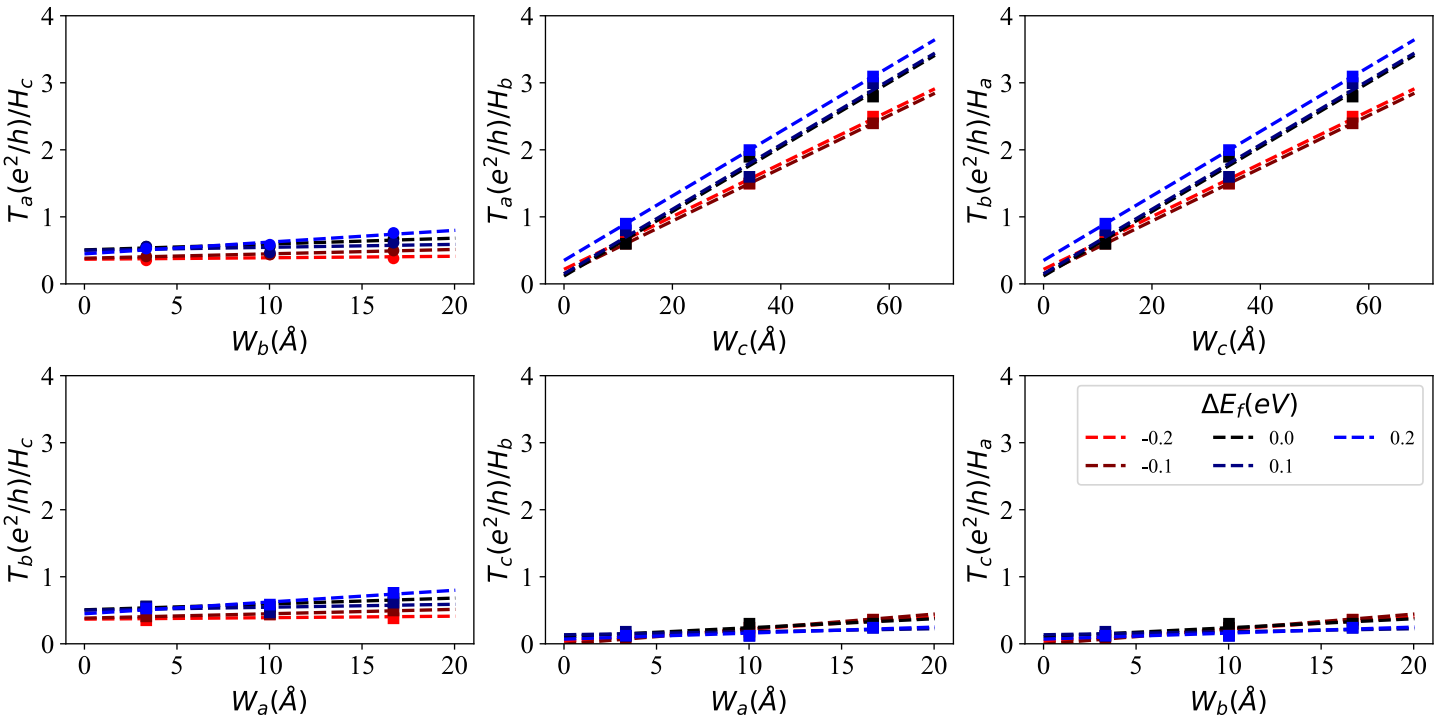

Compound: TaPbSe<sub>2</sub>  
Materials Project ID: 567736

Lattice (conventional cell):

| Parameter        | Value    | Unit |
|------------------|----------|------|
| a                | 3.4835   | Å    |
| b                | 3.4835   | Å    |
| c                | 9.4755   | Å    |
| $\alpha$ (alpha) | 90.0000  | °    |
| $\beta$ (beta)   | 90.0000  | °    |
| $\gamma$ (gamma) | 120.0000 | °    |

Crystal structure (conventional cell):

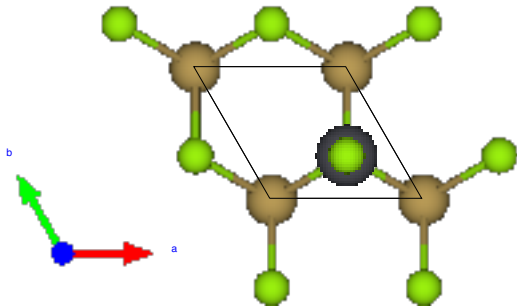

Nanowire Transmission:

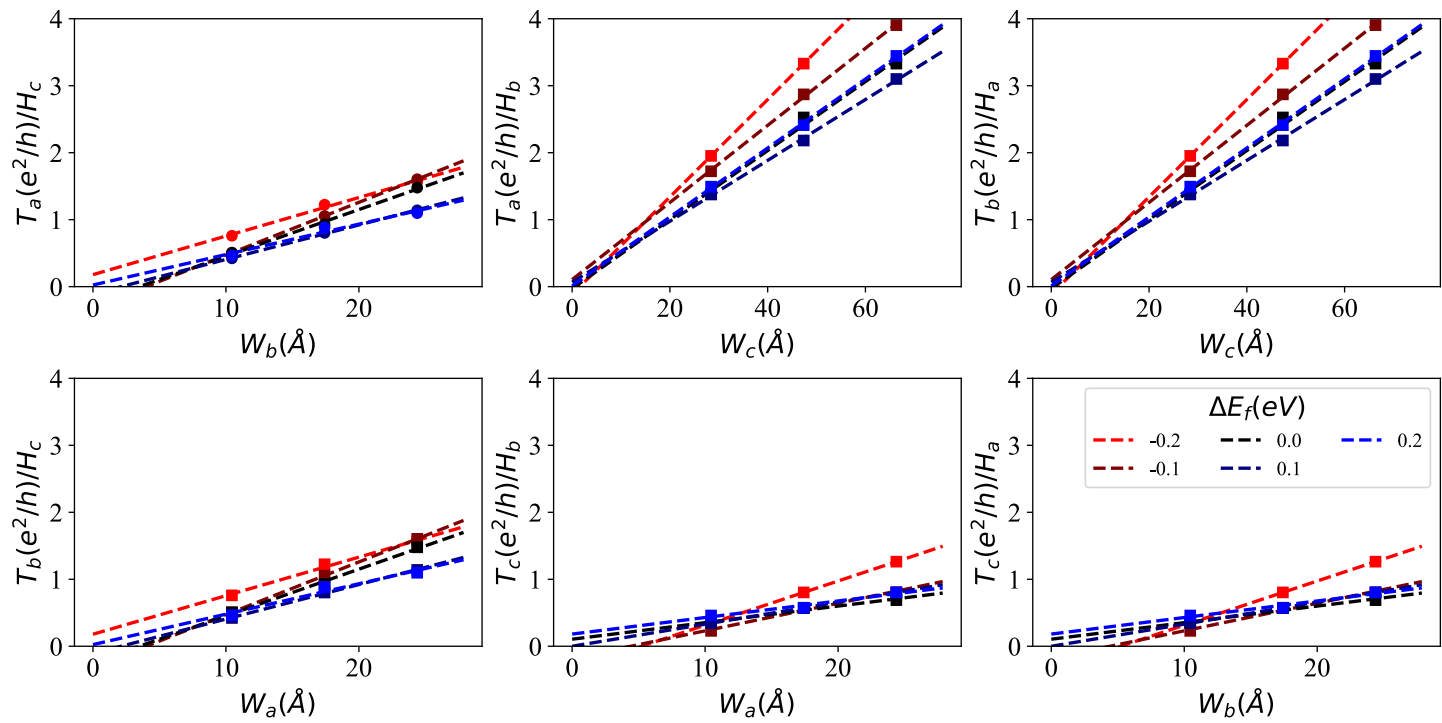

Compound: TaSiAs  
Materials Project ID: 81

Lattice (conventional cell):

| Parameter        | Value   | Unit |
|------------------|---------|------|
| a                | 3.5206  | Å    |
| b                | 3.5206  | Å    |
| c                | 7.9142  | Å    |
| $\alpha$ (alpha) | 90.0000 | °    |
| $\beta$ (beta)   | 90.0000 | °    |
| $\gamma$ (gamma) | 90.0000 | °    |

Crystal structure (conventional cell):

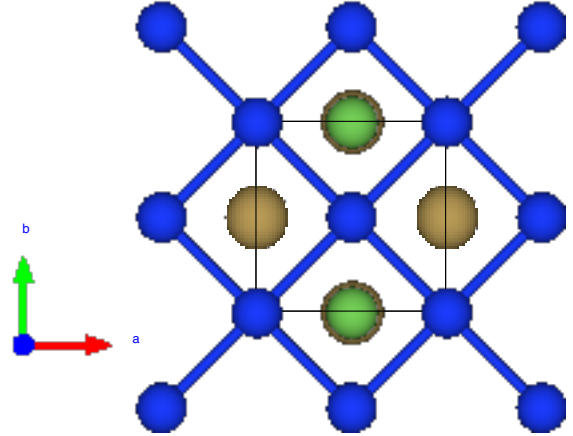

Nanowire Transmission:

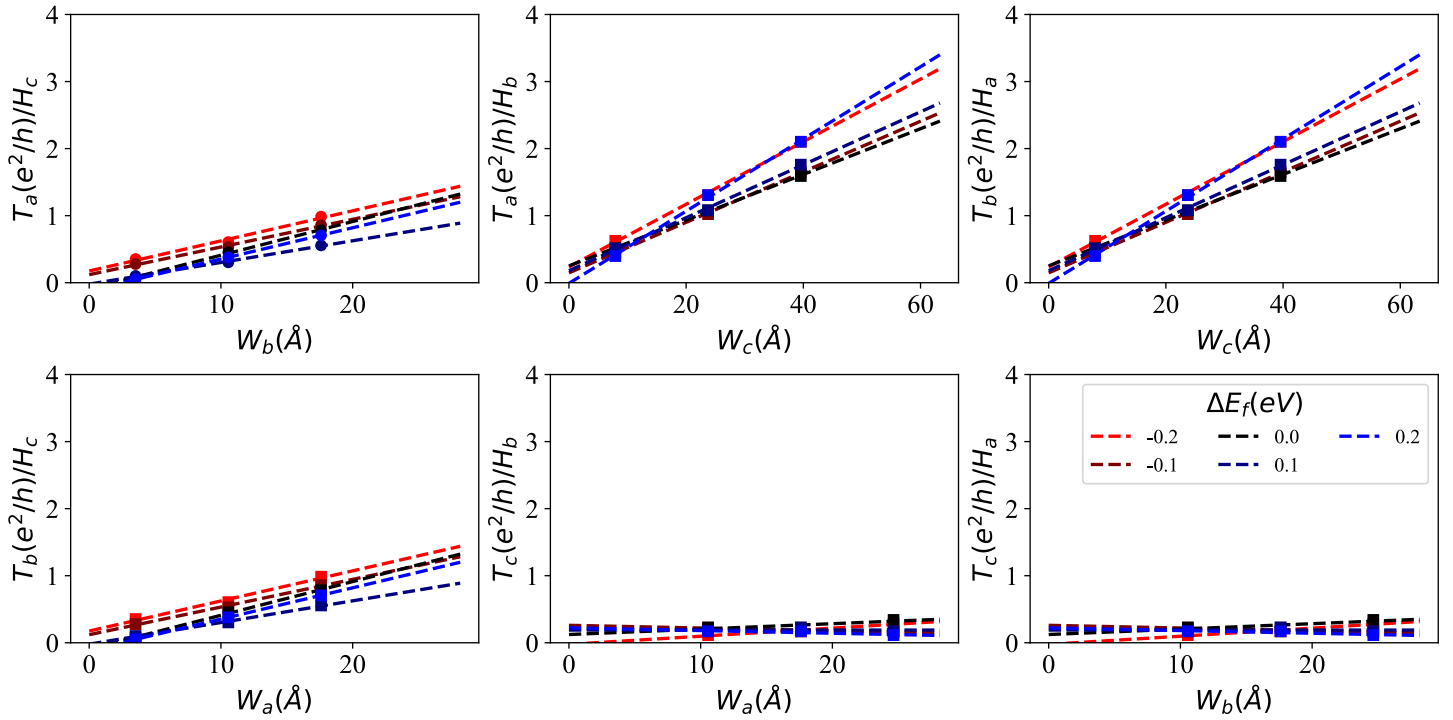



Compound: Te  
Materials Project ID: 19

Lattice (conventional cell):

| Parameter        | Value    | Unit |
|------------------|----------|------|
| a                | 4.5124   | Å    |
| b                | 4.5124   | Å    |
| c                | 5.9599   | Å    |
| $\alpha$ (alpha) | 90.0000  | °    |
| $\beta$ (beta)   | 90.0000  | °    |
| $\gamma$ (gamma) | 120.0000 | °    |

Crystal structure (conventional cell):

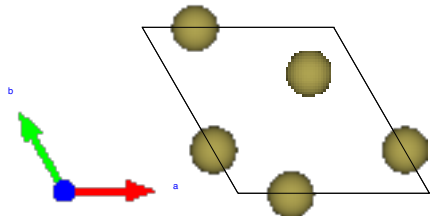

Nanowire Transmission:

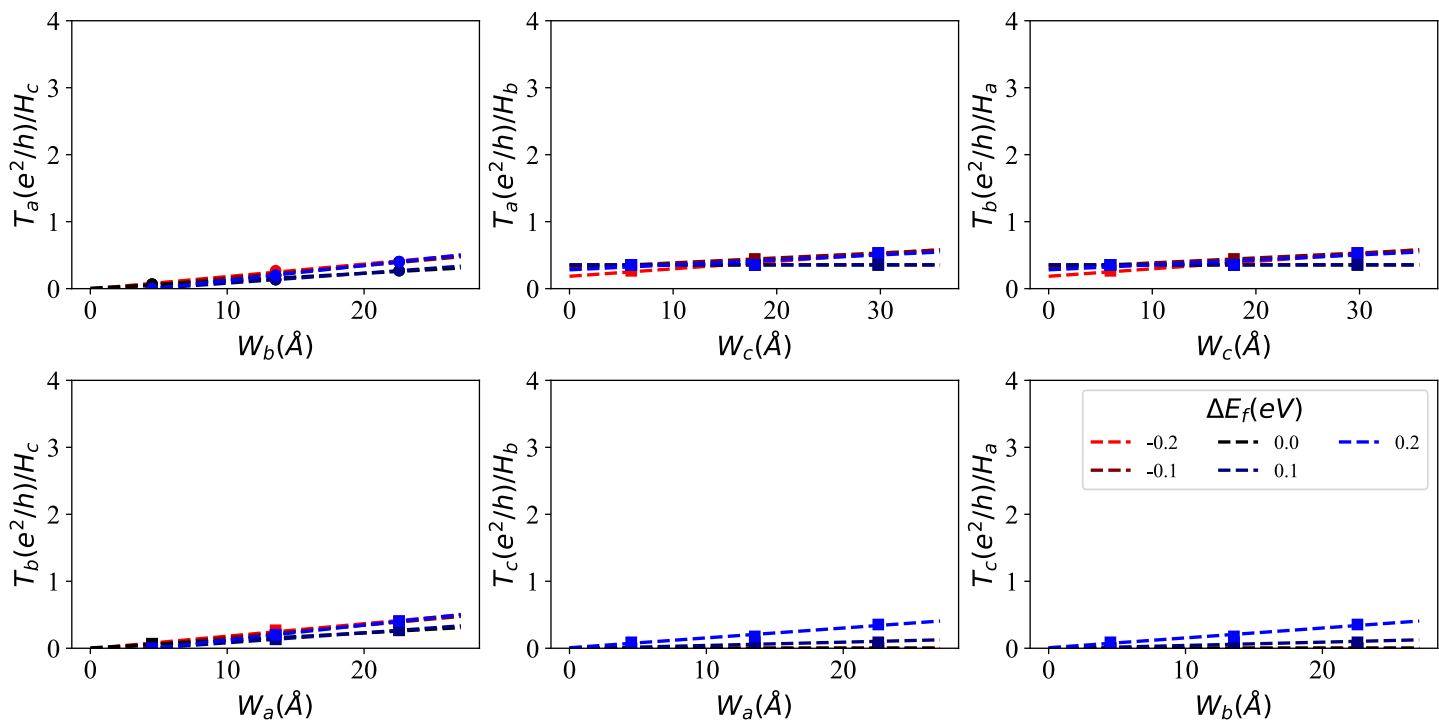

Compound: Te<sub>2</sub>Ir  
Materials Project ID: 2285

Lattice (conventional cell):

| Parameter        | Value    | Unit |
|------------------|----------|------|
| a                | 3.9878   | Å    |
| b                | 3.9878   | Å    |
| c                | 5.5433   | Å    |
| $\alpha$ (alpha) | 90.0000  | °    |
| $\beta$ (beta)   | 90.0000  | °    |
| $\gamma$ (gamma) | 120.0000 | °    |

Crystal structure (conventional cell):

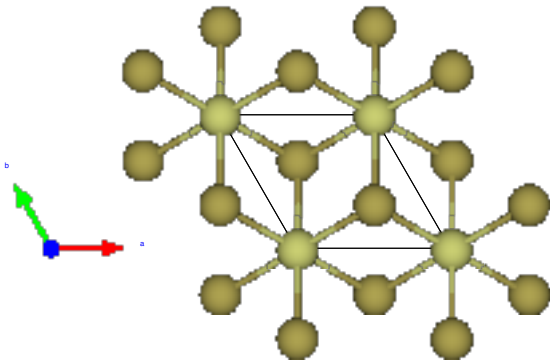

Nanowire Transmission:

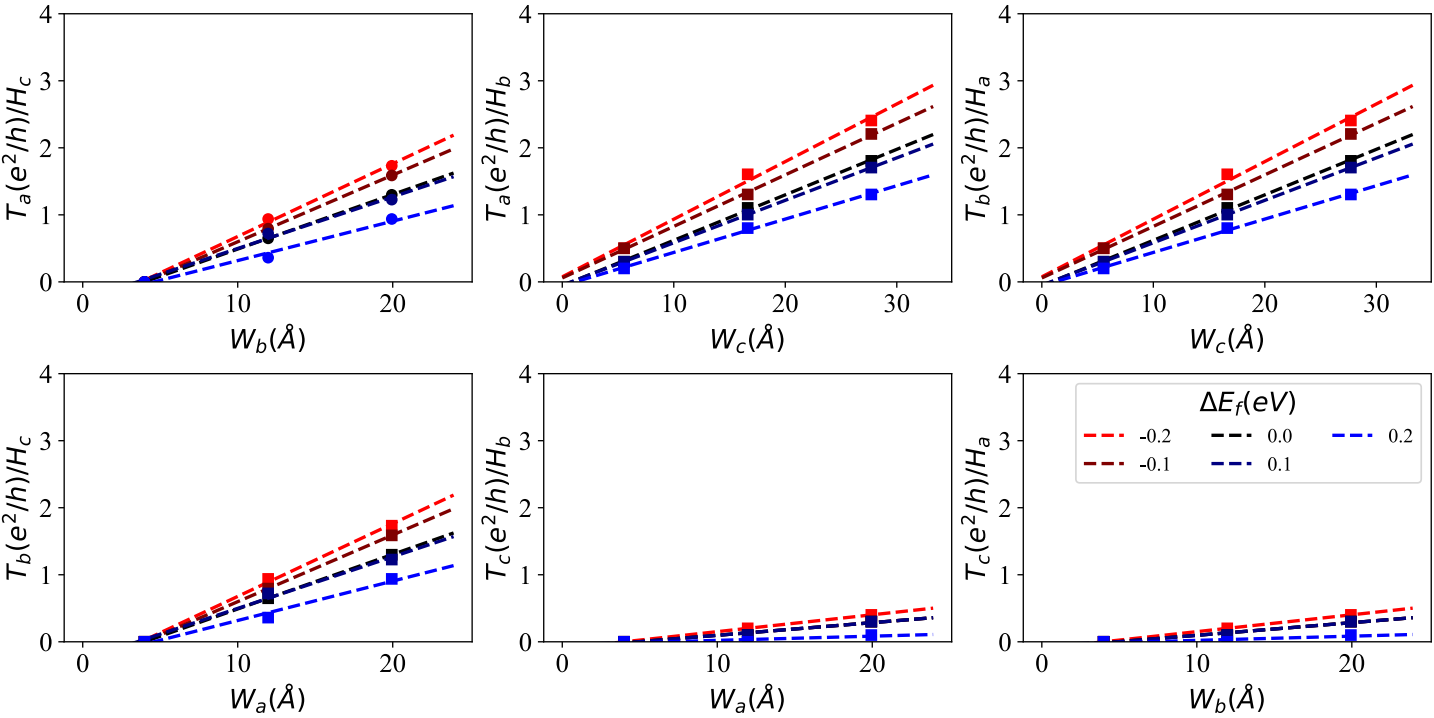

Compound:  $\text{Te}_2\text{Mo}$   
Materials Project ID: 7459

Lattice (conventional cell):

| Parameter        | Value   | Unit |
|------------------|---------|------|
| a                | 6.3662  | Å    |
| b                | 3.4869  | Å    |
| c                | 15.5479 | Å    |
| $\alpha$ (alpha) | 90.0000 | °    |
| $\beta$ (beta)   | 92.3879 | °    |
| $\gamma$ (gamma) | 90.0000 | °    |

Crystal structure (conventional cell):

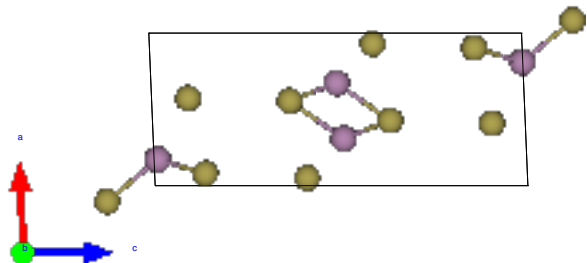

Nanowire Transmission:

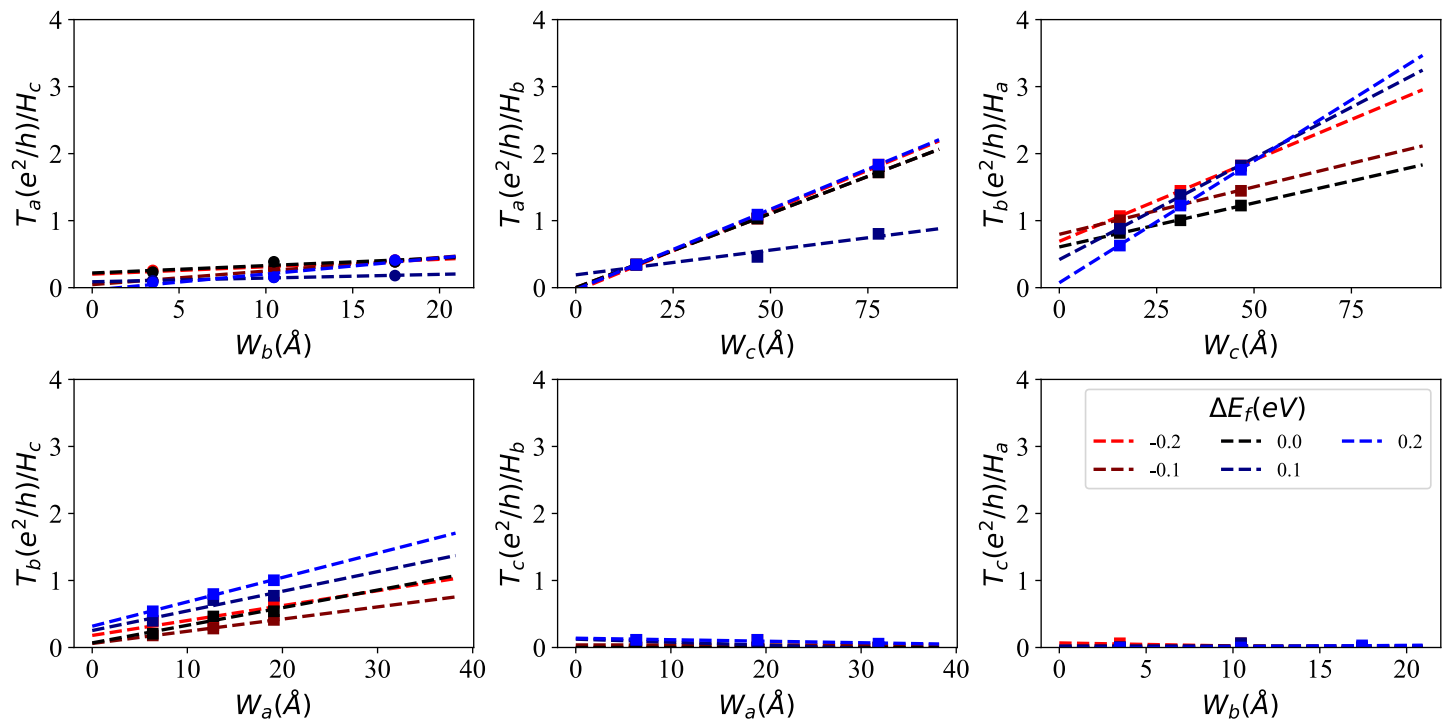

Compound:  $\text{Te}_2\text{W}$   
Materials Project ID:22693

Lattice (conventional cell):

| Parameter        | Value   | Unit |
|------------------|---------|------|
| a                | 3.4979  | Å    |
| b                | 6.3383  | Å    |
| c                | 15.4319 | Å    |
| $\alpha$ (alpha) | 90.0000 | °    |
| $\beta$ (beta)   | 90.0000 | °    |
| $\gamma$ (gamma) | 90.0000 | °    |

Crystal structure (conventional cell):

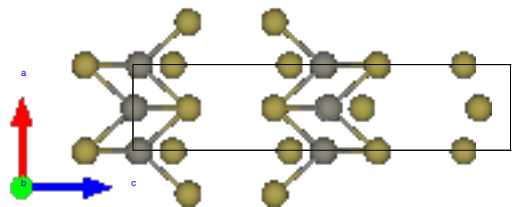

Nanowire Transmission:

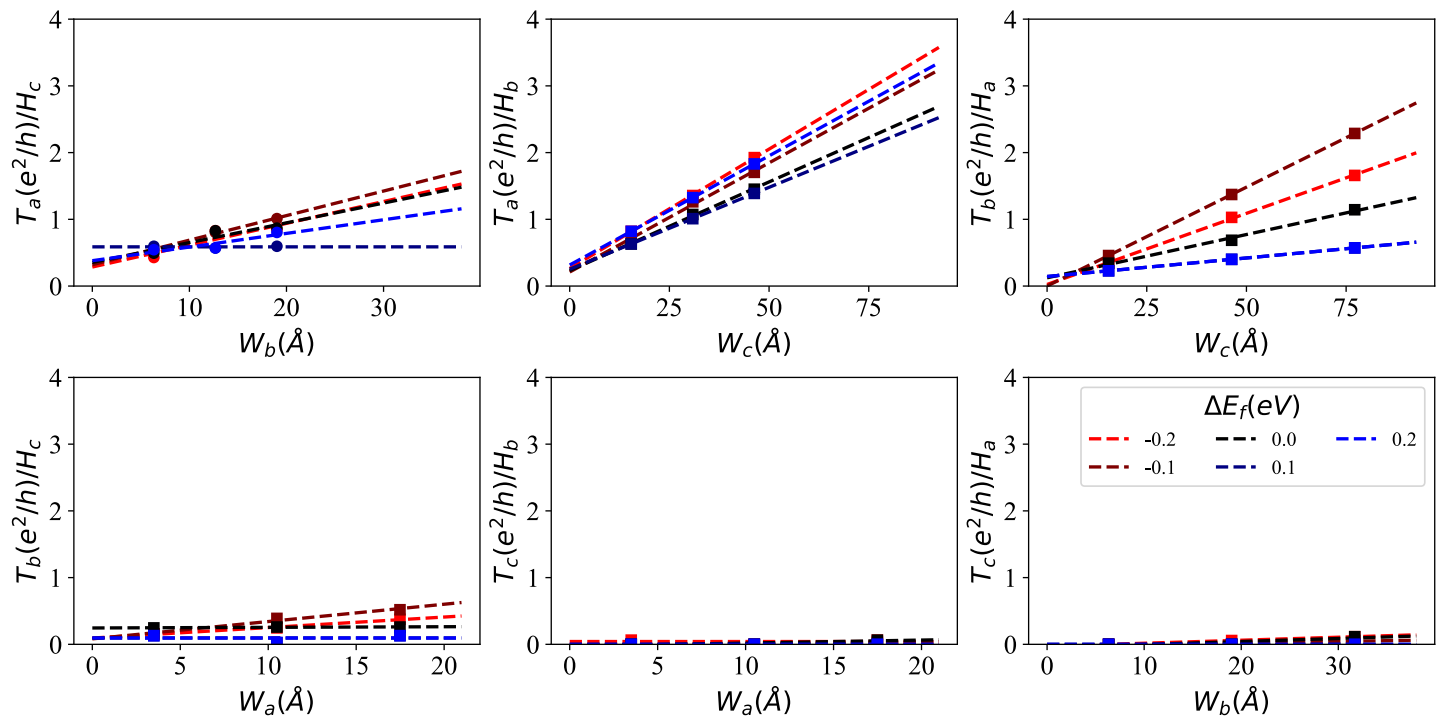

Compound:  $\text{TiB}_2$   
Materials Project ID: 1145

Lattice (conventional cell):

| Parameter        | Value    | Unit |
|------------------|----------|------|
| a                | 3.0351   | Å    |
| b                | 3.0351   | Å    |
| c                | 3.2232   | Å    |
| $\alpha$ (alpha) | 90.0000  | °    |
| $\beta$ (beta)   | 90.0000  | °    |
| $\gamma$ (gamma) | 120.0000 | °    |

Crystal structure (conventional cell):

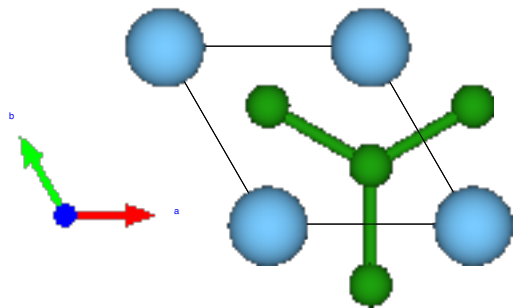

Nanowire Transmission:

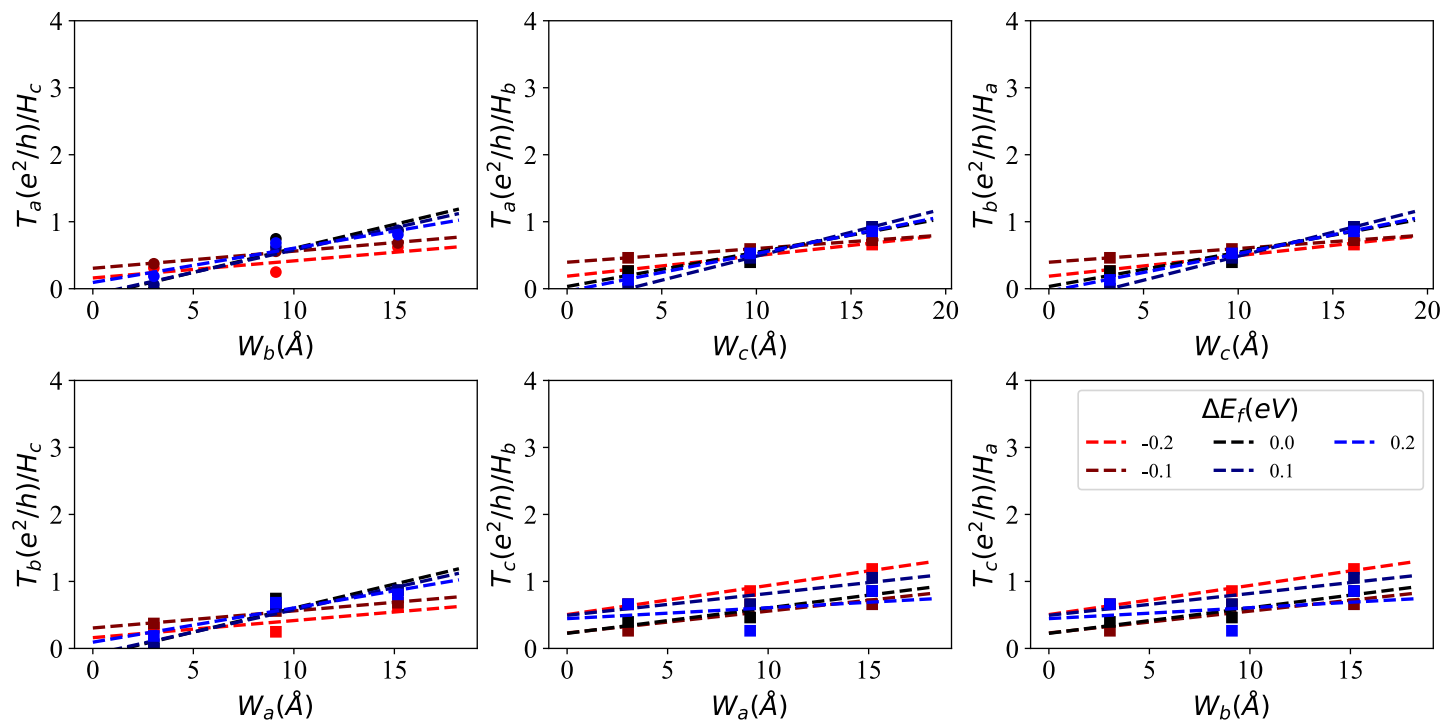

Compound:  $\text{TiCu}_2$   
Materials Project ID: 1077023

Lattice (conventional cell):

| Parameter        | Value   | Unit |
|------------------|---------|------|
| a                | 4.5123  | Å    |
| b                | 7.9862  | Å    |
| c                | 4.4641  | Å    |
| $\alpha$ (alpha) | 90.0000 | °    |
| $\beta$ (beta)   | 90.0000 | °    |
| $\gamma$ (gamma) | 90.0000 | °    |

Crystal structure (conventional cell):

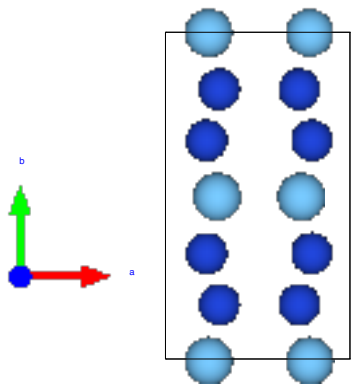

Nanowire Transmission:

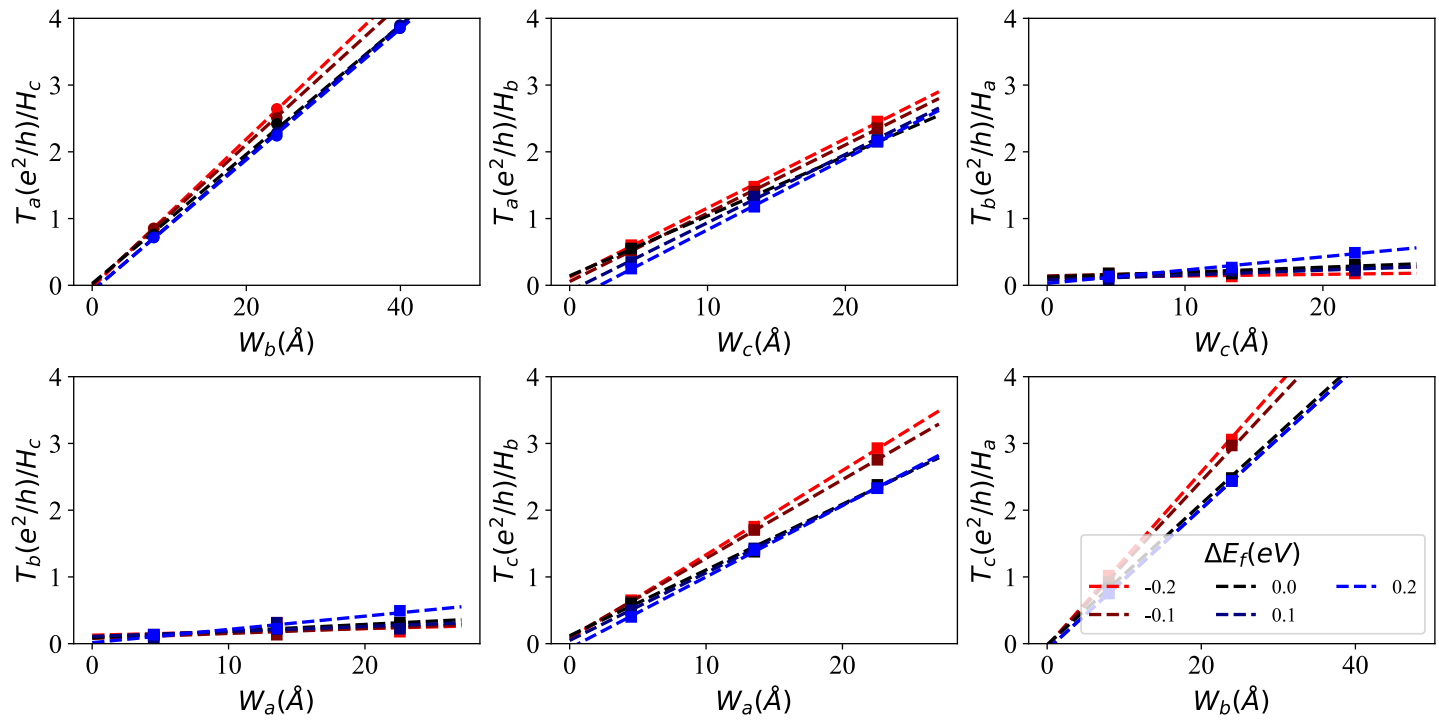

Compound: TiS  
Materials Project ID: 1018028

Lattice (conventional cell):

| Parameter        | Value    | Unit |
|------------------|----------|------|
| a                | 3.2739   | Å    |
| b                | 3.2739   | Å    |
| c                | 3.2191   | Å    |
| $\alpha$ (alpha) | 90.0000  | °    |
| $\beta$ (beta)   | 90.0000  | °    |
| $\gamma$ (gamma) | 120.0000 | °    |

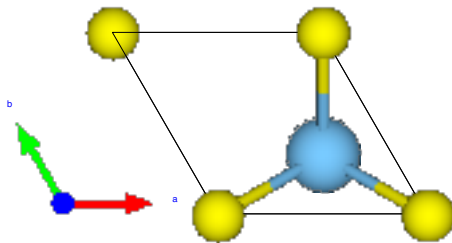

Nanowire Transmission:

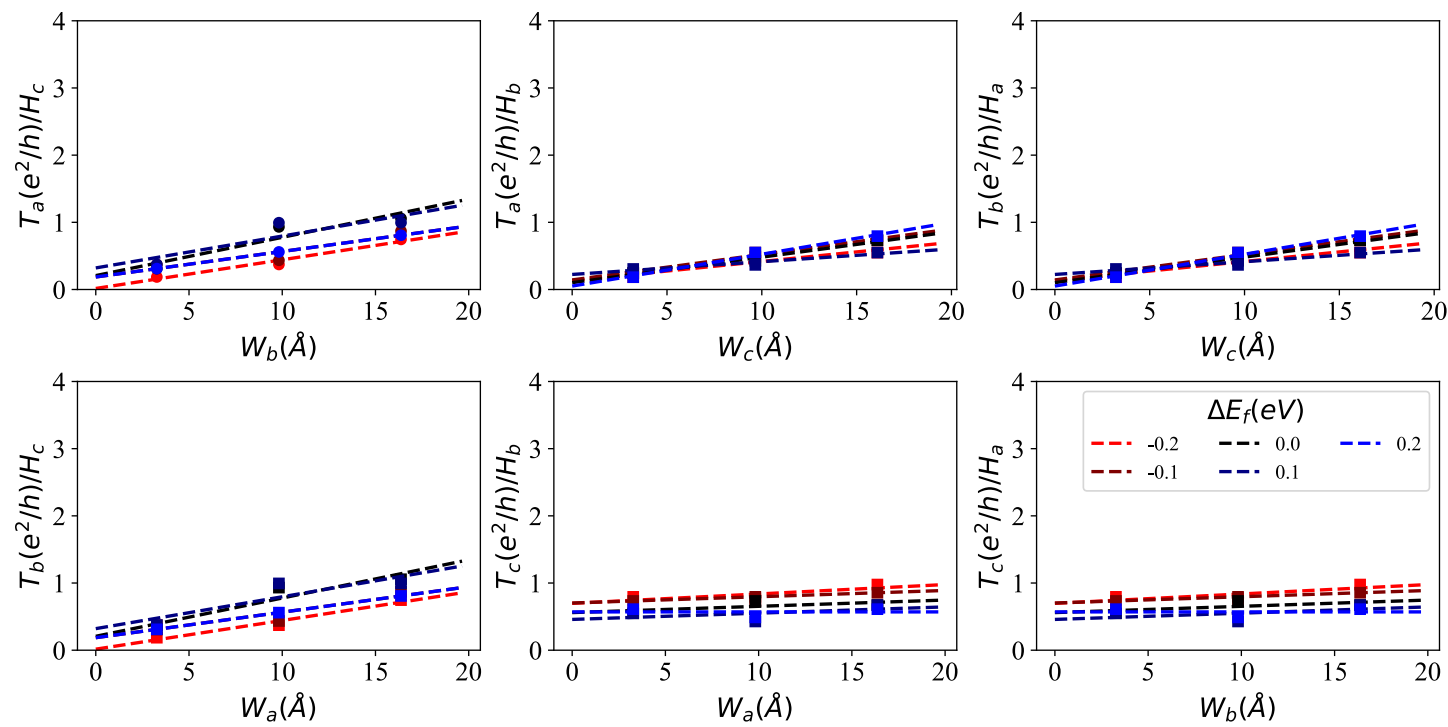

Compound: WC  
Materials Project ID: 1894

Lattice (conventional cell):

| Parameter        | Value    | Unit |
|------------------|----------|------|
| a                | 2.9283   | Å    |
| b                | 2.9283   | Å    |
| c                | 2.8529   | Å    |
| $\alpha$ (alpha) | 90.0000  | °    |
| $\beta$ (beta)   | 90.0000  | °    |
| $\gamma$ (gamma) | 120.0000 | °    |

Crystal structure (conventional cell):

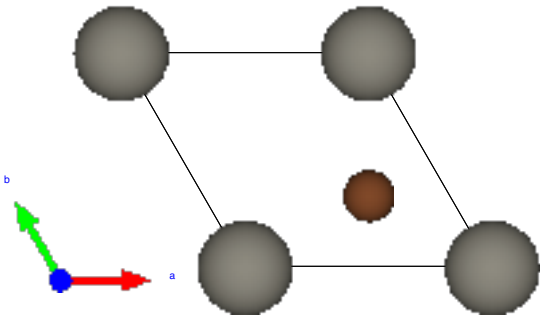

Nanowire Transmission:

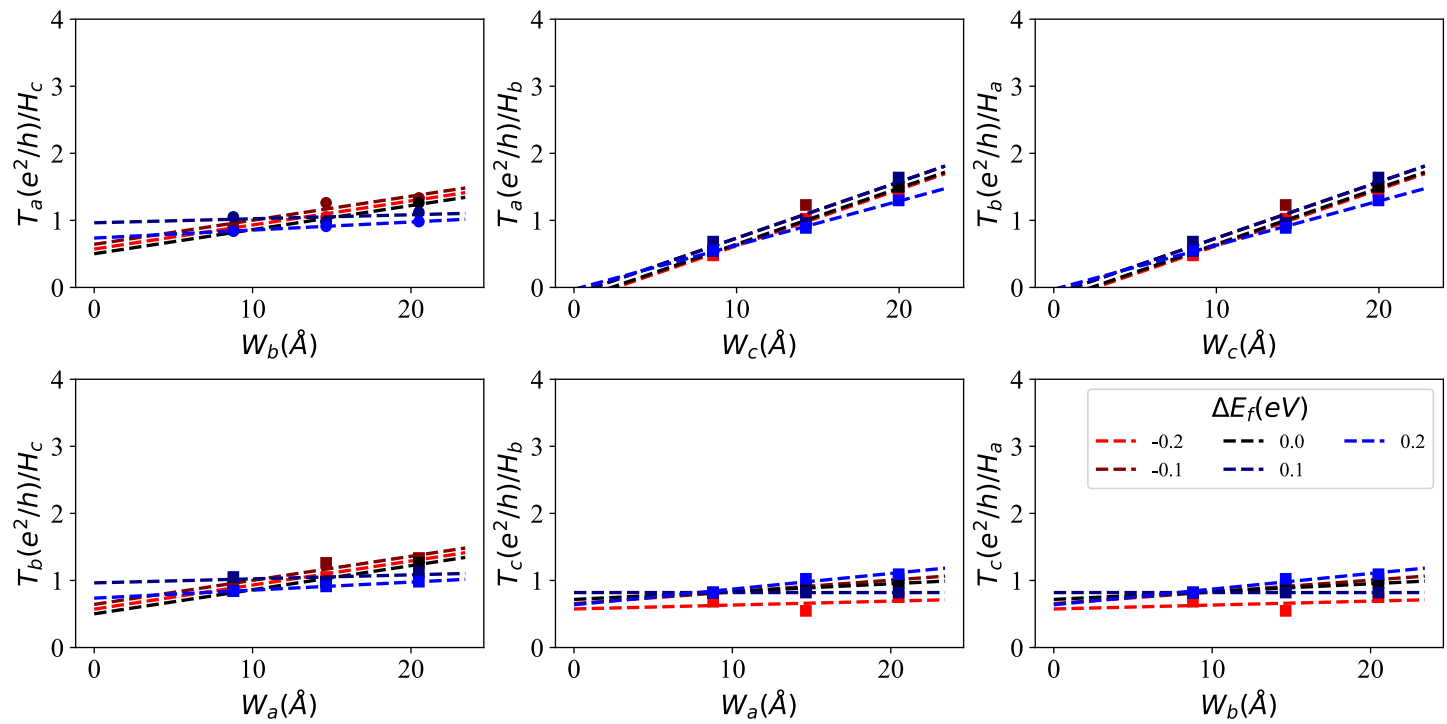



Compound: WN  
Materials Project ID: 991

Lattice (conventional cell):

| Parameter        | Value    | Unit |
|------------------|----------|------|
| a                | 2.8760   | Å    |
| b                | 2.8760   | Å    |
| c                | 2.9080   | Å    |
| $\alpha$ (alpha) | 90.0000  | °    |
| $\beta$ (beta)   | 90.0000  | °    |
| $\gamma$ (gamma) | 120.0000 | °    |

Crystal structure (conventional cell):

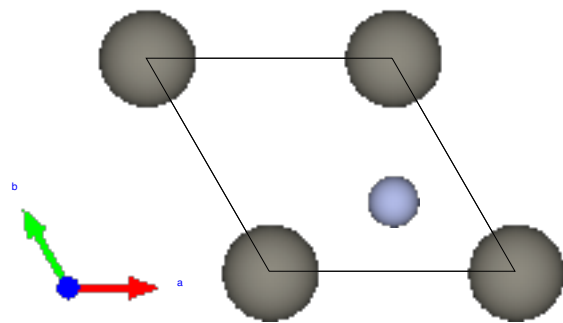

Nanowire Transmission:

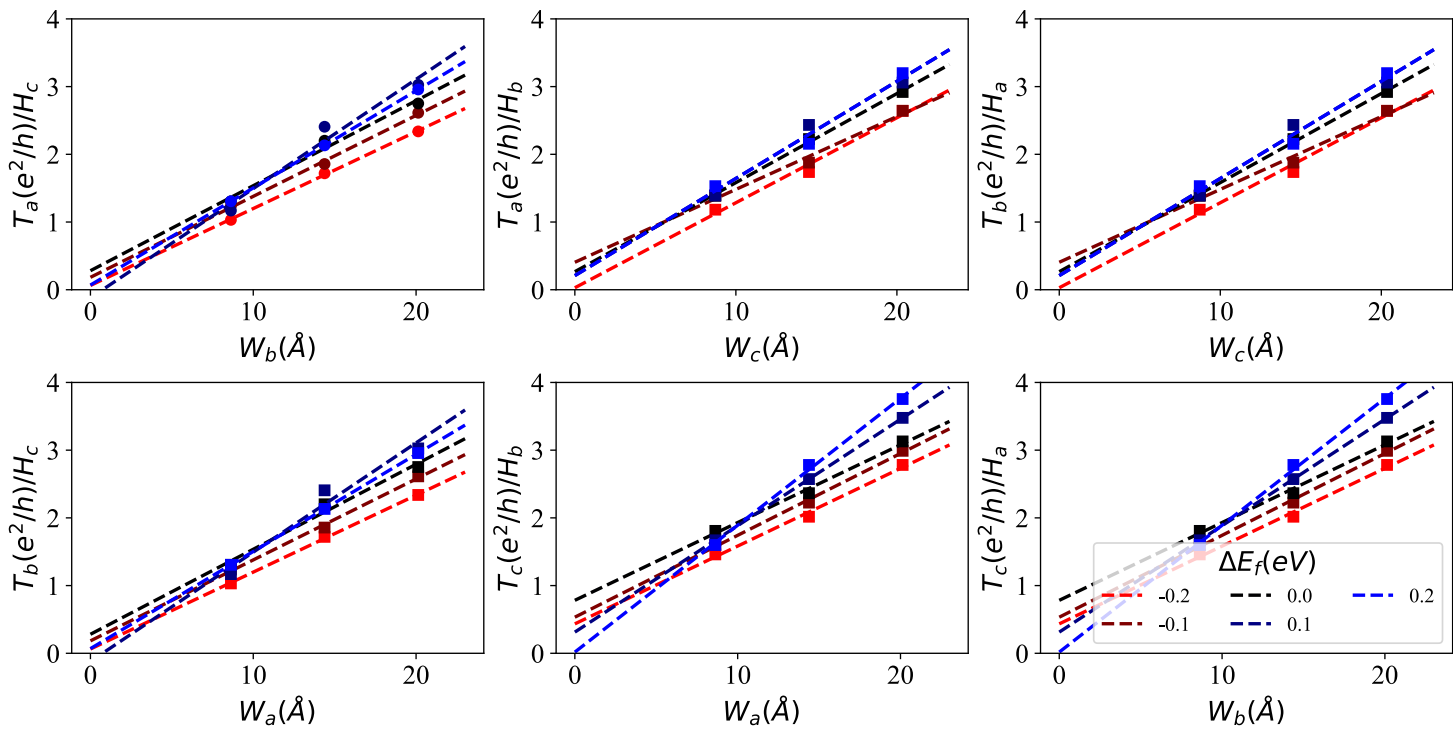

Compound: YAgPb  
Materials Project ID: 21505

Lattice (conventional cell):

| Parameter        | Value    | Unit |
|------------------|----------|------|
| a                | 7.5818   | Å    |
| b                | 7.5818   | Å    |
| c                | 4.5605   | Å    |
| $\alpha$ (alpha) | 90.0000  | °    |
| $\beta$ (beta)   | 90.0000  | °    |
| $\gamma$ (gamma) | 120.0000 | °    |

Crystal structure (conventional cell):

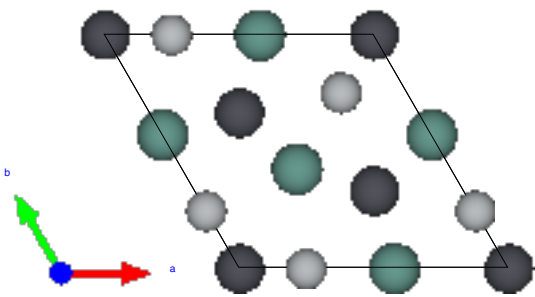

Nanowire Transmission:

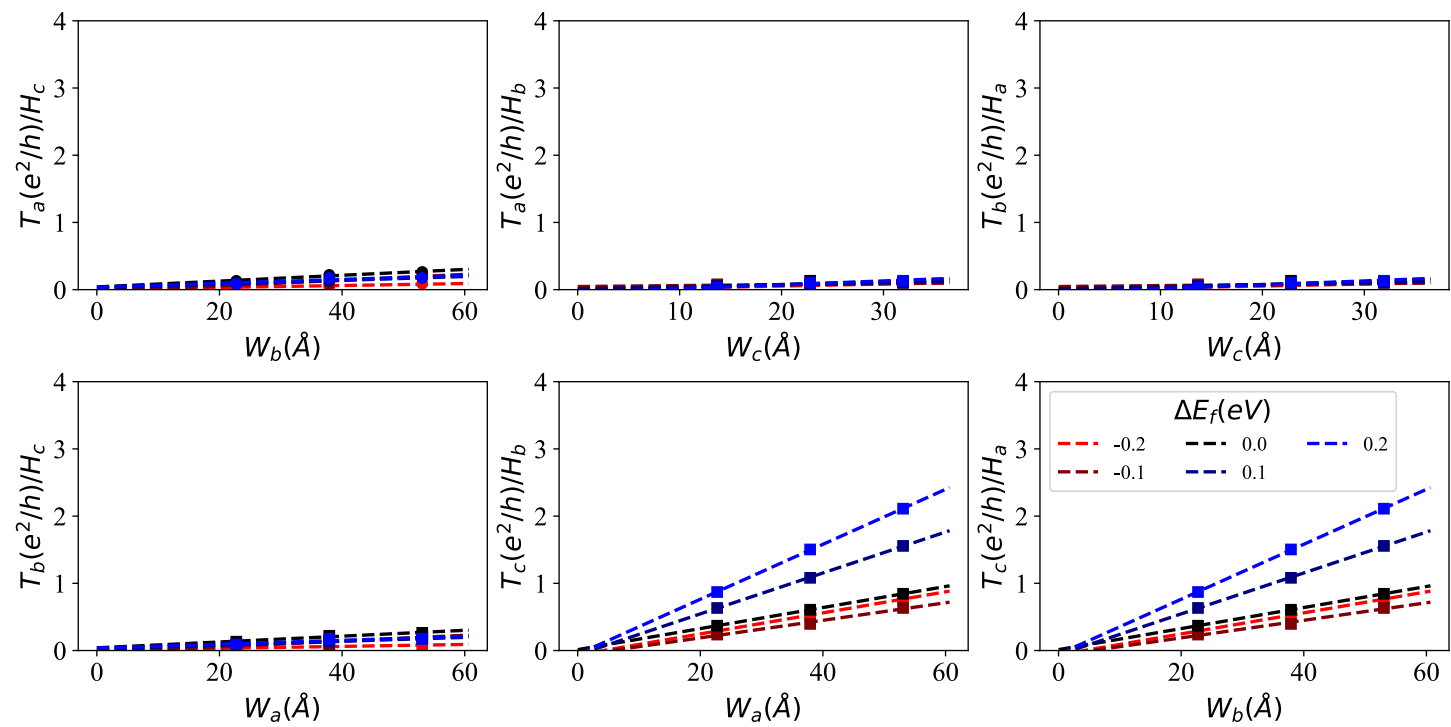

Compound: ZrB<sub>2</sub>  
Materials Project ID: 1472

Lattice (conventional cell):

| Parameter | Value    | Unit |
|-----------|----------|------|
| a         | 3.1805   | Å    |
| b         | 3.1805   | Å    |
| c         | 3.5455   | Å    |
| α (alpha) | 90.0000  | °    |
| β (beta)  | 90.0000  | °    |
| γ (gamma) | 120.0000 | °    |

Crystal structure (conventional cell):

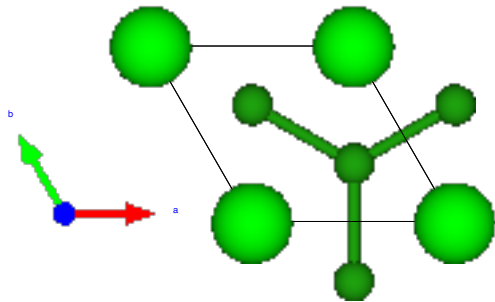

Nanowire Transmission:

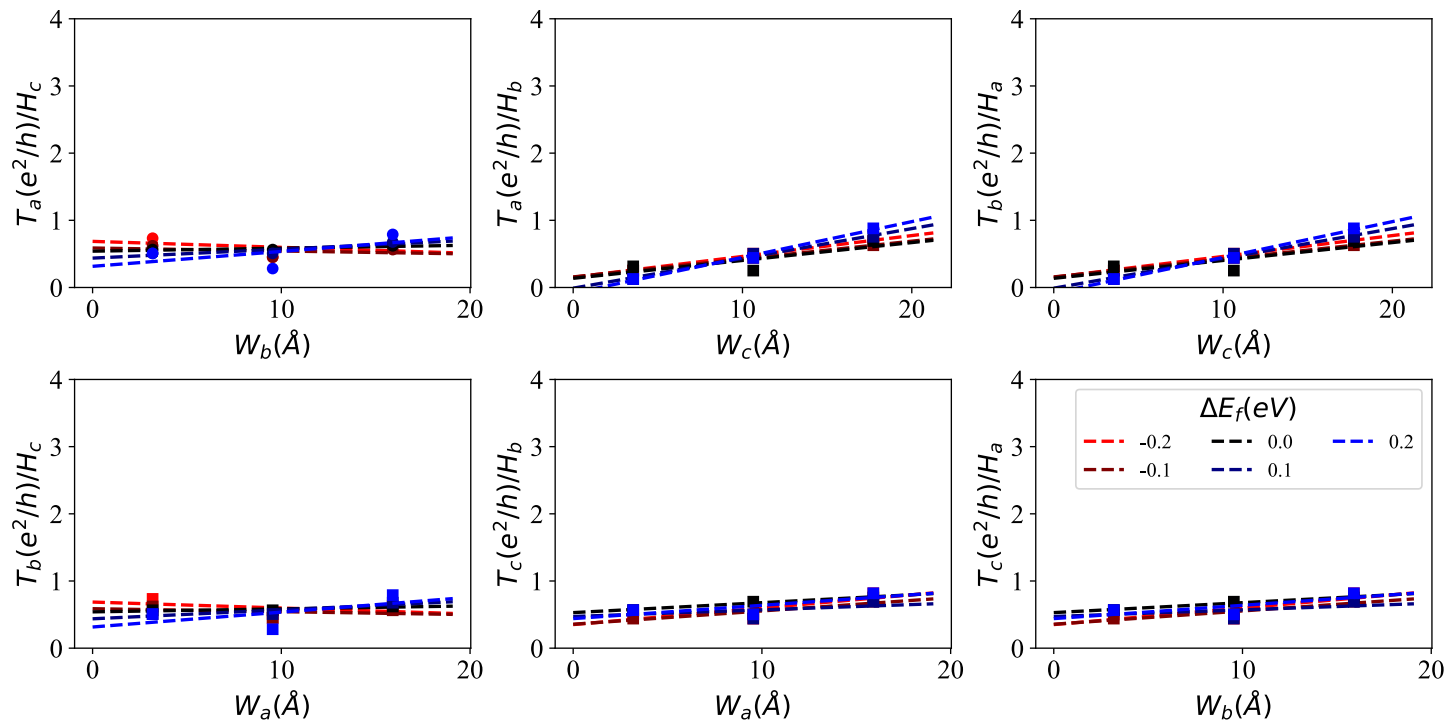

Compound: ZrGePt  
Materials Project ID: 1095610

Lattice (conventional cell):

| Parameter        | Value   | Unit |
|------------------|---------|------|
| a                | 4.0158  | Å    |
| b                | 6.7301  | Å    |
| c                | 7.7560  | Å    |
| $\alpha$ (alpha) | 90.0000 | °    |
| $\beta$ (beta)   | 90.0000 | °    |
| $\gamma$ (gamma) | 90.0000 | °    |

Crystal structure (conventional cell):

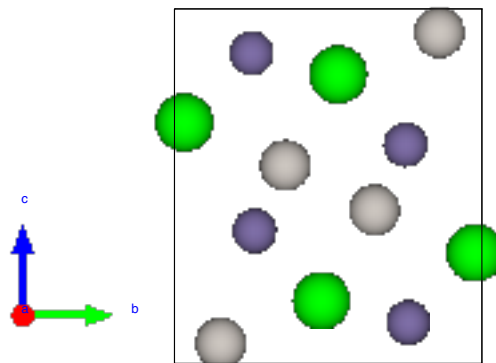

Nanowire Transmission:

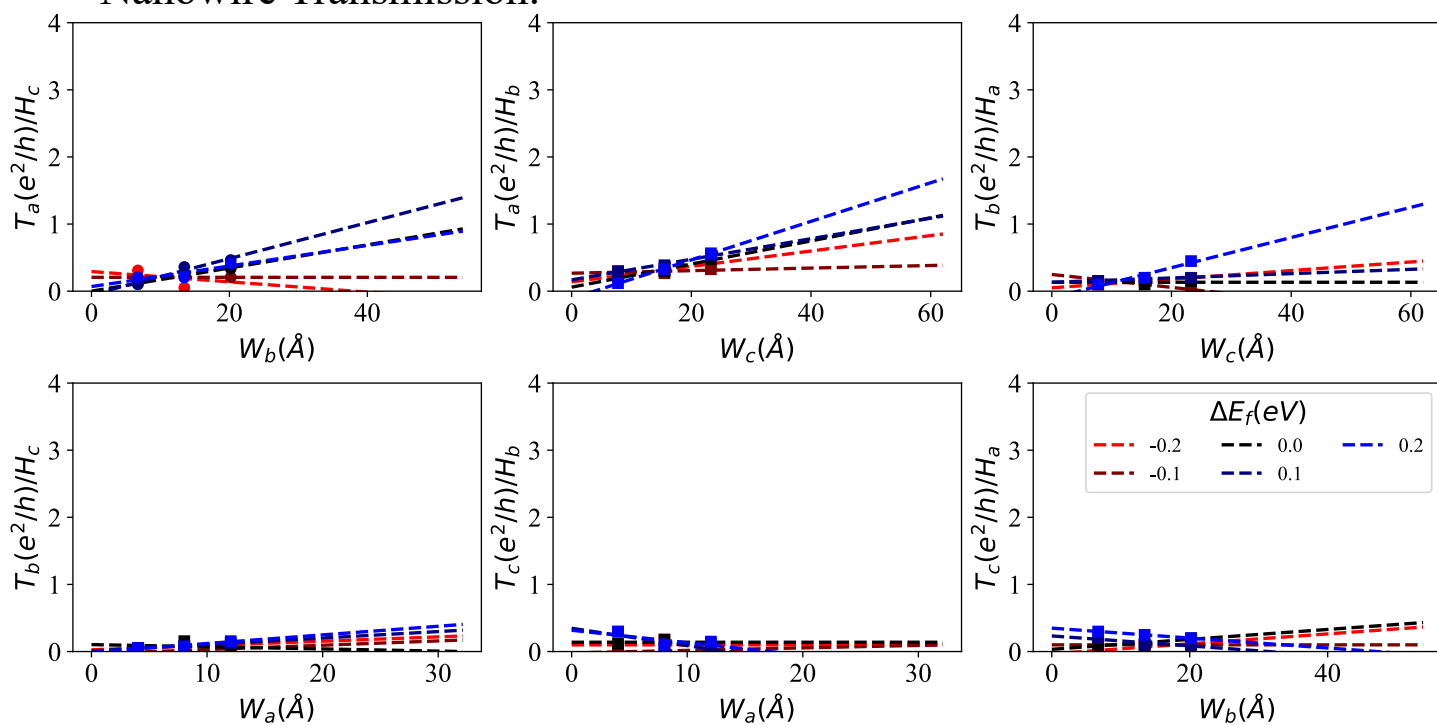

Compound: ZrSiPt  
Materials Project ID: 972187

Lattice (conventional cell):

| Parameter        | Value   | Unit |
|------------------|---------|------|
| a                | 3.9323  | Å    |
| b                | 6.6654  | Å    |
| c                | 7.6233  | Å    |
| $\alpha$ (alpha) | 90.0000 | °    |
| $\beta$ (beta)   | 90.0000 | °    |
| $\gamma$ (gamma) | 90.0000 | °    |

Crystal structure (conventional cell):

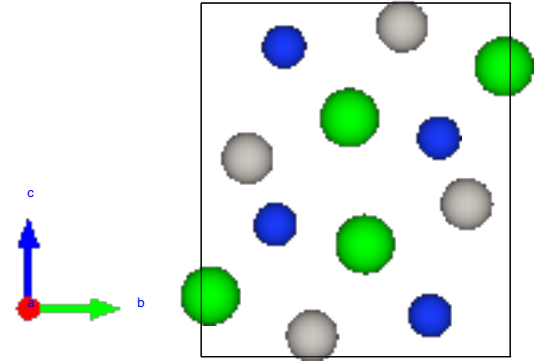

Nanowire Transmission:

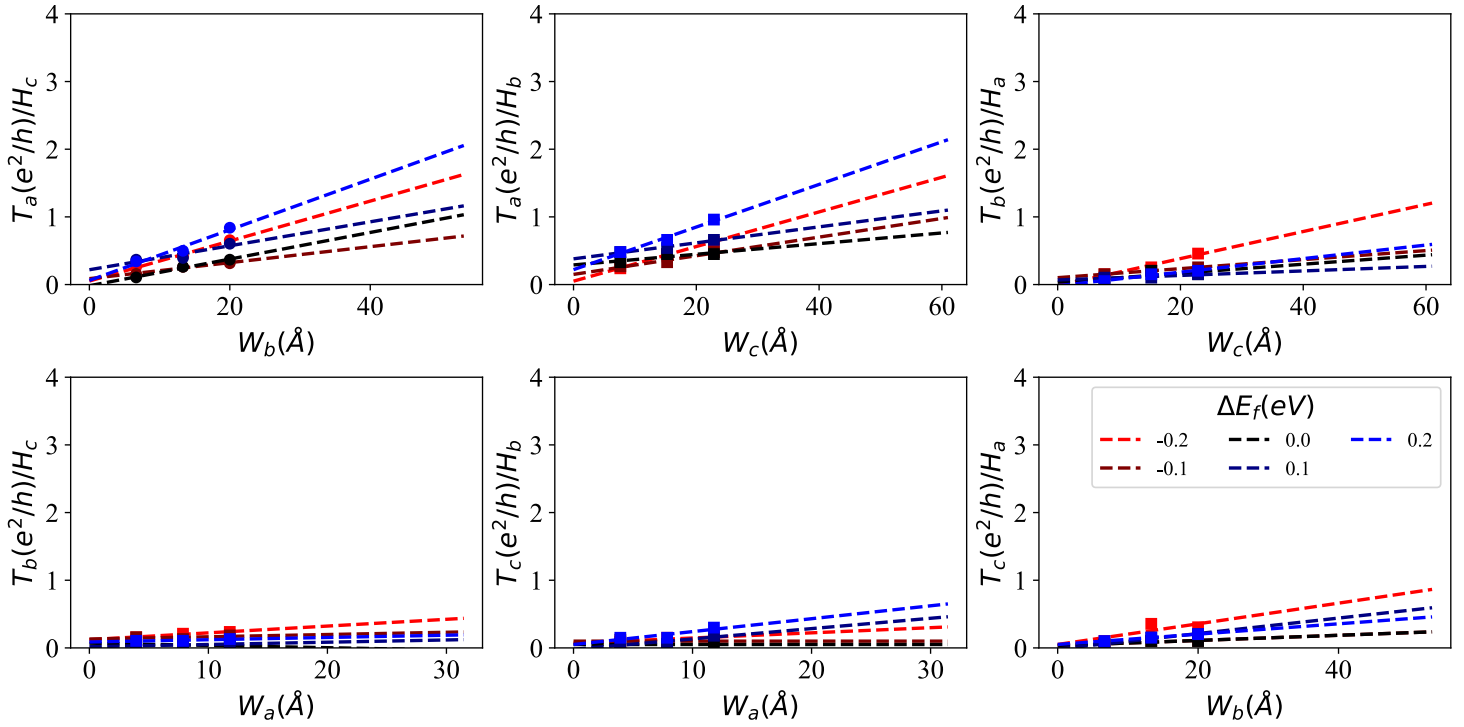

Compound: ZrSiS  
Materials Project ID: 3938

Lattice (conventional cell):

| Parameter        | Value   | Unit |
|------------------|---------|------|
| a                | 3.6168  | Å    |
| b                | 3.6168  | Å    |
| c                | 8.6761  | Å    |
| $\alpha$ (alpha) | 90.0000 | °    |
| $\beta$ (beta)   | 90.0000 | °    |
| $\gamma$ (gamma) | 90.0000 | °    |

Crystal structure (conventional cell):

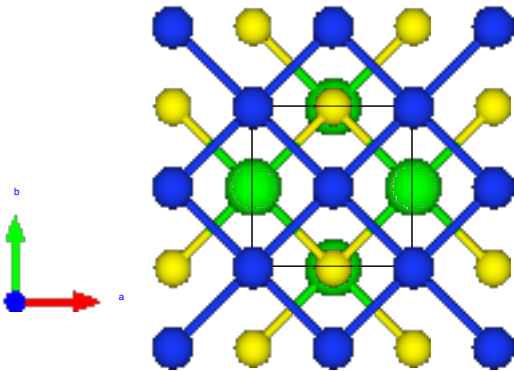

Nanowire Transmission:

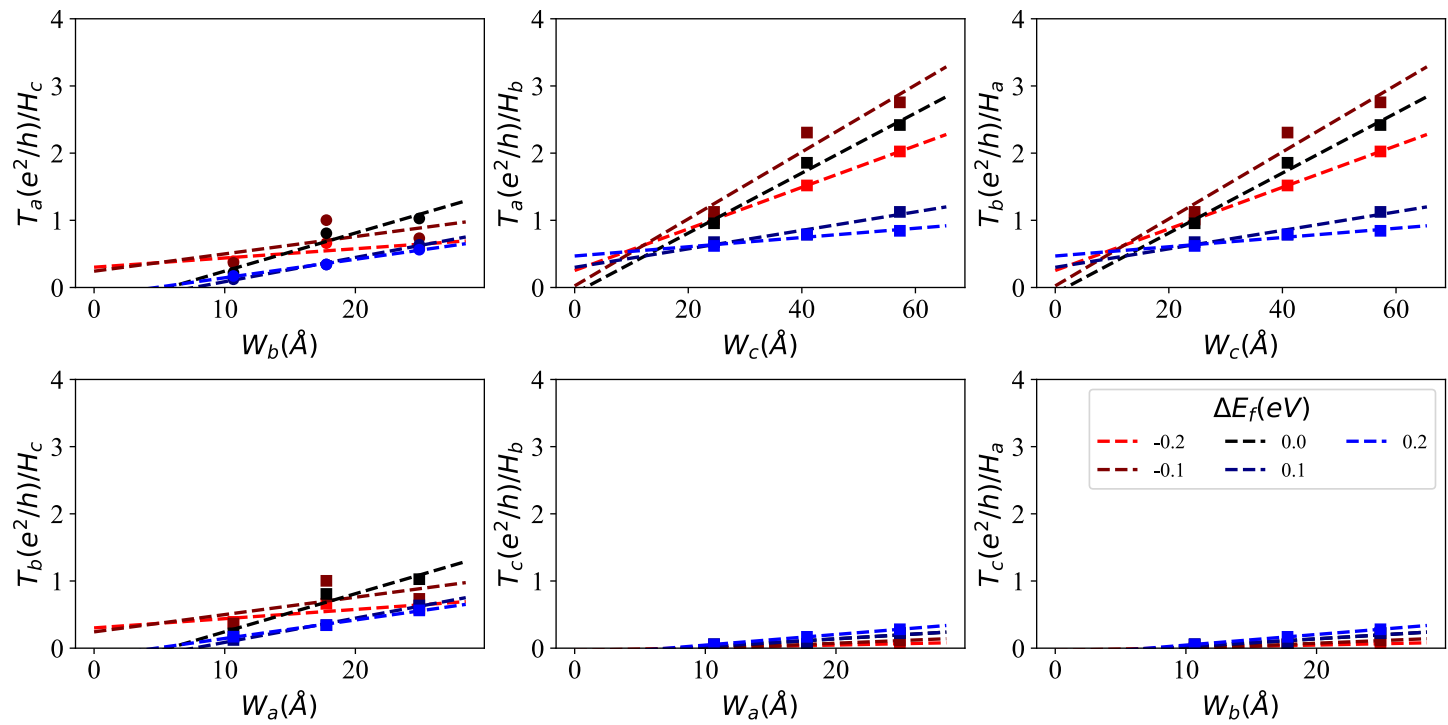

Compound: ZrSiSe  
Materials Project ID: 81

Lattice (conventional cell):

| Parameter        | Value   | Unit |
|------------------|---------|------|
| a                | 3.6168  | Å    |
| b                | 3.6168  | Å    |
| c                | 8.6761  | Å    |
| $\alpha$ (alpha) | 90.0000 | °    |
| $\beta$ (beta)   | 90.0000 | °    |
| $\gamma$ (gamma) | 90.0000 | °    |

Crystal structure (conventional cell):

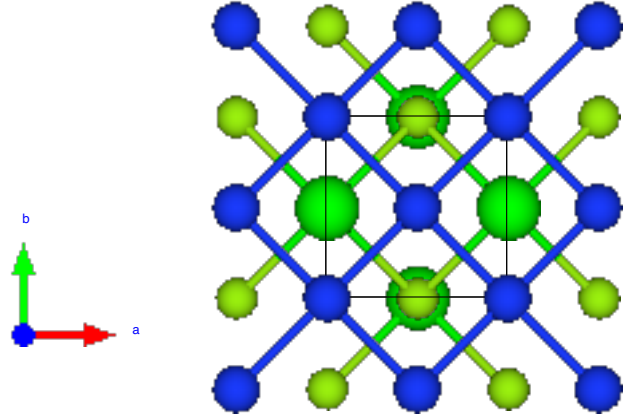

Nanowire Transmission:

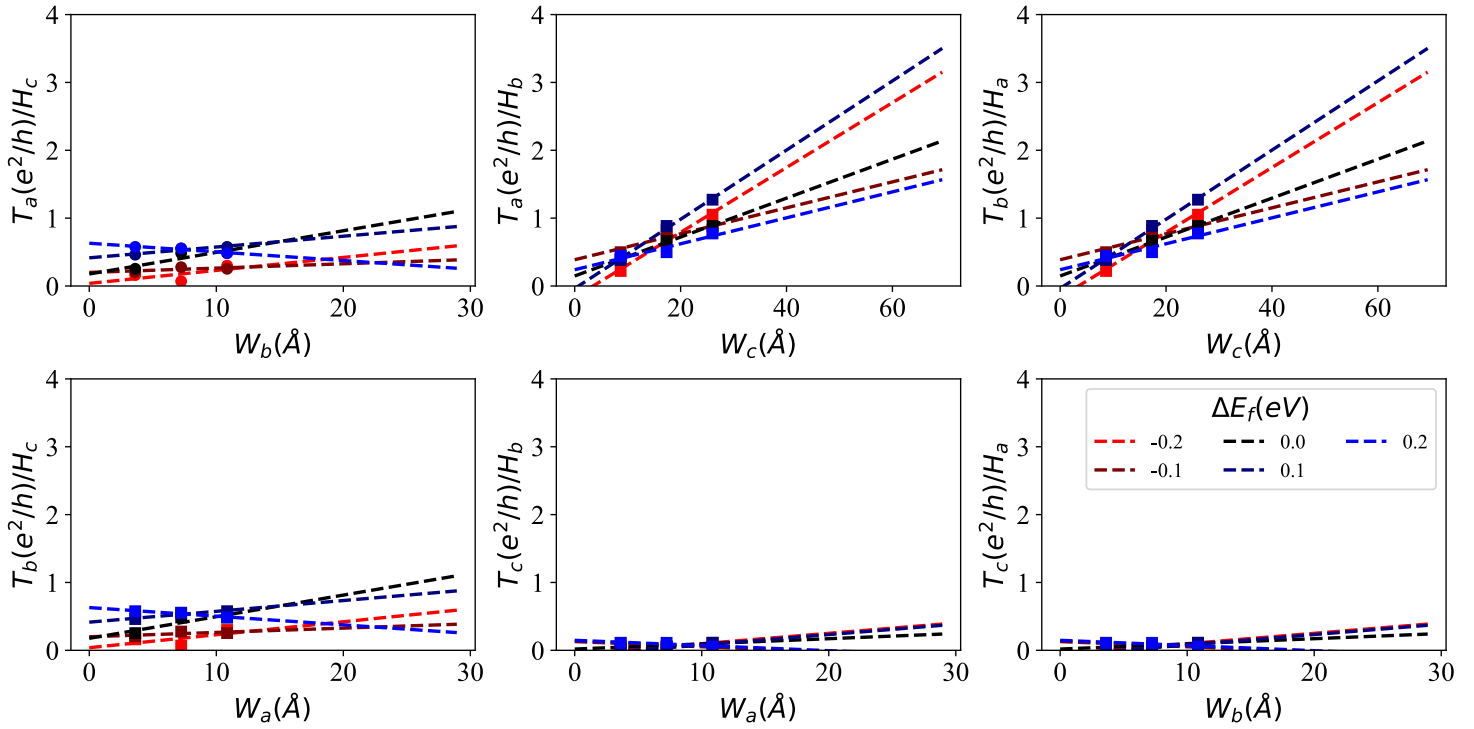

Compound: ZrTe  
Materials Project ID: 1539

Lattice (conventional cell):

| Parameter        | Value    | Unit |
|------------------|----------|------|
| a                | 3.7994   | Å    |
| b                | 3.7994   | Å    |
| c                | 3.8986   | Å    |
| $\alpha$ (alpha) | 90.0000  | °    |
| $\beta$ (beta)   | 90.0000  | °    |
| $\gamma$ (gamma) | 120.0000 | °    |

Crystal structure (conventional cell):

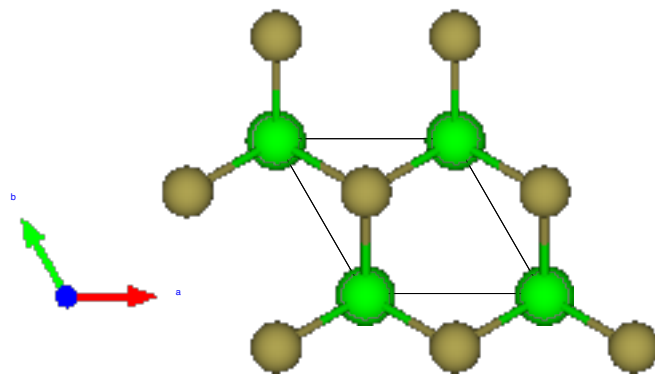

Nanowire Transmission:

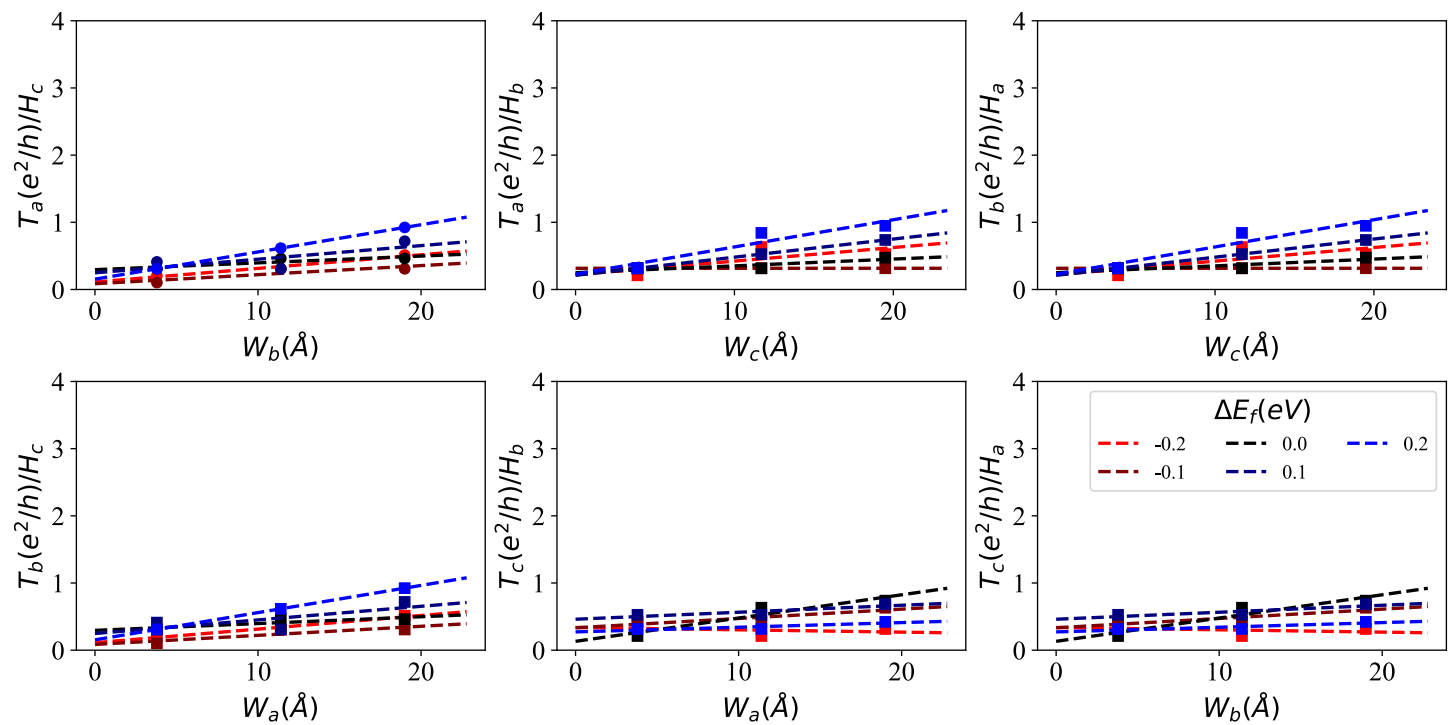

Supplement: Supplementary file 2 [file TSM_SM_Transmission.pdf]
